# Supplementary material for: Validating First-Principles Phonon Lifetimes via Inelastic Neutron Scattering
Source: arXiv:2202.11041 source file (2022-02-22)
Supplement: Supplementary file 2 [file supplemental2_BOpot.pdf]

The third order contribution to Born-Oppenheimer potential of  $\text{CaF}_2$  with  $\hat{\mathbf{S}}_{BZ} = \hat{\mathbf{S}}_O$ :

[illegible]

[illegible]

[illegible]

[illegible]

$$\begin{aligned}
& + d_{\Gamma}^{T_{2g}{}^2A_1{}^2B_1}(-u_{\Gamma}^{T_{2g}{}^{(1)}}u_A^{2A_1}u_{\bar{A}}^{2B_1} + u_{\Gamma}^{T_{2g}{}^{(2)}}u_A^{2A_1}u_{\bar{A}}^{2B_1} + u_{\Gamma}^{T_{2g}{}^{(1)}}u_A^{2B_1}u_{\bar{A}}^{2A_1} - u_{\Gamma}^{T_{2g}{}^{(2)}}u_A^{2B_1}u_{\bar{A}}^{2A_1} + u_{\Gamma}^{T_{2g}{}^{(0)}}u_{A_2}^{2A_1}u_{\bar{A}_2}^{2B_1} \\
& \quad - u_{\Gamma}^{T_{2g}{}^{(1)}}u_{A_2}^{2A_1}u_{\bar{A}_2}^{2B_1} - u_{\Gamma}^{T_{2g}{}^{(0)}}u_{A_2}^{2B_1}u_{\bar{A}_2}^{2A_1} + u_{\Gamma}^{T_{2g}{}^{(1)}}u_{A_2}^{2B_1}u_{\bar{A}_2}^{2A_1} - u_{\Gamma}^{T_{2g}{}^{(0)}}u_{\bar{A}_1}^{2B_1}u_{A_1}^{2A_1} - u_{\Gamma}^{T_{2g}{}^{(2)}}u_{\bar{A}_1}^{2B_1}u_{A_1}^{2A_1} \\
& \quad + u_{\Gamma}^{T_{2g}{}^{(0)}}u_{\bar{A}_1}^{2A_1}u_{A_1}^{2B_1} + u_{\Gamma}^{T_{2g}{}^{(2)}}u_{\bar{A}_1}^{2A_1}u_{A_1}^{2B_1} - u_{\Gamma}^{T_{2g}{}^{(0)}}u_{\bar{A}_4}^{2B_1}u_{A_4}^{2A_1} - u_{\Gamma}^{T_{2g}{}^{(1)}}u_{\bar{A}_4}^{2B_1}u_{A_4}^{2A_1} + u_{\Gamma}^{T_{2g}{}^{(0)}}u_{\bar{A}_4}^{2A_1}u_{A_4}^{2B_1} \\
& \quad + u_{\Gamma}^{T_{2g}{}^{(1)}}u_{\bar{A}_4}^{2A_1}u_{A_4}^{2B_1} + u_{\Gamma}^{T_{2g}{}^{(0)}}u_{\bar{A}_3}^{2A_1}u_{A_3}^{2B_1} - u_{\Gamma}^{T_{2g}{}^{(2)}}u_{\bar{A}_3}^{2A_1}u_{A_3}^{2B_1} - u_{\Gamma}^{T_{2g}{}^{(0)}}u_{\bar{A}_3}^{2B_1}u_{A_3}^{2A_1} + u_{\Gamma}^{T_{2g}{}^{(2)}}u_{\bar{A}_3}^{2B_1}u_{A_3}^{2A_1} \\
& \quad - u_{\Gamma}^{T_{2g}{}^{(1)}}u_{A_5}^{2B_1}u_{\bar{A}_5}^{2A_1} - u_{\Gamma}^{T_{2g}{}^{(2)}}u_{A_5}^{2B_1}u_{\bar{A}_5}^{2A_1} + u_{\Gamma}^{T_{2g}{}^{(1)}}u_{A_5}^{2A_1}u_{\bar{A}_5}^{2B_1} + u_{\Gamma}^{T_{2g}{}^{(2)}}u_{A_5}^{2A_1}u_{\bar{A}_5}^{2B_1}) \\
& + d_{\Gamma}^{T_{1u}{}^2A_1{}^2B_1}(u_{\Gamma}^{T_{1u}{}^{(2)}}u_A^{2A_1}u_{\bar{A}}^{2B_1} + u_{\Gamma}^{T_{1u}{}^{(2)}}u_A^{2B_1}u_{\bar{A}}^{2A_1} + u_{\Gamma}^{T_{1u}{}^{(1)}}u_{A_2}^{2A_1}u_{\bar{A}_2}^{2B_1} + u_{\Gamma}^{T_{1u}{}^{(1)}}u_{A_2}^{2B_1}u_{\bar{A}_2}^{2A_1} - u_{\Gamma}^{T_{1u}{}^{(0)}}u_{\bar{A}_1}^{2B_1}u_{A_1}^{2A_1} \\
& \quad - u_{\Gamma}^{T_{1u}{}^{(0)}}u_{\bar{A}_1}^{2A_1}u_{A_1}^{2B_1} - u_{\Gamma}^{T_{1u}{}^{(1)}}u_{\bar{A}_4}^{2B_1}u_{A_4}^{2A_1} - u_{\Gamma}^{T_{1u}{}^{(1)}}u_{\bar{A}_4}^{2A_1}u_{A_4}^{2B_1} + u_{\Gamma}^{T_{1u}{}^{(0)}}u_{\bar{A}_3}^{2A_1}u_{A_3}^{2B_1} + u_{\Gamma}^{T_{1u}{}^{(0)}}u_{\bar{A}_3}^{2B_1}u_{A_3}^{2A_1} \\
& \quad - u_{\Gamma}^{T_{1u}{}^{(2)}}u_{A_5}^{2B_1}u_{\bar{A}_5}^{2A_1} - u_{\Gamma}^{T_{1u}{}^{(2)}}u_{A_5}^{2A_1}u_{\bar{A}_5}^{2B_1}) \\
& + d_{\Gamma}^{T_{1u}{}^2A_1B_2}(u_{\Gamma}^{T_{1u}{}^{(0)}}u_A^{2A_1}u_{\bar{A}}^{B_2} + u_{\Gamma}^{T_{1u}{}^{(1)}}u_A^{2A_1}u_{\bar{A}}^{B_2} - u_{\Gamma}^{T_{1u}{}^{(0)}}u_A^{B_2}u_{\bar{A}}^{2A_1} - u_{\Gamma}^{T_{1u}{}^{(1)}}u_A^{B_2}u_{\bar{A}}^{2A_1} - u_{\Gamma}^{T_{1u}{}^{(0)}}u_{A_2}^{2A_1}u_{\bar{A}_2}^{B_2} \\
& \quad - u_{\Gamma}^{T_{1u}{}^{(2)}}u_{A_2}^{2A_1}u_{\bar{A}_2}^{B_2} + u_{\Gamma}^{T_{1u}{}^{(0)}}u_{A_2}^{B_2}u_{\bar{A}_2}^{2A_1} + u_{\Gamma}^{T_{1u}{}^{(2)}}u_{A_2}^{B_2}u_{\bar{A}_2}^{2A_1} + u_{\Gamma}^{T_{1u}{}^{(1)}}u_{\bar{A}_1}^{B_2}u_{A_1}^{2A_1} - u_{\Gamma}^{T_{1u}{}^{(2)}}u_{\bar{A}_1}^{B_2}u_{A_1}^{2A_1} \\
& \quad - u_{\Gamma}^{T_{1u}{}^{(1)}}u_{\bar{A}_1}^{2A_1}u_{A_1}^{B_2} + u_{\Gamma}^{T_{1u}{}^{(2)}}u_{\bar{A}_1}^{2A_1}u_{A_1}^{B_2} - u_{\Gamma}^{T_{1u}{}^{(0)}}u_{\bar{A}_4}^{B_2}u_{A_4}^{2A_1} + u_{\Gamma}^{T_{1u}{}^{(2)}}u_{\bar{A}_4}^{B_2}u_{A_4}^{2A_1} + u_{\Gamma}^{T_{1u}{}^{(0)}}u_{\bar{A}_4}^{2A_1}u_{A_4}^{B_2} \\
& \quad - u_{\Gamma}^{T_{1u}{}^{(2)}}u_{\bar{A}_4}^{2A_1}u_{A_4}^{B_2} + u_{\Gamma}^{T_{1u}{}^{(1)}}u_{\bar{A}_3}^{2A_1}u_{A_3}^{B_2} + u_{\Gamma}^{T_{1u}{}^{(2)}}u_{\bar{A}_3}^{2A_1}u_{A_3}^{B_2} - u_{\Gamma}^{T_{1u}{}^{(1)}}u_{\bar{A}_3}^{B_2}u_{A_3}^{2A_1} - u_{\Gamma}^{T_{1u}{}^{(2)}}u_{\bar{A}_3}^{B_2}u_{A_3}^{2A_1} \\
& \quad + u_{\Gamma}^{T_{1u}{}^{(0)}}u_{A_5}^{B_2}u_{\bar{A}_5}^{2A_1} - u_{\Gamma}^{T_{1u}{}^{(1)}}u_{A_5}^{B_2}u_{\bar{A}_5}^{2A_1} - u_{\Gamma}^{T_{1u}{}^{(0)}}u_{A_5}^{2A_1}u_{\bar{A}_5}^{B_2} + u_{\Gamma}^{T_{1u}{}^{(1)}}u_{A_5}^{2A_1}u_{\bar{A}_5}^{B_2}) \\
& + d_{\Gamma}^{T_{1u}{}^2A_1{}^1B_2}(u_{\Gamma}^{T_{1u}{}^{(0)}}u_A^{2A_1}u_{\bar{A}}^{1B_2} + u_{\Gamma}^{T_{1u}{}^{(1)}}u_A^{2A_1}u_{\bar{A}}^{1B_2} - u_{\Gamma}^{T_{1u}{}^{(0)}}u_A^{1B_2}u_{\bar{A}}^{2A_1} - u_{\Gamma}^{T_{1u}{}^{(1)}}u_A^{1B_2}u_{\bar{A}}^{2A_1} - u_{\Gamma}^{T_{1u}{}^{(0)}}u_{A_2}^{2A_1}u_{\bar{A}_2}^{1B_2} \\
& \quad - u_{\Gamma}^{T_{1u}{}^{(2)}}u_{A_2}^{2A_1}u_{\bar{A}_2}^{1B_2} + u_{\Gamma}^{T_{1u}{}^{(0)}}u_{A_2}^{1B_2}u_{\bar{A}_2}^{2A_1} + u_{\Gamma}^{T_{1u}{}^{(2)}}u_{A_2}^{1B_2}u_{\bar{A}_2}^{2A_1} + u_{\Gamma}^{T_{1u}{}^{(1)}}u_{\bar{A}_1}^{1B_2}u_{A_1}^{2A_1} - u_{\Gamma}^{T_{1u}{}^{(2)}}u_{\bar{A}_1}^{1B_2}u_{A_1}^{2A_1} \\
& \quad - u_{\Gamma}^{T_{1u}{}^{(1)}}u_{\bar{A}_1}^{2A_1}u_{A_1}^{1B_2} + u_{\Gamma}^{T_{1u}{}^{(2)}}u_{\bar{A}_1}^{2A_1}u_{A_1}^{1B_2} - u_{\Gamma}^{T_{1u}{}^{(0)}}u_{\bar{A}_4}^{1B_2}u_{A_4}^{2A_1} + u_{\Gamma}^{T_{1u}{}^{(2)}}u_{\bar{A}_4}^{1B_2}u_{A_4}^{2A_1} + u_{\Gamma}^{T_{1u}{}^{(0)}}u_{\bar{A}_4}^{2A_1}u_{A_4}^{1B_2} \\
& \quad - u_{\Gamma}^{T_{1u}{}^{(2)}}u_{\bar{A}_4}^{2A_1}u_{A_4}^{1B_2} + u_{\Gamma}^{T_{1u}{}^{(1)}}u_{\bar{A}_3}^{2A_1}u_{A_3}^{1B_2} + u_{\Gamma}^{T_{1u}{}^{(2)}}u_{\bar{A}_3}^{2A_1}u_{A_3}^{1B_2} - u_{\Gamma}^{T_{1u}{}^{(1)}}u_{\bar{A}_3}^{1B_2}u_{A_3}^{2A_1} - u_{\Gamma}^{T_{1u}{}^{(2)}}u_{\bar{A}_3}^{1B_2}u_{A_3}^{2A_1} \\
& \quad + u_{\Gamma}^{T_{1u}{}^{(0)}}u_{A_5}^{1B_2}u_{\bar{A}_5}^{2A_1} - u_{\Gamma}^{T_{1u}{}^{(1)}}u_{A_5}^{1B_2}u_{\bar{A}_5}^{2A_1} - u_{\Gamma}^{T_{1u}{}^{(0)}}u_{A_5}^{2A_1}u_{\bar{A}_5}^{1B_2} + u_{\Gamma}^{T_{1u}{}^{(1)}}u_{A_5}^{2A_1}u_{\bar{A}_5}^{1B_2}) \\
& + d_{\Gamma}^{T_{2g}{}^A_2A_2}(u_{\Gamma}^{T_{2g}{}^{(0)}}u_A^{A_2}u_{\bar{A}}^{A_2} + u_{\Gamma}^{T_{2g}{}^{(2)}}u_{A_2}^{A_2}u_{\bar{A}_2}^{A_2} - u_{\Gamma}^{T_{2g}{}^{(1)}}u_{\bar{A}_1}^{A_2}u_{A_1}^{A_2} - u_{\Gamma}^{T_{2g}{}^{(2)}}u_{\bar{A}_4}^{A_2}u_{A_4}^{A_2} + u_{\Gamma}^{T_{2g}{}^{(1)}}u_{\bar{A}_3}^{A_2}u_{A_3}^{A_2} \\
& \quad - u_{\Gamma}^{T_{2g}{}^{(0)}}u_{A_5}^{A_2}u_{\bar{A}_5}^{A_2}) \\
& + d_{\Gamma}^{T_{1u}{}^A_2B_1}(u_{$$

$$\begin{aligned}
& + u_{\Gamma^{1u}}^{(0)} u_{A_5}^{2B_1} u_{\bar{A}_5}^{A_2} - u_{\Gamma^{1u}}^{(1)} u_{A_5}^{2B_1} u_{\bar{A}_5}^{A_2} - u_{\Gamma^{1u}}^{(0)} u_{A_5}^{A_2} u_{\bar{A}_5}^{2B_1} + u_{\Gamma^{1u}}^{(1)} u_{A_5}^{A_2} u_{\bar{A}_5}^{2B_1} \\
& + d_{\Gamma}^{T_{2g} A_2 B_2} (-u_{\Gamma}^{T_{2g} (1)} u_A^{A_2} u_{\bar{A}}^{B_2} + u_{\Gamma}^{T_{2g} (2)} u_A^{A_2} u_{\bar{A}}^{B_2} + u_{\Gamma}^{T_{2g} (1)} u_A^{B_2} u_{\bar{A}}^{A_2} - u_{\Gamma}^{T_{2g} (2)} u_A^{B_2} u_{\bar{A}}^{A_2} + u_{\Gamma}^{T_{2g} (0)} u_{A_2}^{A_2} u_{A_2}^{B_2} \\
& - u_{\Gamma}^{T_{2g} (1)} u_{A_2}^{A_2} u_{\bar{A}_2}^{B_2} - u_{\Gamma}^{T_{2g} (0)} u_{A_2}^{B_2} u_{\bar{A}_2}^{A_2} + u_{\Gamma}^{T_{2g} (1)} u_{A_2}^{B_2} u_{\bar{A}_2}^{A_2} - u_{\Gamma}^{T_{2g} (0)} u_{\bar{A}_1}^{B_2} u_{A_1}^{A_2} - u_{\Gamma}^{T_{2g} (2)} u_{\bar{A}_1}^{B_2} u_{A_1}^{A_2} \\
& + u_{\Gamma}^{T_{2g} (0)} u_{\bar{A}_1}^{A_2} u_{A_1}^{B_2} + u_{\Gamma}^{T_{2g} (2)} u_{\bar{A}_1}^{A_2} u_{A_1}^{B_2} - u_{\Gamma}^{T_{2g} (0)} u_{\bar{A}_4}^{B_2} u_{A_4}^{A_2} - u_{\Gamma}^{T_{2g} (1)} u_{\bar{A}_4}^{B_2} u_{A_4}^{A_2} + u_{\Gamma}^{T_{2g} (0)} u_{\bar{A}_4}^{A_2} u_{A_4}^{B_2} \\
& + u_{\Gamma}^{T_{2g} (1)} u_{\bar{A}_4}^{A_2} u_{A_4}^{B_2} + u_{\Gamma}^{T_{2g} (0)} u_{\bar{A}_3}^{A_2} u_{A_3}^{B_2} - u_{\Gamma}^{T_{2g} (2)} u_{\bar{A}_3}^{A_2} u_{A_3}^{B_2} - u_{\Gamma}^{T_{2g} (0)} u_{\bar{A}_3}^{B_2} u_{A_3}^{A_2} + u_{\Gamma}^{T_{2g} (2)} u_{\bar{A}_3}^{B_2} u_{A_3}^{A_2} \\
& - u_{\Gamma}^{T_{2g} (1)} u_{A_5}^{B_2} u_{\bar{A}_5}^{A_2} - u_{\Gamma}^{T_{2g} (2)} u_{A_5}^{B_2} u_{\bar{A}_5}^{A_2} + u_{\Gamma}^{T_{2g} (1)} u_{A_5}^{A_2} u_{\bar{A}_5}^{B_2} + u_{\Gamma}^{T_{2g} (2)} u_{A_5}^{A_2} u_{\bar{A}_5}^{B_2}) \\
& + d_{\Gamma}^{T_{1u} A_2 B_2} (u_{\Gamma^{1u}}^{(2)} u_A^{A_2} u_{\bar{A}}^{B_2} + u_{\Gamma^{1u}}^{(2)} u_A^{B_2} u_{\bar{A}}^{A_2} + u_{\Gamma^{1u}}^{(1)} u_{A_2}^{A_2} u_{\bar{A}_2}^{B_2} + u_{\Gamma^{1u}}^{(1)} u_{A_2}^{B_2} u_{\bar{A}_2}^{A_2} - u_{\Gamma^{1u}}^{(0)} u_{\bar{A}_1}^{B_2} u_{A_1}^{A_2} \\
& - u_{\Gamma^{1u}}^{(0)} u_{\bar{A}_1}^{A_2} u_{A_1}^{B_2} - u_{\Gamma^{1u}}^{(1)} u_{\bar{A}_4}^{B_2} u_{A_4}^{A_2} - u_{\Gamma^{1u}}^{(1)} u_{\bar{A}_4}^{A_2} u_{A_4}^{B_2} + u_{\Gamma^{1u}}^{(0)} u_{\bar{A}_3}^{A_2} u_{A_3}^{B_2} + u_{\Gamma^{1u}}^{(0)} u_{\bar{A}_3}^{B_2} u_{A_3}^{A_2} \\
& - u_{\Gamma^{1u}}^{(2)} u_{A_5}^{B_2} u_{\bar{A}_5}^{A_2} - u_{\Gamma^{1u}}^{(2)} u_{A_5}^{A_2} u_{\bar{A}_5}^{B_2}) \\
& + d_{\Gamma}^{T_{2g} A_2 {}^1B_2} (-u_{\Gamma}^{T_{2g} (1)} u_A^{A_2} u_{\bar{A}}^{1B_2} + u_{\Gamma}^{T_{2g} (2)} u_A^{A_2} u_{\bar{A}}^{1B_2} + u_{\Gamma}^{T_{2g} (1)} u_A^{1B_2} u_{\bar{A}}^{A_2} - u_{\Gamma}^{T_{2g} (2)} u_A^{1B_2} u_{\bar{A}}^{A_2} + u_{\Gamma}^{T_{2g} (0)} u_{A_2}^{A_2} u_{A_2}^{1B_2} \\
& - u_{\Gamma}^{T_{2g} (1)} u_{A_2}^{A_2} u_{\bar{A}_2}^{1B_2} - u_{\Gamma}^{T_{2g} (0)} u_{A_2}^{1B_2} u_{\bar{A}_2}^{A_2} + u_{\Gamma}^{T_{2g} (1)} u_{A_2}^{1B_2} u_{\bar{A}_2}^{A_2} - u_{\Gamma}^{T_{2g} (0)} u_{\bar{A}_1}^{1B_2} u_{A_1}^{A_2} - u_{\Gamma}^{T_{2g} (2)} u_{\bar{A}_1}^{1B_2} u_{A_1}^{A_2} \\
& + u_{\Gamma}^{T_{2g} (0)} u_{\bar{A}_1}^{A_2} u_{A_1}^{1B_2} + u_{\Gamma}^{T_{2g} (2)} u_{\bar{A}_1}^{A_2} u_{A_1}^{1B_2} - u_{\Gamma}^{T_{2g} (0)} u_{\bar{A}_4}^{1B_2} u_{A_4}^{A_2} - u_{\Gamma}^{T_{2g} (1)} u_{\bar{A}_4}^{1B_2} u_{A_4}^{A_2} + u_{\Gamma}^{T_{2g} (0)} u_{\bar{A}_4}^{A_2} u_{A_4}^{1B_2} \\
& + u_{\Gamma}^{T_{2g} (1)} u_{\bar{A}_4}^{A_2} u_{A_4}^{1B_2} + u_{\Gamma}^{T_{2g} (0)} u_{\bar{A}_3}^{A_2} u_{A_3}^{1B_2} - u_{\Gamma}^{T_{2g} (2)} u_{\bar{A}_3}^{A_2} u_{A_3}^{1B_2} - u_{\Gamma}^{T_{2g} (0)} u_{\bar{A}_3}^{1B_2} u_{A_3}^{A_2} + u_{\Gamma}^{T_{2g} (2)} u_{\bar{A}_3}^{1B_2} u_{A_3}^{A_2} \\
& - u_{\Gamma}^{T_{2g} (1)} u_{A_5}^{1B_2} u_{\bar{A}_5}^{A_2} - u_{\Gamma}^{T_{2g} (2)} u_{A_5}^{1B_2} u_{\bar{A}_5}^{A_2} + u_{\Gamma}^{T_{2g} (1)} u_{A_5}^{A_2} u_{\bar{A}_5}^{1B_2} + u_{\Gamma}^{T_{2g} (2)} u_{A_5}^{A_2} u_{\bar{A}_5}^{1B_2}) \\
& + d_{\Gamma}^{T_{1u} A_2 {}^1B_2} (u_{\Gamma^{1u}}^{(2)} u_A^{A_2} u_{\bar{A}}^{1B_2} + u_{\Gamma^{1u}}^{(2)} u_A^{1B_2} u_{\bar{A}}^{A_2} + u_{\Gamma^{1u}}^{(1)} u_{A_2}^{A_2} u_{\bar{A}_2}^{1B_2} + u_{\Gamma^{1u}}^{(1)} u_{A_2}^{1B_2} u_{\bar{A}_2}^{A_2} - u_{\Gamma^{1u}}^{(0)} u_{\bar{A}_1}^{1B_2} u_{A_1}^{A_2} \\
& - u_{\Gamma^{1u}}^{(0)} u_{\bar{A}_1}^{A_2} u_{A_1}^{1B_2} - u_{\Gamma^{1u}}^{(1)} u_{\bar{A}_4}^{1B_2} u_{A_4}^{A_2} - u_{\Gamma^{1u}}^{(1)} u_{\bar{A}_4}^{A_2} u_{A_4}^{1B_2} + u_{\Gamma^{1u}}^{(0)} u_{\bar{A}_3}^{A_2} u_{A_3}^{1B_2} + u_{\Gamma^{1u}}^{(0)} u_{\bar{A}_3}^{1B_2} u_{A_3}^{A_2} \\
& - u_{\Gamma^{1u}}^{(2)} u_{A_5}^{1B_2} u_{\bar{A}_5}^{A_2} - u_{\Gamma^{1u}}^{(2)} u_{A_5}^{A_2} u_{\bar{A}_5}^{1B_2}) \\
& + d_{\Gamma}^{T_{2g} B_1 {}^1B_1} (u_{\Gamma}^{T_{2g} (0)} u_A^{B_1} u_{\bar{A}}^{1B_1} + u_{\Gamma}^{T_{2g} (2)} u_A^{B_1} u_{\bar{A}}^{1B_1} - u_{\Gamma}^{T_{2g} (1)} u_{\bar{A}_1}^{B_1} u_{A_1}^{B_1} - u_{\Gamma}^{T_{2g} (2)} u_{\bar{A}_4}^{B_1} u_{A_4}^{B_1} + u_{\Gamma}^{T_{2g} (1)} u_{\bar{A}_3}^{B_1} u_{A_3}^{B_1} \\
& - u_{\Gamma}^{T_{2g} (0)} u_{A_5}^{B_1} u_{\bar{A}_5}^{1B_1}) \\
& + d_{\Gamma}^{T_{2g} B_1 {}^1B_1} (u_{\Gamma}^{T_{2g} (0)} u_A^{B_1} u_{\bar{A}}^{1B_1} + u_{\Gamma}^{T_{2g} (0)} u_A^{1B_1} u_{\bar{A}}^{B_1} + u_{\Gamma}^{T_{2g} (2)} u_{A_2}^{B_1} u_{\bar{A}_2}^{1B_1} + u_{\Gamma}^{T_{2g} (2)} u_{A_2}^{1B_1} u_{\bar{A}_2}^{B_1} - u_{\Gamma}^{T_{2g} (1)} u_{\bar{A}_1}^{1B_1} u_{A_1}^{B_1} \\
& - u_{\Gamma}^{T_{2g} (1)} u_{\bar{A}_1}^{B_1} u_{A_1}^{1B_1} - u_{\Gamma}^{T_{2g} (2)} u_{\bar{A}_4}^{1B_1} u_{A_4}^{B_1} - u_{\Gamma}^{T_{2g} (2)} u_{\bar{A}_4}^{B_1} u_{A_4}^{1B_1} + u_{\Gamma}^{T_{2g} (1)} u_{\bar{A}_3}^{B_1} u_{A_3}^{1B_1} + u_{\Gamma}^{T_{2g} (1)} u_{\bar{A}_3}^{1B_1} u_{A_3}^{B_1} \\
& - u_{\Gamma}^{T_{2g} (0)} u_{A_5}^{1B_1} u_{\bar{A}_5}^{B_1} - u_{\Gamma}^{T_{2g} (0)} u_{A_5}^{B_1} u_{\bar{A}_5}^{1B_1}) \\
& + d_{\Gamma}^{T_{1u} B_1 {}^1B_1} (u_{\Gamma^{1u}}^{(0)} u_A^{B_1} u_{\bar{A}}^{1B_1} - u_{\Gamma^{1u}}^{(1)} u_A^{B_1} u_{\bar{A}}^{1B_1} - u_{\Gamma^{1u}}^{(0)} u_A^{1B_1} u_{\bar{A}}^{B_1} + u_{\Gamma^{1u}}^{(1)} u_A^{1B_1} u_{\bar{A}}^{B_1} + u_{\Gamma^{1u}}^{(0)} u_{A_2}^{B_1} u_{A_2}^{1B_1} \\
& - u_{\Gamma^{1u}}^{(2)} u_{A$$

$$\begin{aligned}
& -u_{\Gamma}^{T_{1u}^{(2)}} u_{\bar{A}_4}^{B_1} u_{A_4}^{2B_1} + u_{\Gamma}^{T_{1u}^{(1)}} u_{\bar{A}_3}^{B_1} u_{A_3}^{2B_1} - u_{\Gamma}^{T_{1u}^{(2)}} u_{\bar{A}_3}^{B_1} u_{A_3}^{2B_1} - u_{\Gamma}^{T_{1u}^{(1)}} u_{\bar{A}_3}^{2B_1} u_{A_3}^{B_1} + u_{\Gamma}^{T_{1u}^{(2)}} u_{\bar{A}_3}^{2B_1} u_{A_3}^{B_1} \\
& + u_{\Gamma}^{T_{1u}^{(0)}} u_{A_5}^{2B_1} u_{\bar{A}_5}^{B_1} + u_{\Gamma}^{T_{1u}^{(1)}} u_{A_5}^{2B_1} u_{\bar{A}_5}^{B_1} - u_{\Gamma}^{T_{1u}^{(0)}} u_{A_5}^{B_1} u_{\bar{A}_5}^{2B_1} - u_{\Gamma}^{T_{1u}^{(1)}} u_{A_5}^{B_1} u_{\bar{A}_5}^{2B_1}) \\
& + d_{\Gamma}^{T_{2g} B_1 B_2} (-u_{\Gamma}^{T_{2g}^{(1)}} u_A^{B_1} u_{\bar{A}}^{B_2} - u_{\Gamma}^{T_{2g}^{(2)}} u_A^{B_1} u_{\bar{A}}^{B_2} + u_{\Gamma}^{T_{2g}^{(1)}} u_A^{B_2} u_{\bar{A}}^{B_1} + u_{\Gamma}^{T_{2g}^{(2)}} u_A^{B_2} u_{\bar{A}}^{B_1} + u_{\Gamma}^{T_{2g}^{(0)}} u_A^{B_1} u_{\bar{A}_2}^{B_2} \\
& + u_{\Gamma}^{T_{2g}^{(1)}} u_{A_2}^{B_1} u_{\bar{A}_2}^{B_2} - u_{\Gamma}^{T_{2g}^{(0)}} u_{A_2}^{B_2} u_{\bar{A}_2}^{B_1} - u_{\Gamma}^{T_{2g}^{(1)}} u_{A_2}^{B_2} u_{\bar{A}_2}^{B_1} + u_{\Gamma}^{T_{2g}^{(0)}} u_{A_1}^{B_2} u_{A_1}^{B_1} - u_{\Gamma}^{T_{2g}^{(2)}} u_{A_1}^{B_2} u_{A_1}^{B_1} \\
& - u_{\Gamma}^{T_{2g}^{(0)}} u_{\bar{A}_1}^{B_1} u_{A_1}^{B_2} + u_{\Gamma}^{T_{2g}^{(2)}} u_{\bar{A}_1}^{B_1} u_{A_1}^{B_2} - u_{\Gamma}^{T_{2g}^{(0)}} u_{\bar{A}_4}^{B_2} u_{A_4}^{B_1} + u_{\Gamma}^{T_{2g}^{(1)}} u_{\bar{A}_4}^{B_2} u_{A_4}^{B_1} + u_{\Gamma}^{T_{2g}^{(0)}} u_{\bar{A}_4}^{B_1} u_{A_4}^{B_2} \\
& - u_{\Gamma}^{T_{2g}^{(1)}} u_{\bar{A}_4}^{B_1} u_{A_4}^{B_2} - u_{\Gamma}^{T_{2g}^{(0)}} u_{\bar{A}_3}^{B_1} u_{A_3}^{B_2} - u_{\Gamma}^{T_{2g}^{(2)}} u_{\bar{A}_3}^{B_1} u_{A_3}^{B_2} + u_{\Gamma}^{T_{2g}^{(0)}} u_{\bar{A}_3}^{B_2} u_{A_3}^{B_1} + u_{\Gamma}^{T_{2g}^{(2)}} u_{\bar{A}_3}^{B_2} u_{A_3}^{B_1} \\
& - u_{\Gamma}^{T_{2g}^{(1)}} u_{A_5}^{B_2} u_{\bar{A}_5}^{B_1} + u_{\Gamma}^{T_{2g}^{(2)}} u_{A_5}^{B_2} u_{\bar{A}_5}^{B_1} + u_{\Gamma}^{T_{2g}^{(1)}} u_{A_5}^{B_1} u_{\bar{A}_5}^{B_2} - u_{\Gamma}^{T_{2g}^{(2)}} u_{A_5}^{B_1} u_{\bar{A}_5}^{B_2}) \\
& + d_{\Gamma}^{T_{2g} B_1 \bar{B}_2} (-u_{\Gamma}^{T_{2g}^{(1)}} u_A^{B_1} u_{\bar{A}}^{\bar{B}_2} - u_{\Gamma}^{T_{2g}^{(2)}} u_A^{B_1} u_{\bar{A}}^{\bar{B}_2} + u_{\Gamma}^{T_{2g}^{(1)}} u_A^{\bar{B}_2} u_{\bar{A}}^{B_1} + u_{\Gamma}^{T_{2g}^{(2)}} u_A^{\bar{B}_2} u_{\bar{A}}^{B_1} + u_{\Gamma}^{T_{2g}^{(0)}} u_{A_2}^{B_1} u_{\bar{A}_2}^{\bar{B}_2} \\
& + u_{\Gamma}^{T_{2g}^{(1)}} u_{A_2}^{B_1} u_{\bar{A}_2}^{\bar{B}_2} - u_{\Gamma}^{T_{2g}^{(0)}} u_{A_2}^{\bar{B}_2} u_{\bar{A}_2}^{B_1} - u_{\Gamma}^{T_{2g}^{(1)}} u_{A_2}^{\bar{B}_2} u_{\bar{A}_2}^{B_1} + u_{\Gamma}^{T_{2g}^{(0)}} u_{\bar{A}_1}^{\bar{B}_2} u_{A_1}^{B_1} - u_{\Gamma}^{T_{2g}^{(2)}} u_{\bar{A}_1}^{\bar{B}_2} u_{A_1}^{B_1} \\
& - u_{\Gamma}^{T_{2g}^{(0)}} u_{\bar{A}_1}^{B_1} u_{A_1}^{\bar{B}_2} + u_{\Gamma}^{T_{2g}^{(2)}} u_{\bar{A}_1}^{B_1} u_{A_1}^{\bar{B}_2} - u_{\Gamma}^{T_{2g}^{(0)}} u_{\bar{A}_4}^{\bar{B}_2} u_{A_4}^{B_1} + u_{\Gamma}^{T_{2g}^{(1)}} u_{\bar{A}_4}^{\bar{B}_2} u_{A_4}^{B_1} + u_{\Gamma}^{T_{2g}^{(0)}} u_{\bar{A}_4}^{B_1} u_{A_4}^{\bar{B}_2} \\
& - u_{\Gamma}^{T_{2g}^{(1)}} u_{\bar{A}_4}^{B_1} u_{A_4}^{\bar{B}_2} - u_{\Gamma}^{T_{2g}^{(0)}} u_{\bar{A}_3}^{B_1} u_{A_3}^{\bar{B}_2} - u_{\Gamma}^{T_{2g}^{(2)}} u_{\bar{A}_3}^{B_1} u_{A_3}^{\bar{B}_2} + u_{\Gamma}^{T_{2g}^{(0)}} u_{\bar{A}_3}^{\bar{B}_2} u_{A_3}^{B_1} + u_{\Gamma}^{T_{2g}^{(2)}} u_{\bar{A}_3}^{\bar{B}_2} u_{A_3}^{B_1} \\
& - u_{\Gamma}^{T_{2g}^{(1)}} u_{A_5}^{\bar{B}_2} u_{\bar{A}_5}^{B_1} + u_{\Gamma}^{T_{2g}^{(2)}} u_{A_5}^{\bar{B}_2} u_{\bar{A}_5}^{B_1} + u_{\Gamma}^{T_{2g}^{(1)}} u_{A_5}^{B_1} u_{\bar{A}_5}^{\bar{B}_2} - u_{\Gamma}^{T_{2g}^{(2)}} u_{A_5}^{B_1} u_{\bar{A}_5}^{\bar{B}_2}) \\
& + d_{\Gamma}^{T_{2g} \bar{B}_1 \bar{B}_2} (u_{\Gamma}^{T_{2g}^{(0)}} u_A^{\bar{B}_1} u_{\bar{A}}^{\bar{B}_2} + u_{\Gamma}^{T_{2g}^{(2)}} u_{A_2}^{\bar{B}_1} u_{\bar{A}_2}^{\bar{B}_2} - u_{\Gamma}^{T_{2g}^{(1)}} u_{\bar{A}_1}^{\bar{B}_1} u_{A_1}^{\bar{B}_2} - u_{\Gamma}^{T_{2g}^{(2)}} u_{\bar{A}_4}^{\bar{B}_1} u_{A_4}^{\bar{B}_2} + u_{\Gamma}^{T_{2g}^{(1)}} u_{\bar{A}_3}^{\bar{B}_1} u_{A_3}^{\bar{B}_2} \\
& - u_{\Gamma}^{T_{2g}^{(0)}} u_{A_5}^{\bar{B}_1} u_{\bar{A}_5}^{\bar{B}_2}) \\
& + d_{\Gamma}^{T_{2g} \bar{B}_1 \bar{B}_1} (u_{\Gamma}^{T_{2g}^{(0)}} u_A^{\bar{B}_1} u_{\bar{A}}^{2\bar{B}_1} + u_{\Gamma}^{T_{2g}^{(0)}} u_A^{2\bar{B}_1} u_{\bar{A}}^{\bar{B}_1} + u_{\Gamma}^{T_{2g}^{(2)}} u_{A_2}^{\bar{B}_1} u_{\bar{A}_2}^{2\bar{B}_1} + u_{\Gamma}^{T_{2g}^{(2)}} u_{A_2}^{2\bar{B}_1} u_{\bar{A}_2}^{\bar{B}_1} - u_{\Gamma}^{T_{2g}^{(1)}} u_{\bar{A}_1}^{2\bar{B}_1} u_{A_1}^{\bar{B}_1} \\
& - u_{\Gamma}^{T_{2g}^{(1)}} u_{\bar{A}_1}^{\bar{B}_1} u_{A_1}^{2\bar{B}_1} - u_{\Gamma}^{T_{2g}^{(2)}} u_{\bar{A}_4}^{2\bar{B}_1} u_{A_4}^{\bar{B}_1} - u_{\Gamma}^{T_{2g}^{(2)}} u_{\bar{A}_4}^{\bar{B}_1} u_{A_4}^{2\bar{B}_1} + u_{\Gamma}^{T_{2g}^{(1)}} u_{\bar{A}_3}^{\bar{B}_1} u_{A_3}^{2\bar{B}_1} + u_{\Gamma}^{T_{2g}^{(1)}} u_{\bar{A}_3}^{2\bar{B}_1} u_{A_3}^{\bar{B}_1} \\
& - u_{\Gamma}^{T_{2g}^{(0)}} u_{A_5}^{2\bar{B}_1} u_{\bar{A}_5}^{\bar{B}_1} - u_{\Gamma}^{T_{2g}^{(0)}} u_{A_5}^{\bar{B}_1} u_{\bar{A}_5}^{2\bar{B}_1}) \\
& + d_{\Gamma}^{T_{1u} \bar{B}_1 \bar{B}_1} (u_{\Gamma}^{T_{1u}^{(0)}} u_A^{\bar{B}_1} u_{\bar{A}}^{2\bar{B}_1} - u_{\Gamma}^{T_{1u}^{(1)}} u_A^{\bar{B}_1} u_{\bar{A}}^{2\bar{B}_1} - u_{\Gamma}^{T_{1u}^{(0)}} u_A^{2\bar{B}_1} u_{\bar{A}}^{\bar{B}_1} + u_{\Gamma}^{T_{1u}^{(1)}} u_A^{2\bar{B}_1} u_{\bar{A}}^{\bar{B}_1} + u_{\Gamma}^{T_{1u}^{(0)}} u_{A_2}^{\bar{B}_1} u_{\bar{A}_2}^{2\bar{B}_1} \\
& - u_{\Gamma}^{T_{1u}^{(2)}} u_{A_2}^{\bar{B}_1} u_{\bar{A}_2}^{2\bar{B}_1} - u_{\Gamma}^{T_{1u}^{(0)}} u_{A_2}^{2\bar{B}_1} u_{\bar{A}_2}^{\bar{B}_1} + u_{\Gamma}^{T_{1u}^{(2)}} u_{A_2}^{2\bar{B}_1} u_{\bar{A}_2}^{\bar{B}_1} + u_{\Gamma}^{T_{1u}^{(1)}} u_{\bar{A}_1}^{2\bar{B}_1} u_{A_1}^{\bar{B}_1} + u_{\Gamma}^{T_{1u}^{(2)}} u_{\bar{A}_1}^{2\bar{B}_1} u_{A_1}^{\bar{B}_1} \\
& - u_{\Gamma}^{T_{1u}^{(1)}} u_{\bar{A}_1}^{\bar{B}_1} u_{A_1}^{2\bar{B}_1} - u_{\Gamma}^{T_{1u}^{(2)}} u_{\bar{A}_1}^{\bar{B}_1} u_{A_1}^{2\bar{B}_1} + u_{\Gamma}^{T_{1u}^{(0)}} u_{\bar{A}_4}^{2\bar{B}_1} u_{A_4}^{\bar{B}_1} + u_{\Gamma}^{T_{1u}^{(2)}} u_{\bar{A}_4}^{2\bar{B}_1} u_{A_4}^{\bar{B}_1} - u_{\Gamma}^{T_{1u}^{(0)}} u_{\bar{A}_4}^{\bar{B}_1} u_{A_4}^{2$$

[illegible]



[illegible]

[illegible]

$$\begin{aligned}
& -u_{X_1}^{E_g^{(0)}} u_{A_1 A_1}^{A_2} - u_{X_1}^{E_g^{(1)}} u_{A_1 A_1}^{A_2} - u_{A_4}^{E_g^{(0)}} u_{A_4}^{A_2} u_{X_2}^{E_g^{(0)}} - u_{A_4}^{A_2} u_{A_4}^{E_g^{(1)}} u_{X_2}^{E_g^{(1)}} - u_{X_1}^{E_g^{(0)}} u_{A_3}^{A_1} u_{A_3}^{A_2} \\
& + u_{X_1}^{E_g^{(1)}} u_{A_3}^{A_1} u_{A_3}^{A_2} + u_{A_2}^{A_1} u_{A_2}^{A_2} u_{X_2}^{E_g^{(0)}} - u_{A_2}^{A_1} u_{A_2}^{A_2} u_{X_2}^{E_g^{(1)}} + u_{X_2}^{E_g^{(0)}} u_{A_4}^{A_1} u_{A_4}^{A_2} + u_{X_2}^{E_g^{(1)}} u_{A_4}^{A_1} u_{A_4}^{A_2} \\
& + u_{A_3}^{A_1} u_{A_3}^{A_2} u_{X_1}^{E_g^{(0)}} - u_{A_3}^{A_1} u_{A_3}^{A_2} u_{X_1}^{E_g^{(1)}} + u_{X_1}^{E_g^{(0)}} u_{A_1}^{A_1} u_{A_1}^{A_2} + u_{X_1}^{E_g^{(1)}} u_{A_1}^{A_1} u_{A_1}^{A_2}) \\
+ d_{X \bar{A} \bar{A}}^{E_g A_1 B_1} & (-u_X^{E_g^{(0)}} u_{\bar{A}}^{A_1} u_{\bar{A}}^{B_1} - u_X^{E_g^{(1)}} u_{\bar{A}}^{A_1} u_{\bar{A}}^{B_1} + u_A^{A_1} u_A^{B_1} u_X^{E_g^{(0)}} + u_A^{A_1} u_A^{B_1} u_X^{E_g^{(1)}} - u_{A_5}^{A_1} u_{A_5}^{B_1} u_X^{E_g^{(0)}} \\
& + u_{A_5}^{A_1} u_{A_5}^{B_1} u_X^{E_g^{(1)}} + u_X^{E_g^{(0)}} u_{A_5}^{A_1} u_{A_5}^{B_1} - u_X^{E_g^{(1)}} u_{A_5}^{A_1} u_{A_5}^{B_1} + u_{X_2}^{E_g^{(0)}} u_{A_2}^{A_1} u_{A_2}^{B_1} + u_{X_2}^{E_g^{(1)}} u_{A_2}^{A_1} u_{A_2}^{B_1} \\
& - u_{X_1}^{E_g^{(0)}} u_{A_1}^{A_1} u_{A_1}^{B_1} + u_{X_1}^{E_g^{(1)}} u_{A_1}^{A_1} u_{A_1}^{B_1} + u_{A_4}^{A_1} u_{A_4}^{B_1} u_{X_2}^{E_g^{(0)}} - u_{A_4}^{A_1} u_{A_4}^{B_1} u_{X_2}^{E_g^{(1)}} - u_{X_1}^{E_g^{(0)}} u_{A_3}^{A_1} u_{A_3}^{B_1} \\
& - u_{X_1}^{E_g^{(1)}} u_{A_3}^{A_1} u_{A_3}^{B_1} - u_{A_2}^{A_1} u_{A_2}^{B_1} u_{X_2}^{E_g^{(0)}} - u_{A_2}^{A_1} u_{A_2}^{B_1} u_{X_2}^{E_g^{(1)}} - u_{X_2}^{E_g^{(0)}} u_{A_4}^{A_1} u_{A_4}^{B_1} + u_{X_2}^{E_g^{(1)}} u_{A_4}^{A_1} u_{A_4}^{B_1} \\
& + u_{A_3}^{A_1} u_{A_3}^{B_1} u_{X_1}^{E_g^{(0)}} + u_{A_3}^{A_1} u_{A_3}^{B_1} u_{X_1}^{E_g^{(1)}} + u_{X_1}^{E_g^{(0)}} u_{A_1}^{A_1} u_{A_1}^{B_1} - u_{X_1}^{E_g^{(1)}} u_{A_1}^{A_1} u_{A_1}^{B_1}) \\
+ d_{X \bar{A} \bar{A}}^{E_g A_1 {}^1 B_1} & (-u_X^{E_g^{(0)}} u_{\bar{A}}^{A_1} u_{\bar{A}}^{1 B_1} - u_X^{E_g^{(1)}} u_{\bar{A}}^{A_1} u_{\bar{A}}^{1 B_1} + u_A^{A_1} u_A^{1 B_1} u_X^{E_g^{(0)}} + u_A^{A_1} u_A^{1 B_1} u_X^{E_g^{(1)}} - u_{A_5}^{A_1} u_{A_5}^{1 B_1} u_X^{E_g^{(0)}} \\
& + u_{A_5}^{A_1} u_{A_5}^{1 B_1} u_X^{E_g^{(1)}} + u_X^{E_g^{(0)}} u_{A_5}^{A_1} u_{A_5}^{1 B_1} - u_X^{E_g^{(1)}} u_{A_5}^{A_1} u_{A_5}^{1 B_1} + u_{X_2}^{E_g^{(0)}} u_{A_2}^{A_1} u_{A_2}^{1 B_1} + u_{X_2}^{E_g^{(1)}} u_{A_2}^{A_1} u_{A_2}^{1 B_1} \\
& - u_{X_1}^{E_g^{(0)}} u_{A_1}^{A_1} u_{A_1}^{1 B_1} + u_{X_1}^{E_g^{(1)}} u_{A_1}^{A_1} u_{A_1}^{1 B_1} + u_{A_4}^{A_1} u_{A_4}^{1 B_1} u_{X_2}^{E_g^{(0)}} - u_{A_4}^{A_1} u_{A_4}^{1 B_1} u_{X_2}^{E_g^{(1)}} - u_{X_1}^{E_g^{(0)}} u_{A_3}^{A_1} u_{A_3}^{1 B_1} \\
& - u_{X_1}^{E_g^{(1)}} u_{A_3}^{A_1} u_{A_3}^{1 B_1} - u_{A_2}^{A_1} u_{A_2}^{1 B_1} u_{X_2}^{E_g^{(0)}} - u_{A_2}^{A_1} u_{A_2}^{1 B_1} u_{X_2}^{E_g^{(1)}} - u_{X_2}^{E_g^{(0)}} u_{A_4}^{A_1} u_{A_4}^{1 B_1} + u_{X_2}^{E_g^{(1)}} u_{A_4}^{A_1} u_{A_4}^{1 B_1} \\
& + u_{A_3}^{A_1} u_{A_3}^{1 B_1} u_{X_1}^{E_g^{(0)}} + u_{A_3}^{A_1} u_{A_3}^{1 B_1} u_{X_1}^{E_g^{(1)}} + u_{X_1}^{E_g^{(0)}} u_{A_1}^{A_1} u_{A_1}^{1 B_1} - u_{X_1}^{E_g^{(1)}} u_{A_1}^{A_1} u_{A_1}^{1 B_1}) \\
+ d_{X \bar{A} \bar{A}}^{E_g A_1 {}^2 B_1} & (-u_X^{E_g^{(0)}} u_{\bar{A}}^{A_1} u_{\bar{A}}^{2 B_1} - u_X^{E_g^{(1)}} u_{\bar{A}}^{A_1} u_{\bar{A}}^{2 B_1} + u_A^{A_1} u_A^{2 B_1} u_X^{E_g^{(0)}} + u_A^{A_1} u_A^{2 B_1} u_X^{E_g^{(1)}} - u_{A_5}^{A_1} u_{A_5}^{2 B_1} u_X^{E_g^{(0)}} \\
& + u_{A_5}^{A_1} u_{A_5}^{2 B_1} u_X^{E_g^{(1)}} + u_X^{E_g^{(0)}} u_{A_5}^{A_1} u_{A_5}^{2 B_1} - u_X^{E_g^{(1)}} u_{A_5}^{A_1} u_{A_5}^{2 B_1} + u_{X_2}^{E_g^{(0)}} u_{A_2}^{A_1} u_{A_2}^{2 B_1} + u_{X_2}^{E_g^{(1)}} u_{A_2}^{A_1} u_{A_2}^{2 B_1} \\
& - u_{X_1}^{E_g^{(0)}} u_{A_1}^{A_1} u_{A_1}^{2 B_1} + u_{X_1}^{E_g^{(1)}} u_{A_1}^{A_1} u_{A_1}^{2 B_1} + u_{A_4}^{A_1} u_{A_4}^{2 B_1} u_{X_2}^{E_g^{(0)}} - u_{A_4}^{A_1} u_{A_4}^{2 B_1} u_{X_2}^{E_g^{(1)}} - u_{X_1}^{E_g^{(0)}} u_{A_3}^{A_1} u_{A_3}^{2 B_1} \\
& - u_{X_1}^{E_g^{(1)}} u_{A_3}^{A_1} u_{A_3}^{2 B_1} - u_{A_2}^{A_1} u_{A_2}^{2 B_1} u_{X_2}^{E_g^{(0)}} - u_{A_2}^{A_1} u_{A_2}^{2 B_1} u_{X_2}^{E_g^{(1)}} - u_{X_2}^{E_g^{(0)}} u_{A_4}^{A_1} u_{A_4}^{2 B_1} + u_{X_2}^{E_g^{(1)}} u_{A_4}^{A_1} u_{A_4}^{2 B_1} \\
& + u_{A_3}^{A_1} u_{A_3}^{2 B_1} u_{X_1}^{E_g^{(0)}} + u_{A_3}^{A_1} u_{A_3}^{2 B_1} u_{X_1}^{E_g^{(1)}} + u_{X_1}^{E_g^{(0)}} u_{A_1}^{A_1} u_{A_1}^{2 B_1} - u_{X_1}^{E_g^{(1)}} u_{A_1}^{A_1} u_{A_1}^{2 B_1}) \\
+ d_{X \bar{A} \bar{A}}^{E_g {}^1 A_1 A_2} & (-u_X^{E_g^{(0)}} u_{\bar{A}}^{1 A_1} u_{\bar{A}}^{A_2} + u_X^{E_g^{(1)}} u_{\bar{A}}^{1 A_1} u_{\bar{A}}^{A_2} + u_A^{1 A_1} u_A^{A_2} u_X^{E_g^{(0)}} - u_A^{1 A_1} u_A^{A_2} u_X^{E_g^{(1)}} - u_{A_5}^{1 A_1} u_{A_5}^{A_2} u_X^{E_g^{(0)}} \\
& - u_{A_5}^{1 A_1} u_{A_5}^{A_2} u_X^{E_g^{(1)}} + u_X^{E_g^{(0)}} u_{A_5}^{1 A_1} u_{A_5}^{A_2} + u_X^{E_g^{(1)}} u_{A_5}^{1 A_1} u_{A_5}^{A_2} - u_{X_2}^{E_g^{(0)}} u_{A_2}^{1 A_1} u_{A_2}^{A_2} + u_{X_2}^{E_g^{(1)}} u_{A_2}^{1 A_1} u_{A_2}^{A_2} \\
& - u_{X_1}^{E_g^{(0)}} u_{A_1}^{1 A_1} u_{A_1}^{A_2} - u_{X_1}^{E_g^{(1)}} u_{A_1}^{1 A_1} u_{A_1}^{A_2} - u_{A_4}^{1 A_1} u_{A_4}^{A_2} u_{X_2}^{E_g^{(0)}} - u_{A_4}^{1 A_1} u_{A_4}^{A_2} u_{X_2}^{E_g^{(1)}} - u_{X_1}^{E_g^{(0)}} u_{A_3}^{1 A_1} u_{A_3}^{A_2} \\
& + u_{X_1}^{E_g^{(1)}} u_{A_3}^{1 A_1} u_{A_3}^{A_2} + u_{A_2}^{1 A_1} u_{A_2}^{A_2} u_{X_2}^{E_g^{(0)}} - u_{A_2}^{1 A_1} u_{A_2}^{A_2} u_{X_2}^{E_g^{(1)}} + u_{X_2}^{E_g^{(0)}} u_{A_4}^{1 A_1} u_{A_4}^{A_2} + u_{X_2}^{E_g^{(1)}} u_{A_4}^{1 A_1} u_{A_4}^{A_2} \\
& + u_{A_3}^{1 A_1} u_{A_3}^{A_2} u_{X_1}^{E_g^{(0)}} - u_{A_3}^{1 A_1} u_{A_3}^{A_2} u_{X_1}^{E_g^{(1)}} + u_{X_1}^{E_g^{(0)}} u_{A_1}^{1 A_1} u_{A_1}^{A_2} + u_{X_1}^{E_g^{(1)}} u_{A_1}^{1 A_1} u_{A_1}^{A_2}) \\
+ d_{X \bar{A} \bar{A}}^{E_g {}^1 A_1 B_1} & (-u_X^{E_g^{($$

$$\begin{aligned}
& +d_{X\bar{A}\bar{A}}^{E_g^1A_1^2B_1^1}(-u_X^{E_g^{(0)}}u_{\bar{A}}^{1A_1}u_{\bar{A}}^{2B_1}-u_X^{E_g^{(1)}}u_{\bar{A}}^{1A_1}u_{\bar{A}}^{2B_1}+u_A^{1A_1}u_A^{2B_1}u_X^{E_g^{(0)}}+u_A^{1A_1}u_A^{2B_1}u_X^{E_g^{(1)}}-u_{A_5}^{1A_1}u_{A_5}^{2B_1}u_X^{E_g^{(0)}} \\
& +u_{A_5}^{1A_1}u_{A_5}^{2B_1}u_X^{E_g^{(1)}}+u_X^{E_g^{(0)}}u_{\bar{A}_5}^{1A_1}u_{\bar{A}_5}^{2B_1}-u_X^{E_g^{(1)}}u_{\bar{A}_5}^{1A_1}u_{\bar{A}_5}^{2B_1}+u_{X_2}^{E_g^{(0)}}u_{\bar{A}_2}^{1A_1}u_{\bar{A}_2}^{2B_1}+u_{X_2}^{E_g^{(1)}}u_{\bar{A}_2}^{1A_1}u_{\bar{A}_2}^{2B_1} \\
& -u_{X_1}^{E_g^{(0)}}u_{\bar{A}_1}^{1A_1}u_{\bar{A}_1}^{2B_1}+u_{X_1}^{E_g^{(1)}}u_{\bar{A}_1}^{1A_1}u_{\bar{A}_1}^{2B_1}+u_{\bar{A}_4}^{1A_1}u_{\bar{A}_4}^{2B_1}u_X^{E_g^{(0)}}-u_{\bar{A}_4}^{1A_1}u_{\bar{A}_4}^{2B_1}u_X^{E_g^{(1)}}-u_{X_1}^{E_g^{(0)}}u_{A_3}^{1A_1}u_{A_3}^{2B_1} \\
& -u_{X_1}^{E_g^{(1)}}u_{A_3}^{1A_1}u_{A_3}^{2B_1}-u_{A_2}^{1A_1}u_{A_2}^{2B_1}u_X^{E_g^{(0)}}-u_{A_2}^{1A_1}u_{A_2}^{2B_1}u_X^{E_g^{(1)}}-u_{X_2}^{E_g^{(0)}}u_{A_4}^{1A_1}u_{A_4}^{2B_1}+u_{X_2}^{E_g^{(1)}}u_{A_4}^{1A_1}u_{A_4}^{2B_1} \\
& +u_{\bar{A}_3}^{1A_1}u_{\bar{A}_3}^{2B_1}u_{X_1}^{E_g^{(0)}}+u_{\bar{A}_3}^{1A_1}u_{\bar{A}_3}^{2B_1}u_{X_1}^{E_g^{(1)}}+u_{X_1}^{E_g^{(0)}}u_{A_1}^{1A_1}u_{A_1}^{2B_1}-u_{X_1}^{E_g^{(1)}}u_{A_1}^{1A_1}u_{A_1}^{2B_1}) \\
& +d_{X\bar{A}\bar{A}}^{E_g^2A_1A_2}(-u_X^{E_g^{(0)}}u_{\bar{A}}^{2A_1}u_{\bar{A}}^{A_2}+u_X^{E_g^{(1)}}u_{\bar{A}}^{2A_1}u_{\bar{A}}^{A_2}+u_A^{2A_1}u_A^{A_2}u_X^{E_g^{(0)}}-u_A^{2A_1}u_A^{A_2}u_X^{E_g^{(1)}}-u_{A_5}^{2A_1}u_{A_5}^{A_2}u_X^{E_g^{(0)}} \\
& -u_{A_5}^{2A_1}u_{A_5}^{A_2}u_X^{E_g^{(1)}}+u_X^{E_g^{(0)}}u_{\bar{A}_5}^{2A_1}u_{\bar{A}_5}^{A_2}-u_X^{E_g^{(1)}}u_{\bar{A}_5}^{2A_1}u_{\bar{A}_5}^{A_2}-u_{X_2}^{E_g^{(0)}}u_{\bar{A}_2}^{2A_1}u_{\bar{A}_2}^{A_2}+u_{X_2}^{E_g^{(1)}}u_{\bar{A}_2}^{2A_1}u_{\bar{A}_2}^{A_2} \\
& -u_{X_1}^{E_g^{(0)}}u_{\bar{A}_1}^{2A_1}u_{\bar{A}_1}^{A_2}-u_{X_1}^{E_g^{(1)}}u_{\bar{A}_1}^{2A_1}u_{\bar{A}_1}^{A_2}-u_{\bar{A}_4}^{2A_1}u_{\bar{A}_4}^{A_2}u_X^{E_g^{(0)}}-u_{\bar{A}_4}^{2A_1}u_{\bar{A}_4}^{A_2}u_X^{E_g^{(1)}}-u_{X_1}^{E_g^{(0)}}u_{A_3}^{2A_1}u_{A_3}^{A_2} \\
& +u_{X_1}^{E_g^{(1)}}u_{A_3}^{2A_1}u_{A_3}^{A_2}+u_{A_2}^{2A_1}u_{A_2}^{A_2}u_X^{E_g^{(0)}}-u_{A_2}^{2A_1}u_{A_2}^{A_2}u_X^{E_g^{(1)}}+u_{X_2}^{E_g^{(0)}}u_{A_4}^{2A_1}u_{A_4}^{A_2}+u_{X_2}^{E_g^{(1)}}u_{A_4}^{2A_1}u_{A_4}^{A_2} \\
& +u_{\bar{A}_3}^{2A_1}u_{\bar{A}_3}^{A_2}u_{X_1}^{E_g^{(0)}}-u_{\bar{A}_3}^{2A_1}u_{\bar{A}_3}^{A_2}u_{X_1}^{E_g^{(1)}}+u_{X_1}^{E_g^{(0)}}u_{A_1}^{2A_1}u_{A_1}^{A_2}+u_{X_1}^{E_g^{(1)}}u_{A_1}^{2A_1}u_{A_1}^{A_2}) \\
& +d_{X\bar{A}\bar{A}}^{E_g^2A_1B_1}(-u_X^{E_g^{(0)}}u_{\bar{A}}^{2A_1}u_{\bar{A}}^{B_1}-u_X^{E_g^{(1)}}u_{\bar{A}}^{2A_1}u_{\bar{A}}^{B_1}+u_A^{2A_1}u_A^{B_1}u_X^{E_g^{(0)}}+u_A^{2A_1}u_A^{B_1}u_X^{E_g^{(1)}}-u_{A_5}^{2A_1}u_{A_5}^{B_1}u_X^{E_g^{(0)}} \\
& +u_{A_5}^{2A_1}u_{A_5}^{B_1}u_X^{E_g^{(1)}}+u_X^{E_g^{(0)}}u_{\bar{A}_5}^{2A_1}u_{\bar{A}_5}^{B_1}-u_X^{E_g^{(1)}}u_{\bar{A}_5}^{2A_1}u_{\bar{A}_5}^{B_1}+u_{X_2}^{E_g^{(0)}}u_{\bar{A}_2}^{2A_1}u_{\bar{A}_2}^{B_1}+u_{X_2}^{E_g^{(1)}}u_{\bar{A}_2}^{2A_1}u_{\bar{A}_2}^{B_1} \\
& -u_{X_1}^{E_g^{(0)}}u_{\bar{A}_1}^{2A_1}u_{\bar{A}_1}^{B_1}+u_{X_1}^{E_g^{(1)}}u_{\bar{A}_1}^{2A_1}u_{\bar{A}_1}^{B_1}+u_{\bar{A}_4}^{2A_1}u_{\bar{A}_4}^{B_1}u_X^{E_g^{(0)}}-u_{\bar{A}_4}^{2A_1}u_{\bar{A}_4}^{B_1}u_X^{E_g^{(1)}}-u_{X_1}^{E_g^{(0)}}u_{A_3}^{2A_1}u_{A_3}^{B_1} \\
& -u_{X_1}^{E_g^{(1)}}u_{A_3}^{2A_1}u_{A_3}^{B_1}-u_{A_2}^{2A_1}u_{A_2}^{B_1}u_X^{E_g^{(0)}}-u_{A_2}^{2A_1}u_{A_2}^{B_1}u_X^{E_g^{(1)}}-u_{X_2}^{E_g^{(0)}}u_{A_4}^{2A_1}u_{A_4}^{B_1}+u_{X_2}^{E_g^{(1)}}u_{A_4}^{2A_1}u_{A_4}^{B_1} \\
& +u_{\bar{A}_3}^{2A_1}u_{\bar{A}_3}^{B_1}u_{X_1}^{E_g^{(0)}}+u_{\bar{A}_3}^{2A_1}u_{\bar{A}_3}^{B_1}u_{X_1}^{E_g^{(1)}}+u_{X_1}^{E_g^{(0)}}u_{A_1}^{2A_1}u_{A_1}^{B_1}-u_{X_1}^{E_g^{(1)}}u_{A_1}^{2A_1}u_{A_1}^{B_1}) \\
& +d_{X\bar{A}\bar{A}}^{E_g^2A_1^1B_1}(-u_X^{E_g^{(0)}}u_{\bar{A}}^{2A_1}u_{\bar{A}}^{1B_1}-u_X^{E_g^{(1)}}u_{\bar{A}}^{2A_1}u_{\bar{A}}^{1B_1}+u_A^{2A_1}u_A^{1B_1}u_X^{E_g^{(0)}}+u_A^{2A_1}u_A^{1B_1}u_X^{E_g^{(1)}}-u_{A_5}^{2A_1}u_{A_5}^{1B_1}u_X^{E_g^{(0)}} \\
& +u_{A_5}^{2A_1}u_{A_5}^{1B_1}u_X^{E_g^{(1)}}+u_X^{E_g^{(0)}}u_{\bar{A}_5}^{2A_1}u_{\bar{A}_5}^{1B_1}-u_X^{E_g^{(1)}}u_{\bar{A}_5}^{2A_1}u_{\bar{A}_5}^{1B_1}+u_{X_2}^{E_g^{(0)}}u_{\bar{A}_2}^{2A_1}u_{\bar{A}_2}^{1B_1}+u_{X_2}^{E_g^{(1)}}u_{\bar{A}_2}^{2A_1}u_{\bar{A}_2}^{1B_1} \\
& -u_{X_1}^{E_g^{(0)}}u_{\bar{A}_1}^{2A_1}u_{\bar{A}_1}^{1B_1}+u_{X_1}^{E_g^{(1)}}u_{\bar{A}_1}^{2A_1}u_{\bar{A}_1}^{1B_1}+u_{\bar{A}_4}^{2A_1}u_{\bar{A}_4}^{1B_1}u_X^{E_g^{(0)}}-u_{\bar{A}_4}^{2A_1}u_{\bar{A}_4}^{1B_1}u_X^{E_g^{(1)}}-u_{X_1}^{E_g^{(0)}}u_{A_3}^{2A_1}u_{A_3}^{1B_1} \\
& -u_{X_1}^{E_g^{(1)}}u_{A_3}^{2A_1}u_{A_3}^{1B_1}-u_{A_2}^{2A_1}u_{A_2}^{1B_1}u_X^{E_g^{(0)}}-u_{A_2}^{2A_1}u_{A_2}^{1B_1}u_X^{E_g^{(1)}}-u_{X_2}^{E_g^{(0)}}u_{A_4}^{2A_1}u_{A_4}^{1B_1}+u_{X_2}^{E_g^{(1)}}u_{A_4}^{2A_1}u_{A_4}^{1B_1} \\
& +u_{\bar{A}_3}^{2A_1}u_{\bar{A}_3}^{1B_1}u_{X_1}^{E_g^{(0)}}+u_{\bar{A}_3}^{2A_1}u_{\bar{A}_3}^{1B_1}u_{X_1}^{E_g^{(1)}}+u_{X_1}^{E_g^{(0)}}u_{A_1}^{2A_1}u_{A_1}^{1B_1}-u_{X_1}^{E_g^{(1)}}u_{A_1}^{2A_1}u_{A_1}^{1B_1}) \\
& +d_{X\bar{A}\bar{A}}^{E_g^2A_1^2B_1}(-u_X^{E_g^{(0)}}u_{\bar{A}}^{2A_1}u_{\bar{A}}^{2B_1}-u_X^{E_g^{(1)}}u_{\bar{A}}^{2A_1}u_{\bar{A}}^{2B_1}+u_A^{2A_1}u_A^{2B_1}u_X^{E_g^{(0)}}+u_A^{2A_1}u_A^{2B_1}u_X^{E_g^{(1)}}-u_{A_5}^{2A_1}u_{A_5}^{2B_1}u_X^{E_g^{(0)}} \\
& +u_{A_5}^{2A_1}u_{A_5}^{2B_1}u_X^{E_g^{(1)}}+u_X^{E_g^{(0)}}u_{\bar{A}_5}^{2A_1}u_{\bar{A}_5}^{2B_1}-u_X^{E_g^{(1)}}u_{\bar{A}_5}^{2A_1}u_{\bar{A}_5}^{2B_1}+u_{X_2}^{E_g$$

$$\begin{aligned}
& -u_{X_1}^{E_g(1)} u_{A_3}^{\bar{1}B_2} u_{A_3}^{E_g(0)} - u_{A_2}^{\bar{1}B_2} u_{A_2}^{\bar{1}B_2} u_{X_2}^{E_g(1)} - u_{A_2}^{\bar{1}B_2} u_{A_2}^{\bar{1}B_2} u_{X_2}^{E_g(0)} - u_{X_2}^{E_g(1)} u_{A_4}^{\bar{1}B_2} u_{A_4}^{E_g(1)} + u_{X_2}^{E_g(1)} u_{A_4}^{\bar{1}B_2} u_{A_4}^{E_g(0)} \\
& + u_{A_3}^{\bar{1}B_2} u_{A_3}^{\bar{1}B_2} u_{X_1}^{E_g(0)} + u_{A_3}^{\bar{1}B_2} u_{A_3}^{\bar{1}B_2} u_{X_1}^{E_g(1)} + u_{X_1}^{E_g(0)} u_{A_1}^{\bar{1}B_2} u_{A_1}^{E_g(1)} - u_{X_1}^{E_g(1)} u_{A_1}^{\bar{1}B_2} u_{A_1}^{E_g(0)} \\
& + d_X^{E_g B_2 B_1} (-u_{X'}^{E_g(0)} u_{\bar{A}}^{\bar{1}B_2} u_{\bar{A}}^{B_1} + u_{X'}^{E_g(1)} u_{\bar{A}}^{\bar{1}B_2} u_{\bar{A}}^{B_1} + u_A^{B_2} u_A^{B_1} u_X^{E_g(0)} - u_A^{B_2} u_A^{B_1} u_X^{E_g(1)} - u_{A_5}^{B_2} u_{A_5}^{B_1} u_X^{E_g(0)} \\
& - u_{A_5}^{B_2} u_{A_5}^{B_1} u_X^{E_g(1)} + u_X^{E_g(0)} u_{A_5}^{B_2} u_{A_5}^{B_1} + u_X^{E_g(1)} u_{A_5}^{B_2} u_{A_5}^{B_1} - u_{X_2}^{E_g(0)} u_{A_2}^{B_2} u_{A_2}^{B_1} + u_{X_2}^{E_g(1)} u_{A_2}^{B_2} u_{A_2}^{B_1} \\
& - u_{X_1}^{E_g(0)} u_{A_1}^{B_2} u_{A_1}^{B_1} - u_{X_1}^{E_g(1)} u_{A_1}^{B_2} u_{A_1}^{B_1} - u_{A_4}^{B_2} u_{A_4}^{B_1} u_{X_2}^{E_g(0)} - u_{A_4}^{B_2} u_{A_4}^{B_1} u_{X_2}^{E_g(1)} - u_{X_1}^{E_g(0)} u_{A_3}^{B_2} u_{A_3}^{B_1} \\
& + u_{X_1}^{E_g(1)} u_{A_3}^{B_2} u_{A_3}^{B_1} + u_{A_2}^{B_2} u_{A_2}^{B_1} u_{X_2}^{E_g(0)} - u_{A_2}^{B_2} u_{A_2}^{B_1} u_{X_2}^{E_g(1)} + u_{X_2}^{E_g(0)} u_{A_4}^{B_2} u_{A_4}^{B_1} + u_{X_2}^{E_g(1)} u_{A_4}^{B_2} u_{A_4}^{B_1} \\
& + u_{A_3}^{B_2} u_{A_3}^{B_1} u_{X_1}^{E_g(0)} - u_{A_3}^{B_2} u_{A_3}^{B_1} u_{X_1}^{E_g(1)} + u_{X_1}^{E_g(0)} u_{A_1}^{B_2} u_{A_1}^{B_1} + u_{X_1}^{E_g(1)} u_{A_1}^{B_2} u_{A_1}^{B_1}) \\
& + d_X^{E_g \bar{1}B_2 B_1} (-u_{X'}^{E_g(0)} u_{\bar{A}}^{\bar{1}B_2} u_{\bar{A}}^{B_1} + u_{X'}^{E_g(1)} u_{\bar{A}}^{\bar{1}B_2} u_{\bar{A}}^{B_1} + u_A^{\bar{1}B_2} u_A^{B_1} u_X^{E_g(0)} - u_A^{\bar{1}B_2} u_A^{B_1} u_X^{E_g(1)} - u_{A_5}^{\bar{1}B_2} u_{A_5}^{B_1} u_X^{E_g(0)} \\
& - u_{A_5}^{\bar{1}B_2} u_{A_5}^{B_1} u_X^{E_g(1)} + u_X^{E_g(0)} u_{A_5}^{\bar{1}B_2} u_{A_5}^{B_1} + u_X^{E_g(1)} u_{A_5}^{\bar{1}B_2} u_{A_5}^{B_1} - u_{X_2}^{E_g(0)} u_{A_2}^{\bar{1}B_2} u_{A_2}^{B_1} + u_{X_2}^{E_g(1)} u_{A_2}^{\bar{1}B_2} u_{A_2}^{B_1} \\
& - u_{X_1}^{E_g(0)} u_{A_1}^{\bar{1}B_2} u_{A_1}^{B_1} - u_{X_1}^{E_g(1)} u_{A_1}^{\bar{1}B_2} u_{A_1}^{B_1} - u_{A_4}^{\bar{1}B_2} u_{A_4}^{B_1} u_{X_2}^{E_g(0)} - u_{A_4}^{\bar{1}B_2} u_{A_4}^{B_1} u_{X_2}^{E_g(1)} - u_{X_1}^{E_g(0)} u_{A_3}^{\bar{1}B_2} u_{A_3}^{B_1} \\
& + u_{X_1}^{E_g(1)} u_{A_3}^{\bar{1}B_2} u_{A_3}^{B_1} + u_{A_2}^{\bar{1}B_2} u_{A_2}^{B_1} u_{X_2}^{E_g(0)} - u_{A_2}^{\bar{1}B_2} u_{A_2}^{B_1} u_{X_2}^{E_g(1)} + u_{X_2}^{E_g(0)} u_{A_4}^{\bar{1}B_2} u_{A_4}^{B_1} + u_{X_2}^{E_g(1)} u_{A_4}^{\bar{1}B_2} u_{A_4}^{B_1} \\
& + u_{A_3}^{\bar{1}B_2} u_{A_3}^{B_1} u_{X_1}^{E_g(0)} - u_{A_3}^{\bar{1}B_2} u_{A_3}^{B_1} u_{X_1}^{E_g(1)} + u_{X_1}^{E_g(0)} u_{A_1}^{\bar{1}B_2} u_{A_1}^{B_1} + u_{X_1}^{E_g(1)} u_{A_1}^{\bar{1}B_2} u_{A_1}^{B_1}) \\
& + d_X^{E_g B_2 \bar{1}B_1} (-u_{X'}^{E_g(0)} u_{\bar{A}}^{\bar{1}B_2} u_{\bar{A}}^{\bar{1}B_1} + u_{X'}^{E_g(1)} u_{\bar{A}}^{\bar{1}B_2} u_{\bar{A}}^{\bar{1}B_1} + u_A^{B_2} u_A^{\bar{1}B_1} u_X^{E_g(0)} - u_A^{B_2} u_A^{\bar{1}B_1} u_X^{E_g(1)} - u_{A_5}^{B_2} u_{A_5}^{\bar{1}B_1} u_X^{E_g(0)} \\
& - u_{A_5}^{B_2} u_{A_5}^{\bar{1}B_1} u_X^{E_g(1)} + u_X^{E_g(0)} u_{A_5}^{B_2} u_{A_5}^{\bar{1}B_1} + u_X^{E_g(1)} u_{A_5}^{B_2} u_{A_5}^{\bar{1}B_1} - u_{X_2}^{E_g(0)} u_{A_2}^{B_2} u_{A_2}^{\bar{1}B_1} + u_{X_2}^{E_g(1)} u_{A_2}^{B_2} u_{A_2}^{\bar{1}B_1} \\
& - u_{X_1}^{E_g(0)} u_{A_1}^{B_2} u_{A_1}^{\bar{1}B_1} - u_{X_1}^{E_g(1)} u_{A_1}^{B_2} u_{A_1}^{\bar{1}B_1} - u_{A_4}^{B_2} u_{A_4}^{\bar{1}B_1} u_{X_2}^{E_g(0)} - u_{A_4}^{B_2} u_{A_4}^{\bar{1}B_1} u_{X_2}^{E_g(1)} - u_{X_1}^{E_g(0)} u_{A_3}^{B_2} u_{A_3}^{\bar{1}B_1} \\
& + u_{X_1}^{E_g(1)} u_{A_3}^{B_2} u_{A_3}^{\bar{1}B_1} + u_{A_2}^{B_2} u_{A_2}^{\bar{1}B_1} u_{X_2}^{E_g(0)} - u_{A_2}^{B_2} u_{A_2}^{\bar{1}B_1} u_{X_2}^{E_g(1)} + u_{X_2}^{E_g(0)} u_{A_4}^{B_2} u_{A_4}^{\bar{1}B_1} + u_{X_2}^{E_g(1)} u_{A_4}^{B_2} u_{A_4}^{\bar{1}B_1} \\
& + u_{A_3}^{B_2} u_{A_3}^{\bar{1}B_1} u_{X_1}^{E_g(0)} - u_{A_3}^{B_2} u_{A_3}^{\bar{1}B_1} u_{X_1}^{E_g(1)} + u_{X_1}^{E_g(0)} u_{A_1}^{B_2} u_{A_1}^{\bar{1}B_1} + u_{X_1}^{E_g(1)} u_{A_1}^{B_2} u_{A_1}^{\bar{1}B_1}) \\
& + d_X^{E_g \bar{1}B_2 \bar{1}B_1} (-u_{X'}^{E_g(0)} u_{\bar{A}}^{\bar{1}B_2} u_{\bar{A}}^{\bar{1}B_1} + u_{X'}^{E_g(1)} u_{\bar{A}}^{\bar{1}B_2} u_{\bar{A}}^{\bar{1}B_1} + u_A^{\bar{1}B_2} u_A^{\bar{1}B_1} u_X^{E_g(0)} - u_A^{\bar{1}B_2} u_A^{\bar{1}B_1} u_X^{E_g(1)} - u_{A_5}^{\bar{1}B_2} u_{A_5}^{\bar{1}B_1} u_X^{E_g(0)} \\
& - u_{A_5}^{\bar{1}B_2} u_{A_5}^{\bar{1}B_1} u_X^{E_g(1)} + u_X^{E_g(0)} u_{A_5}^{\bar{1}B_2} u_{A_5}^{\bar{1}B_1} + u_X^{E_g(1)} u_{A_5}^{\bar{1}B_2} u_{A_5}^{\bar{1}B_1} - u_{X_2}^{E_g(0)} u_{A_2}^{\bar{1}B_2} u_{A_2}^{\bar{1}B_1} + u_{X_2}^{E_g(1)} u_{A_2}^{\bar{1}B_2} u_{A_2}^{\bar{1}B_1} \\
& - u_{X_1}^{E_g(0)} u_{A_1}^{\bar{1}B_2} u_{A_1}^{\bar{1}B_1} - u_{X_1}^{E_g(1)} u_{A_1}^{\bar{1}B_2} u_{A_1}^{\bar{1}B_1} - u_{A_4}^{\bar{1}B_2} u_{A_4}^{\bar{1}B_1} u_{X_2}^{E_g(0)} - u_{A_4}^{\bar{1}B_2} u_{A_4}^{\bar{1}B_1} u_{X_2}^{E_g(1)} - u_{X_1}^{E_g(0)} u_{A_3}^{\bar{1}B_2} u_{A_3}^{\bar{1}B_1} \\
& + u_{X_1}^{E_g(1)} u_{A_3}^{\bar{1}B_2} u_{A_3}^{\bar{1}B_1} + u_{A_2}^{\bar{1}B_2} u_{A_2}^{\bar{1}B_1} u_{X_2}^{E_g(0)} - u_{A_2}^{\bar{1}B_2} u_{A_2}^{\bar{1}B_1} u_{X_2}^{E_g(1)} + u_{X_2}^{E_g(0)} u_{A_4}^{\bar{1}B_2} u_{A_4}^{\bar{1}B_1} + u_{X_2}^{E_g(1)} u_{A_4}^{\bar{1}B_2} u_{A_4}^{\bar{1}B_1} \\
& + u_{A_3}^{\bar{1}B_2} u_{A$$

14







$$\begin{aligned}
& + u_{A_5}^{1A_1} u_{A_5}^{1B_2} u_X^{E_u^{(1)}} + u_X^{E_u^{(0)}} u_{A_5}^{1A_1} u_{A_5}^{1B_2} - u_X^{E_u^{(1)}} u_{A_5}^{1A_1} u_{A_5}^{1B_2} + u_{X_2}^{E_u^{(0)}} u_{A_2}^{1A_1} u_{A_2}^{1B_2} + u_{X_2}^{E_u^{(1)}} u_{A_2}^{1A_1} u_{A_2}^{1B_2} \\
& - u_{X_1}^{E_u^{(0)}} u_{A_1}^{1A_1} u_{A_1}^{1B_2} + u_{X_1}^{E_u^{(1)}} u_{A_1}^{1A_1} u_{A_1}^{1B_2} + u_{A_4}^{1A_1} u_{A_4}^{1B_2} u_{X_2}^{E_u^{(0)}} - u_{A_4}^{1A_1} u_{A_4}^{1B_2} u_{X_2}^{E_u^{(1)}} - u_{X_1}^{E_u^{(0)}} u_{A_3}^{1A_1} u_{A_3}^{1B_2} \\
& - u_{X_1}^{E_u^{(1)}} u_{A_3}^{1A_1} u_{A_3}^{1B_2} - u_{A_2}^{1A_1} u_{A_2}^{1B_2} u_{X_2}^{E_u^{(0)}} - u_{A_2}^{1A_1} u_{A_2}^{1B_2} u_{X_2}^{E_u^{(1)}} - u_{X_2}^{E_u^{(0)}} u_{A_4}^{1A_1} u_{A_4}^{1B_2} + u_{X_2}^{E_u^{(1)}} u_{A_4}^{1A_1} u_{A_4}^{1B_2} \\
& + u_{A_3}^{1A_1} u_{A_3}^{1B_2} u_{X_1}^{E_u^{(0)}} + u_{A_3}^{1A_1} u_{A_3}^{1B_2} u_{X_1}^{E_u^{(1)}} + u_{X_1}^{E_u^{(0)}} u_{A_1}^{1A_1} u_{A_1}^{1B_2} - u_{X_1}^{E_u^{(1)}} u_{A_1}^{1A_1} u_{A_1}^{1B_2} \\
& + d_X^{E_u^{2A_1} 2A_1} (-u_X^{E_u^{(0)}} u_{A_1}^{2A_1} u_{A_1}^{2A_1} + u_X^{E_u^{(1)}} u_{A_1}^{2A_1} u_{A_1}^{2A_1} + u_A^{2A_1} u_A^{2A_1} u_X^{E_u^{(0)}} - u_A^{2A_1} u_A^{2A_1} u_X^{E_u^{(1)}} - u_{A_5}^{2A_1} u_{A_5}^{2A_1} u_X^{E_u^{(0)}} \\
& - u_{A_5}^{2A_1} u_{A_5}^{2A_1} u_X^{E_u^{(1)}} + u_X^{E_u^{(0)}} u_{A_5}^{2A_1} u_{A_5}^{2A_1} + u_X^{E_u^{(1)}} u_{A_5}^{2A_1} u_{A_5}^{2A_1} - u_{X_2}^{E_u^{(0)}} u_{A_2}^{2A_1} u_{A_2}^{2A_1} + u_{X_2}^{E_u^{(1)}} u_{A_2}^{2A_1} u_{A_2}^{2A_1} \\
& - u_{X_1}^{E_u^{(0)}} u_{A_1}^{2A_1} u_{A_1}^{2A_1} - u_{X_1}^{E_u^{(1)}} u_{A_1}^{2A_1} u_{A_1}^{2A_1} - u_{A_4}^{2A_1} u_{A_4}^{2A_1} u_{X_2}^{E_u^{(0)}} - u_{A_4}^{2A_1} u_{A_4}^{2A_1} u_{X_2}^{E_u^{(1)}} - u_{X_1}^{E_u^{(0)}} u_{A_3}^{2A_1} u_{A_3}^{2A_1} \\
& + u_{X_1}^{E_u^{(1)}} u_{A_3}^{2A_1} u_{A_3}^{2A_1} + u_{A_2}^{2A_1} u_{A_2}^{2A_1} u_{X_2}^{E_u^{(0)}} - u_{A_2}^{2A_1} u_{A_2}^{2A_1} u_{X_2}^{E_u^{(1)}} + u_{X_2}^{E_u^{(0)}} u_{A_4}^{2A_1} u_{A_4}^{2A_1} + u_{X_2}^{E_u^{(1)}} u_{A_4}^{2A_1} u_{A_4}^{2A_1} \\
& + u_{A_3}^{2A_1} u_{A_3}^{2A_1} u_{X_1}^{E_u^{(0)}} - u_{A_3}^{2A_1} u_{A_3}^{2A_1} u_{X_1}^{E_u^{(1)}} + u_{X_1}^{E_u^{(0)}} u_{A_1}^{2A_1} u_{A_1}^{2A_1} + u_{X_1}^{E_u^{(1)}} u_{A_1}^{2A_1} u_{A_1}^{2A_1}) \\
& + d_X^{E_u^{2A_1} B_2} (-u_X^{E_u^{(0)}} u_{A_1}^{2A_1} u_{A_1}^{B_2} - u_X^{E_u^{(1)}} u_{A_1}^{2A_1} u_{A_1}^{B_2} + u_A^{2A_1} u_A^{B_2} u_X^{E_u^{(0)}} + u_A^{2A_1} u_A^{B_2} u_X^{E_u^{(1)}} - u_{A_5}^{2A_1} u_{A_5}^{B_2} u_X^{E_u^{(0)}} \\
& + u_{A_5}^{2A_1} u_{A_5}^{B_2} u_X^{E_u^{(1)}} + u_X^{E_u^{(0)}} u_{A_5}^{2A_1} u_{A_5}^{B_2} - u_X^{E_u^{(1)}} u_{A_5}^{2A_1} u_{A_5}^{B_2} + u_{X_2}^{E_u^{(0)}} u_{A_2}^{2A_1} u_{A_2}^{B_2} + u_{X_2}^{E_u^{(1)}} u_{A_2}^{2A_1} u_{A_2}^{B_2} \\
& - u_{X_1}^{E_u^{(0)}} u_{A_1}^{2A_1} u_{A_1}^{B_2} + u_{X_1}^{E_u^{(1)}} u_{A_1}^{2A_1} u_{A_1}^{B_2} + u_{A_4}^{2A_1} u_{A_4}^{B_2} u_{X_2}^{E_u^{(0)}} - u_{A_4}^{2A_1} u_{A_4}^{B_2} u_{X_2}^{E_u^{(1)}} - u_{X_1}^{E_u^{(0)}} u_{A_3}^{2A_1} u_{A_3}^{B_2} \\
& - u_{X_1}^{E_u^{(1)}} u_{A_3}^{2A_1} u_{A_3}^{B_2} - u_{A_2}^{2A_1} u_{A_2}^{B_2} u_{X_2}^{E_u^{(0)}} - u_{A_2}^{2A_1} u_{A_2}^{B_2} u_{X_2}^{E_u^{(1)}} - u_{X_2}^{E_u^{(0)}} u_{A_4}^{2A_1} u_{A_4}^{B_2} + u_{X_2}^{E_u^{(1)}} u_{A_4}^{2A_1} u_{A_4}^{B_2} \\
& + u_{A_3}^{2A_1} u_{A_3}^{B_2} u_{X_1}^{E_u^{(0)}} + u_{A_3}^{2A_1} u_{A_3}^{B_2} u_{X_1}^{E_u^{(1)}} + u_{X_1}^{E_u^{(0)}} u_{A_1}^{2A_1} u_{A_1}^{B_2} - u_{X_1}^{E_u^{(1)}} u_{A_1}^{2A_1} u_{A_1}^{B_2}) \\
& + d_X^{E_u^{2A_1} 1B_2} (-u_X^{E_u^{(0)}} u_{A_1}^{2A_1} u_{A_1}^{1B_2} - u_X^{E_u^{(1)}} u_{A_1}^{2A_1} u_{A_1}^{1B_2} + u_A^{2A_1} u_A^{1B_2} u_X^{E_u^{(0)}} + u_A^{2A_1} u_A^{1B_2} u_X^{E_u^{(1)}} - u_{A_5}^{2A_1} u_{A_5}^{1B_2} u_X^{E_u^{(0)}} \\
& + u_{A_5}^{2A_1} u_{A_5}^{1B_2} u_X^{E_u^{(1)}} + u_X^{E_u^{(0)}} u_{A_5}^{2A_1} u_{A_5}^{1B_2} - u_X^{E_u^{(1)}} u_{A_5}^{2A_1} u_{A_5}^{1B_2} + u_{X_2}^{E_u^{(0)}} u_{A_2}^{2A_1} u_{A_2}^{1B_2} + u_{X_2}^{E_u^{(1)}} u_{A_2}^{2A_1} u_{A_2}^{1B_2} \\
& - u_{X_1}^{E_u^{(0)}} u_{A_1}^{2A_1} u_{A_1}^{1B_2} + u_{X_1}^{E_u^{(1)}} u_{A_1}^{2A_1} u_{A_1}^{1B_2} + u_{A_4}^{2A_1} u_{A_4}^{1B_2} u_{X_2}^{E_u^{(0)}} - u_{A_4}^{2A_1} u_{A_4}^{1B_2} u_{X_2}^{E_u^{(1)}} - u_{X_1}^{E_u^{(0)}} u_{A_3}^{2A_1} u_{A_3}^{1B_2} \\
& - u_{X_1}^{E_u^{(1)}} u_{A_3}^{2A_1} u_{A_3}^{1B_2} - u_{A_2}^{2A_1} u_{A_2}^{1B_2} u_{X_2}^{E_u^{(0)}} - u_{A_2}^{2A_1} u_{A_2}^{1B_2} u_{X_2}^{E_u^{(1)}} - u_{X_2}^{E_u^{(0)}} u_{A_4}^{2A_1} u_{A_4}^{1B_2} + u_{X_2}^{E_u^{(1)}} u_{A_4}^{2A_1} u_{A_4}^{1B_2} \\
& + u_{A_3}^{2A_1} u_{A_3}^{1B_2} u_{X_1}^{E_u^{(0)}} + u_{A_3}^{2A_1} u_{A_3}^{1B_2} u_{X_1}^{E_u^{(1)}} + u_{X_1}^{E_u^{(0)}} u_{A_1}^{2A_1} u_{A_1}^{1B_2} - u_{X_1}^{E_u^{(1)}} u_{A_1}^{2A_1} u_{A_1}^{1B_2}) \\
& + d_X^{E_u^{A_2} A_2} (-u_X^{E_u^{(0)}} u_{A_1}^{A_2} u_{A_1}^{A_2} + u_X^{E_u^{(1)}} u_{A_1}^{A_2} u_{A_1}^{A_2} + u_A^{A_2} u_A^{A_2} u_X^{E_u^{(0)}} - u_A^{A_2} u_A^{A_2} u_X^{E_u^{(1)}} - u_{A_5}^{A_2} u_{A_5}^{A_2} u_X^{E_u^{(0)}} \\
& - u_{A_5}^{A_2} u_{A_5}^{A_2} u_X^{E_u^{(1)}} + u_X^{E_u^{(0)}} u_{A_5}^{A_2} u_{A_5}^{A_2} + u_X^{E_u^{(1)}} u_{A_5}^{A_2} u_{A_5}^{A_2} - u_{X_2}^{E_u^{(0)}} u_{A_2}^{A_2} u_{A_2}^{A_2} + u_{X_2}^{E_u^{(1)}} u_{A_2}^{A_2} u_{A_2}^{A_2} \\
& - u_{X_1}^{E_u^{(0)}} u_{A_1}^{A_2} u_{A_1}^{A_2} - u_{X_1}^{E_u^{(1)}} u_{A_1}^{A_2} u_{A_1}^{A_2} - u_{A_4}^{A_2} u_{A_4}^{A_2} u_{X_2}^{E_u^{(0)}} - u_{A_4}^{A_2} u_{A_4}^{A_2} u_{X_2}^{E_u^{(1)}} - u_{X_1}^{E_u^{(0)}} u_{A_3}^{A_2} u_{A_3}^{A_2} \\
& + u_{X_1}^{E_u^{(1)}} u_{A_3}^{A_2} u_{A_3}^{A_2} + u_{A_2}^{A_2} u_{A_2}^{A_2} u_{X_2}^{E_u^{(0)}} - u_{A_2}^{A_2} u_{A_2}^{A_2} u_{X_2}^{E_u^{(1)}} + u_{X_2}^{E_u^{(0)}} u_{A_4}^{A_2} u_{A_4}^{A_2} + u_{X_2}^{E_u^{($$

[illegible]



[illegible]

[illegible]

[illegible]

[illegible]

$$\begin{aligned}
& + u_{A_3}^{A_1} u_A^{2A_1} u_{A_4}^{1A_1} + u_{A_3}^{2A_1} u_A^{A_1} u_{A_4}^{1A_1} + u_{A_3}^{A_1} u_A^{1A_1} u_{A_4}^{2A_1} + u_{A_3}^{1A_1} u_A^{A_1} u_{A_4}^{2A_1} + u_{A_3}^{A_1} u_{A_5}^{1A_1} u_{A_2}^{2A_1} \\
& + u_{A_3}^{2A_1} u_{A_5}^{A_1} u_{A_2}^{1A_1} + u_{A_3}^{A_1} u_{A_5}^{1A_1} u_{A_2}^{2A_1} + u_{A_3}^{1A_1} u_{A_5}^{2A_1} u_{A_2}^{A_1} + u_{A_3}^{A_1} u_{A_5}^{2A_1} u_{A_2}^{1A_1} + u_{A_3}^{1A_1} u_{A_5}^{2A_1} u_{A_2}^{A_1} \\
& + u_{A_5}^{A_1} u_{A_4}^{1A_1} u_{A_1}^{2A_1} + u_{A_5}^{1A_1} u_{A_4}^{2A_1} u_{A_1}^{A_1} + u_{A_5}^{A_1} u_{A_4}^{1A_1} u_{A_1}^{2A_1} + u_{A_5}^{1A_1} u_{A_4}^{2A_1} u_{A_1}^{A_1} + u_{A_5}^{A_1} u_{A_4}^{1A_1} u_{A_1}^{2A_1} \\
& + u_{A_5}^{2A_1} u_{A_4}^{A_1} u_{A_1}^{1A_1} + u_{A_3}^{A_1} u_{A_2}^{1A_1} u_{A_5}^{2A_1} + u_{A_3}^{1A_1} u_{A_2}^{2A_1} u_{A_5}^{A_1} + u_{A_3}^{A_1} u_{A_2}^{1A_1} u_{A_5}^{2A_1} + u_{A_3}^{1A_1} u_{A_2}^{2A_1} u_{A_5}^{A_1} \\
& + u_{A_3}^{2A_1} u_{A_2}^{A_1} u_{A_5}^{1A_1} + u_{A_3}^{A_1} u_{A_2}^{1A_1} u_{A_5}^{2A_1} + u_{A_1}^{A_1} u_{A_4}^{1A_1} u_{A_5}^{2A_1} + u_{A_1}^{1A_1} u_{A_4}^{2A_1} u_{A_5}^{A_1} + u_{A_1}^{A_1} u_{A_4}^{1A_1} u_{A_5}^{2A_1} \\
& + u_{A_1}^{2A_1} u_{A_4}^{A_1} u_{A_5}^{1A_1} + u_{A_1}^{A_1} u_{A_4}^{1A_1} u_{A_5}^{2A_1} + u_{A_1}^{1A_1} u_{A_4}^{2A_1} u_{A_5}^{A_1} + u_{A_1}^{A_1} u_{A_4}^{1A_1} u_{A_5}^{2A_1} + u_{A_1}^{1A_1} u_{A_4}^{2A_1} u_{A_5}^{A_1} \\
& + d_{A_5 A_4 A_1}^{A_1 A_1 A_2} (u_{A_1}^{A_1} u_{A_2}^{1A_1} u_{A_4}^{A_2} - u_{A_1}^{A_1} u_{A_2}^{A_2} u_{A_4}^{1A_1} - u_{A_1}^{1A_1} u_{A_2}^{A_1} u_{A_4}^{A_2} + u_{A_1}^{1A_1} u_{A_2}^{A_2} u_{A_4}^{A_1} + u_{A_1}^{A_2} u_{A_2}^{A_1} u_{A_4}^{1A_1} \\
& - u_{A_1}^{A_2} u_{A_2}^{1A_1} u_{A_4}^{A_1} - u_{A_3}^{A_1} u_{A_4}^{1A_1} u_{A_2}^{A_2} + u_{A_3}^{1A_1} u_{A_4}^{A_2} u_{A_2}^{1A_1} + u_{A_3}^{A_1} u_{A_4}^{1A_1} u_{A_2}^{A_2} - u_{A_3}^{1A_1} u_{A_4}^{A_2} u_{A_2}^{A_1} \\
& - u_{A_3}^{A_2} u_{A_4}^{A_1} u_{A_2}^{1A_1} + u_{A_3}^{A_2} u_{A_4}^{1A_1} u_{A_2}^{A_1} + u_{A_2}^{A_1} u_{A_4}^{A_2} u_{A_1}^{1A_1} - u_{A_2}^{A_1} u_{A_4}^{1A_1} u_{A_2}^{A_2} - u_{A_2}^{1A_1} u_{A_4}^{A_2} u_{A_1}^{A_1} \\
& + u_{A_2}^{1A_1} u_{A_4}^{A_1} u_{A_2}^{A_2} + u_{A_2}^{A_2} u_{A_4}^{1A_1} u_{A_1}^{A_1} - u_{A_2}^{A_2} u_{A_4}^{A_1} u_{A_1}^{1A_1} - u_{A_3}^{1A_1} u_{A_2}^{A_2} u_{A_4}^{A_1} + u_{A_3}^{A_2} u_{A_4}^{1A_1} u_{A_1}^{A_1} \\
& + u_{A_3}^{A_1} u_{A_2}^{A_2} u_{A_4}^{1A_1} - u_{A_3}^{A_2} u_{A_4}^{A_1} u_{A_1}^{1A_1} - u_{A_3}^{A_1} u_{A_4}^{1A_1} u_{A_2}^{A_2} + u_{A_3}^{1A_1} u_{A_4}^{A_2} u_{A_2}^{A_1} - u_{A_3}^{A_1} u_{A_5}^{1A_1} u_{A_2}^{A_2} \\
& + u_{A_3}^{A_2} u_{A_5}^{A_1} u_{A_2}^{1A_1} + u_{A_3}^{A_1} u_{A_5}^{1A_1} u_{A_2}^{A_2} - u_{A_3}^{A_2} u_{A_5}^{1A_1} u_{A_2}^{A_1} - u_{A_3}^{1A_1} u_{A_5}^{A_2} u_{A_2}^{1A_1} + u_{A_3}^{A_1} u_{A_5}^{2A_1} u_{A_2}^{A_1} \\
& - u_{A_5}^{A_1} u_{A_4}^{1A_1} u_{A_2}^{A_2} + u_{A_5}^{A_1} u_{A_4}^{A_2} u_{A_1}^{1A_1} + u_{A_5}^{1A_1} u_{A_4}^{A_2} u_{A_1}^{A_1} - u_{A_5}^{A_1} u_{A_4}^{1A_1} u_{A_2}^{A_2} - u_{A_5}^{1A_1} u_{A_4}^{A_2} u_{A_1}^{A_1} \\
& + u_{A_5}^{A_2} u_{A_4}^{1A_1} u_{A_1}^{A_1} + u_{A_3}^{A_1} u_{A_2}^{1A_1} u_{A_5}^{A_2} - u_{A_3}^{1A_1} u_{A_2}^{A_2} u_{A_5}^{A_1} - u_{A_3}^{A_1} u_{A_2}^{1A_1} u_{A_5}^{A_2} + u_{A_3}^{1A_1} u_{A_2}^{A_2} u_{A_5}^{A_1} \\
& + u_{A_3}^{A_2} u_{A_2}^{A_1} u_{A_5}^{1A_1} - u_{A_3}^{A_2} u_{A_2}^{1A_1} u_{A_5}^{A_1} - u_{A_1}^{A_1} u_{A_4}^{1A_1} u_{A_5}^{A_2} + u_{A_1}^{1A_1} u_{A_4}^{A_2} u_{A_5}^{A_1} + u_{A_1}^{A_1} u_{A_4}^{1A_1} u_{A_5}^{A_2} \\
& - u_{A_1}^{1A_1} u_{A_4}^{A_2} u_{A_5}^{A_1} - u_{A_1}^{A_2} u_{A_4}^{1A_1} u_{A_5}^{A_1} + u_{A_1}^{A_2} u_{A_4}^{A_1} u_{A_5}^{1A_1}) \\
& + d_{A_5 A_4 A_1}^{A_1 A_1 B_1} (u_{A_1}^{A_1} u_{A_2}^{1A_1} u_{A_4}^{B_1} + u_{A_1}^{A_1} u_{A_2}^{A_2} u_{A_4}^{1A_1} + u_{A_1}^{1A_1} u_{A_2}^{A_1} u_{A_4}^{B_1} + u_{A_1}^{1A_1} u_{A_2}^{A_2} u_{A_4}^{A_1} + u_{A_1}^{B_1} u_{A_2}^{A_1} u_{A_4}^{1A_1} \\
& + u_{A_1}^{B_1} u_{A_2}^{1A_1} u_{A_4}^{A_1} - u_{A_3}^{A_1} u_{A_4}^{1A_1} u_{A_2}^{B_1} - u_{A_3}^{1A_1} u_{A_4}^{A_2} u_{A_2}^{1A_1} - u_{A_3}^{A_1} u_{A_4}^{1A_1} u_{A_2}^{B_1} - u_{A_3}^{1A_1} u_{A_4}^{A_2} u_{A_2}^{A_1} \\
& - u_{A_3}^{B_1} u_{A_4}^{A_1} u_{A_2}^{1A_1} - u_{A_3}^{B_1} u_{A_4}^{1A_1} u_{A_2}^{A_1} - u_{A_2}^{A_1} u_{A_4}^{B_1} u_{A_1}^{1A_1} - u_{A_2}^{A_1} u_{A_4}^{1A_1} u_{A_1}^{B_1} - u_{A_2}^{1A_1} u_{A_4}^{B_1} u_{A_1}^{A_1} \\
& - u_{A_2}^{1A_1} u_{A_4}^{A_1} u_{A_1}^{B_1} - u_{A_2}^{B_1} u_{A_4}^{1A_1} u_{A_1}^{A_1} - u_{B_1} u_{A_4}^{A_1} u_{A_1}^{1A_1} + u_{A_3}^{1A_1} u_{B_1} u_{A_4}^{A_1} + u_{A_3}^{B_1} u_{A_4}^{1A_1} u_{A_1}^{A_1} \\
& + u_{A_3}^{A_1} u_{A_4}^{B_1} u_{A_1}^{1A_1} + u_{A_3}^{B_1} u_{A_4}^{A_1} u_{A_1}^{1A_1} + u_{A_3}^{A_1} u_{A_4}^{1A_1} u_{A_1}^{B_1} + u_{A_3}^{1A_1} u_{A_4}^{B_1} u_{A_1}^{A_1} - u_{A_3}^{B_1} u_{A_5}^{1A_1} u_{A_2}^{A_2} \\
& - u_{A_3}^{B_1} u_{A_5}^{A_1} u_{A_2}^{1A_1} - u_{A_3}^{A_1} u_{A_5}^{1A_1} u_{A_2}^{B_1} - u_{A_3}^{1A_1} u_{A_5}^{A_2} u_{A_2}^{1A_1} - u_{A_3}^{A_1} u_{A_5}^{2A_1} u_{A_2}^{A_1} - u_{A_3}^{1A_1} u_{A_5}^{2A_1} u_{A_2}^{A_1} \\
& + u_{A_5}^{A_1} u_{A_4}^{1A_1} u_{A_1}^{B_1} + u_{A_5}^{A_1} u_{A_4}^{B_1} u_{A_1}^{1A_1} + u_{A_5}^{1A_1} u_{A_4}^{A_2} u_{A_1}^{B_1} + u_{A_5}^{1A_1} u_{A_4}^{1A_1} u_{A_1}^{B_1} + u_{A_5}^{B_1} u_{A$$



$$\begin{aligned}
& - u_{A_1}^{1A_1} u_{A_4}^{B_1} u_{A_5}^{A_1} - u_{A_1}^{B_1} u_{A_4}^{A_1} u_{A_5}^{1A_1} - u_{A_1}^{B_1} u_{A_4}^{1A_1} u_{A_5}^{A_1}) \\
+ d_{A_5 A_4 \bar{A}_1}^{A_1 1A_1 B_1} & (u_{A_1}^{A_1} u_{A_2}^{1A_1} u_{\bar{A}}^{B_1} + u_{A_1}^{A_1} u_{A_2}^{B_1} u_{\bar{A}}^{1A_1} + u_{A_1}^{1A_1} u_{A_2}^{A_1} u_{\bar{A}}^{B_1} + u_{A_1}^{1A_1} u_{A_2}^{B_1} u_{\bar{A}}^{A_1} + u_{A_1}^{B_1} u_{A_2}^{A_1} u_{\bar{A}}^{1A_1} \\
& + u_{A_1}^{B_1} u_{A_2}^{1A_1} u_{\bar{A}}^{A_1} - u_{A_3}^{A_1} u_{A_4}^{1A_1} u_{\bar{A}}^{B_1} - u_{A_3}^{A_1} u_{A_4}^{B_1} u_{\bar{A}}^{1A_1} - u_{A_3}^{1A_1} u_{A_4}^{A_1} u_{\bar{A}}^{B_1} - u_{A_3}^{1A_1} u_{A_4}^{B_1} u_{\bar{A}}^{A_1} \\
& - u_{A_3}^{B_1} u_{A_4}^{A_1} u_{\bar{A}}^{1A_1} - u_{A_3}^{B_1} u_{A_4}^{1A_1} u_{\bar{A}}^{A_1} - u_{A_2}^{A_1} u_A^{B_1} u_{\bar{A}}^{1A_1} - u_{A_2}^{A_1} u_A^{1A_1} u_{\bar{A}}^{B_1} - u_{A_2}^{1A_1} u_A^{A_1} u_{\bar{A}}^{B_1} \\
& - u_{A_2}^{1A_1} u_A^{B_1} u_{\bar{A}}^{A_1} - u_{A_2}^{B_1} u_A^{A_1} u_{\bar{A}}^{1A_1} - u_{A_2}^{B_1} u_A^{1A_1} u_{\bar{A}}^{A_1} + u_{A_3}^{1A_1} u_A^{B_1} u_{\bar{A}}^{A_1} + u_{A_3}^{B_1} u_A^{1A_1} u_{\bar{A}}^{A_1} \\
& + u_{A_3}^{A_1} u_A^{B_1} u_{\bar{A}}^{1A_1} + u_{A_3}^{B_1} u_A^{A_1} u_{\bar{A}}^{1A_1} + u_{A_3}^{A_1} u_A^{1A_1} u_{\bar{A}}^{B_1} + u_{A_3}^{1A_1} u_A^{A_1} u_{\bar{A}}^{B_1} - u_{A_3}^{1A_1} u_{A_5}^{A_1} u_{\bar{A}}^{B_1} \\
& - u_{A_3}^{B_1} u_{A_5}^{A_1} u_{\bar{A}}^{A_1} - u_{A_3}^{A_1} u_{A_5}^{1A_1} u_{\bar{A}}^{B_1} - u_{A_3}^{B_1} u_{A_5}^{1A_1} u_{\bar{A}}^{A_1} - u_{A_3}^{A_1} u_{A_5}^{B_1} u_{\bar{A}}^{1A_1} - u_{A_3}^{1A_1} u_{A_5}^{B_1} u_{\bar{A}}^{A_1} \\
& + u_{A_5}^{A_1} u_{\bar{A}_4}^{1A_1} u_{\bar{A}_1}^{B_1} + u_{A_5}^{A_1} u_{\bar{A}_4}^{B_1} u_{\bar{A}_1}^{1A_1} + u_{A_5}^{1A_1} u_{\bar{A}_4}^{A_1} u_{\bar{A}_1}^{B_1} + u_{A_5}^{1A_1} u_{\bar{A}_4}^{B_1} u_{\bar{A}_1}^{A_1} + u_{A_5}^{B_1} u_{\bar{A}_4}^{A_1} u_{\bar{A}_1}^{1A_1} \\
& + u_{A_5}^{B_1} u_{\bar{A}_4}^{1A_1} u_{\bar{A}_1}^{A_1} + u_{A_3}^{A_1} u_{A_2}^{1A_1} u_{\bar{A}_5}^{B_1} + u_{A_3}^{A_1} u_{A_2}^{B_1} u_{\bar{A}_5}^{1A_1} + u_{A_3}^{1A_1} u_{A_2}^{A_1} u_{\bar{A}_5}^{B_1} + u_{A_3}^{1A_1} u_{A_2}^{B_1} u_{\bar{A}_5}^{A_1} \\
& + u_{A_3}^{B_1} u_{A_2}^{A_1} u_{\bar{A}_5}^{1A_1} + u_{A_3}^{B_1} u_{A_2}^{1A_1} u_{\bar{A}_5}^{A_1} - u_{A_1}^{A_1} u_{A_4}^{1A_1} u_{\bar{A}_5}^{B_1} - u_{A_1}^{A_1} u_{A_4}^{B_1} u_{\bar{A}_5}^{1A_1} - u_{A_1}^{1A_1} u_{A_4}^{A_1} u_{\bar{A}_5}^{B_1} \\
& - u_{A_1}^{1A_1} u_{A_4}^{B_1} u_{\bar{A}_5}^{A_1} - u_{A_1}^{B_1} u_{A_4}^{A_1} u_{\bar{A}_5}^{1A_1} - u_{A_1}^{B_1} u_{A_4}^{1A_1} u_{\bar{A}_5}^{A_1}) \\
+ d_{A_5 A_4 \bar{A}_1}^{A_1 1A_1 B_2} & (u_{A_1}^{A_1} u_{A_2}^{1A_1} u_{\bar{A}}^{B_2} - u_{A_1}^{A_1} u_{A_2}^{B_2} u_{\bar{A}}^{1A_1} - u_{A_1}^{1A_1} u_{A_2}^{A_1} u_{\bar{A}}^{B_2} + u_{A_1}^{1A_1} u_{A_2}^{B_2} u_{\bar{A}}^{A_1} + u_{A_1}^{B_2} u_{A_2}^{A_1} u_{\bar{A}}^{1A_1} \\
& - u_{A_1}^{B_2} u_{A_2}^{1A_1} u_{\bar{A}}^{A_1} + u_{A_3}^{A_1} u_{A_4}^{1A_1} u_{\bar{A}}^{B_2} - u_{A_3}^{A_1} u_{A_4}^{B_2} u_{\bar{A}}^{1A_1} - u_{A_3}^{1A_1} u_{A_4}^{A_1} u_{\bar{A}}^{B_2} + u_{A_3}^{1A_1} u_{A_4}^{B_2} u_{\bar{A}}^{A_1} \\
& + u_{A_3}^{B_2} u_{A_4}^{A_1} u_{\bar{A}}^{1A_1} - u_{A_3}^{B_2} u_{A_4}^{1A_1} u_{\bar{A}}^{A_1} - u_{A_2}^{A_1} u_A^{B_2} u_{\bar{A}_1}^{1A_1} + u_{A_2}^{A_1} u_A^{1A_1} u_{\bar{A}_1}^{B_2} + u_{A_2}^{1A_1} u_A^{A_1} u_{\bar{A}_1}^{B_2} \\
& - u_{A_2}^{1A_1} u_A^{A_1} u_{\bar{A}_1}^{B_2} - u_{A_2}^{B_2} u_A^{1A_1} u_{\bar{A}_1}^{A_1} + u_{A_2}^{B_2} u_A^{A_1} u_{\bar{A}_1}^{1A_1} - u_{A_3}^{1A_1} u_A^{B_2} u_{\bar{A}_4}^{A_1} + u_{A_3}^{B_2} u_A^{1A_1} u_{\bar{A}_4}^{A_1} \\
& + u_{A_3}^{A_1} u_A^{B_2} u_{\bar{A}_4}^{1A_1} - u_{A_3}^{B_2} u_A^{A_1} u_{\bar{A}_4}^{1A_1} - u_{A_3}^{A_1} u_{A_5}^{1A_1} u_{\bar{A}_2}^{B_2} + u_{A_3}^{1A_1} u_{A_5}^{A_1} u_{\bar{A}_2}^{B_2} + u_{A_3}^{1A_1} u_{A_5}^{B_2} u_{\bar{A}_2}^{A_1} \\
& - u_{A_3}^{B_2} u_{A_5}^{A_1} u_{\bar{A}_2}^{1A_1} - u_{A_3}^{A_1} u_{A_5}^{1A_1} u_{\bar{A}_2}^{B_2} + u_{A_3}^{B_2} u_{A_5}^{1A_1} u_{\bar{A}_2}^{A_1} + u_{A_3}^{A_1} u_{A_5}^{B_2} u_{\bar{A}_2}^{1A_1} - u_{A_3}^{1A_1} u_{A_5}^{B_2} u_{\bar{A}_2}^{A_1} \\
& - u_{A_5}^{A_1} u_{\bar{A}_4}^{1A_1} u_{\bar{A}_1}^{B_2} + u_{A_5}^{A_1} u_{\bar{A}_4}^{B_2} u_{\bar{A}_1}^{1A_1} + u_{A_5}^{1A_1} u_{\bar{A}_4}^{A_1} u_{\bar{A}_1}^{B_2} - u_{A_5}^{1A_1} u_{\bar{A}_4}^{B_2} u_{\bar{A}_1}^{A_1} - u_{A_5}^{B_2} u_{\bar{A}_4}^{A_1} u_{\bar{A}_1}^{1A_1} \\
& + u_{A_5}^{B_2} u_{\bar{A}_4}^{1A_1} u_{\bar{A}_1}^{A_1} + u_{A_3}^{A_1} u_{A_2}^{1A_1} u_{\bar{A}_5}^{B_2} - u_{A_3}^{A_1} u_{A_2}^{B_2} u_{\bar{A}_5}^{1A_1} - u_{A_3}^{1A_1} u_{A_2}^{A_1} u_{\bar{A}_5}^{B_2} + u_{A_3}^{1A_1} u_{A_2}^{B_2} u_{\bar{A}_5}^{A_1} \\
& + u_{A_3}^{B_2} u_{A_2}^{A_1} u_{\bar{A}_5}^{1A_1} - u_{A_3}^{B_2} u_{A_2}^{1A_1} u_{\bar{A}_5}^{A_1} + u_{A_1}^{A_1} u_{A_4}^{1A_1} u_{\bar{A}_5}^{B_2} - u_{A_1}^{A_1} u_{A_4}^{B_2} u_{\bar{A}_5}^{1A_1} - u_{A_1}^{1A_1} u_{A_4}^{A_1} u_{\bar{A}_5}^{B_2} \\
& + u_{A_1}^{1A_1} u_{A_4}^{B_2} u_{\bar{A}_5}^{A_1} + u_{A_1}^{B_2} u_{A_4}^{A_1} u_{\bar{A}_5}^{1A_1} - u_{A_1}^{B_2} u_{A_4}^{1A_1} u_{\bar{A}_5}^{A_1}) \\
+ d_{A_5 A_4 \bar{A}_1}^{A_1 1A_1 B_2} & (u_{A_1}^{A_1} u_{A_2}^{1A_1} u_{\bar{A}}^{B_2} - u_{A_1}^{A_1} u_{A_2}^{B_2} u_{\bar{A}}^{1A_1} - u_{A_1}^{1A_1} u_{A_2}^{A_1} u_{\bar{A}}^{B_2} + u_{A_1}^{1A_1} u_{A_2}^{B_2} u_{\bar{A}}^{A_1} + u_{A_1}^{B_2} u_{A_2}^{A_1} u_{\bar{A}}^{1A_1} \\
& - u_{A_1}^{B_2} u_{A_2}^{1A_1} u_{\bar{A}}^{A_1} + u_{A_3}^{A_1} u_{A_4}^{1A_1} u_{\bar{A}}^{B_2} - u_{A_3}^{A_1} u_{A_4}^{B_2} u_{\bar{A}}^{1A_1$$

[illegible]

$$\begin{aligned}
& + u_{A_3}^{2B_1} u_A^{2A_1} u_{A_4}^{2A_1} + u_{A_3}^{2B_1} u_A^{A_1} u_{A_4}^{2A_1} + u_{A_3}^{2A_1} u_A^{2B_1} u_{A_4}^{2B_1} + u_{A_3}^{2A_1} u_A^{A_1} u_{A_4}^{2B_1} - u_{A_3}^{2A_1} u_{A_5}^{2B_1} u_{\bar{A}_2}^{2B_1} \\
& - u_{A_3}^{2B_1} u_{A_5}^{A_1} u_{\bar{A}_2}^{2A_1} - u_{A_3}^{A_1} u_{A_5}^{2A_1} u_{\bar{A}_2}^{2B_1} - u_{A_3}^{2B_1} u_{A_5}^{2A_1} u_{\bar{A}_2}^{A_1} - u_{A_3}^{A_1} u_{A_5}^{2B_1} u_{\bar{A}_2}^{2A_1} - u_{A_3}^{2A_1} u_{A_5}^{2B_1} u_{\bar{A}_2}^{A_1} \\
& + u_{A_5}^{A_1} u_{\bar{A}_4}^{2A_1} u_{\bar{A}_1}^{2B_1} + u_{A_5}^{A_1} u_{\bar{A}_4}^{2B_1} u_{\bar{A}_1}^{2A_1} + u_{A_5}^{2B_1} u_{\bar{A}_4}^{A_1} u_{\bar{A}_1}^{2B_1} + u_{A_5}^{2A_1} u_{\bar{A}_4}^{A_1} u_{\bar{A}_1}^{2B_1} + u_{A_5}^{2B_1} u_{\bar{A}_4}^{A_1} u_{\bar{A}_1}^{2A_1} \\
& + u_{A_5}^{2B_1} u_{\bar{A}_4}^{2A_1} u_{\bar{A}_1}^{A_1} + u_{A_3}^{A_1} u_{A_2}^{2A_1} u_{\bar{A}_5}^{2B_1} + u_{A_3}^{A_1} u_{A_2}^{2B_1} u_{\bar{A}_5}^{2A_1} + u_{A_3}^{2A_1} u_{A_2}^{A_1} u_{\bar{A}_5}^{2B_1} + u_{A_3}^{2A_1} u_{A_2}^{2B_1} u_{\bar{A}_5}^{A_1} \\
& + u_{\bar{A}_3}^{2B_1} u_{A_2}^{A_1} u_{\bar{A}_5}^{2A_1} + u_{\bar{A}_3}^{2B_1} u_{A_2}^{2A_1} u_{\bar{A}_5}^{A_1} - u_{A_1}^{A_1} u_{A_4}^{2A_1} u_{\bar{A}_5}^{2B_1} - u_{A_1}^{A_1} u_{A_4}^{2B_1} u_{\bar{A}_5}^{2A_1} - u_{A_1}^{2A_1} u_{A_4}^{A_1} u_{\bar{A}_5}^{2B_1} \\
& - u_{A_1}^{2A_1} u_{A_4}^{2B_1} u_{\bar{A}_5}^{A_1} - u_{A_1}^{2B_1} u_{A_4}^{A_1} u_{\bar{A}_5}^{2A_1} - u_{A_1}^{2B_1} u_{A_4}^{2A_1} u_{\bar{A}_5}^{A_1} ) \\
& + d_{A_5 \bar{A}_4 \bar{A}_1}^{A_1 2A_1 B_2} (u_{A_1}^{A_1} u_{\bar{A}_2}^{2A_1} u_{\bar{A}}^{B_2} - u_{A_1}^{A_1} u_{\bar{A}_2}^{B_2} u_{\bar{A}}^{2A_1} - u_{A_1}^{2A_1} u_{\bar{A}_2}^{A_1} u_{\bar{A}}^{B_2} + u_{A_1}^{2A_1} u_{\bar{A}_2}^{B_2} u_{\bar{A}}^{A_1} + u_{A_1}^{B_2} u_{\bar{A}_2}^{A_1} u_{\bar{A}}^{2A_1} \\
& - u_{A_1}^{B_2} u_{\bar{A}_2}^{2A_1} u_{\bar{A}}^{A_1} + u_{A_3}^{A_1} u_{\bar{A}_4}^{2A_1} u_{\bar{A}}^{B_2} - u_{A_3}^{A_1} u_{\bar{A}_4}^{B_2} u_{\bar{A}}^{2A_1} - u_{A_3}^{2A_1} u_{\bar{A}_4}^{A_1} u_{\bar{A}}^{B_2} + u_{A_3}^{2A_1} u_{\bar{A}_4}^{B_2} u_{\bar{A}}^{A_1} \\
& + u_{A_3}^{B_2} u_{\bar{A}_4}^{A_1} u_{\bar{A}}^{2A_1} - u_{A_3}^{B_2} u_{\bar{A}_4}^{2A_1} u_{\bar{A}}^{A_1} - u_{A_2}^{A_1} u_{\bar{A}}^{B_2} u_{\bar{A}_1}^{2A_1} + u_{A_2}^{A_1} u_{\bar{A}}^{2A_1} u_{\bar{A}_1}^{B_2} + u_{A_2}^{2A_1} u_{\bar{A}}^{B_2} u_{\bar{A}_1}^{A_1} \\
& - u_{A_2}^{2A_1} u_{\bar{A}}^{A_1} u_{\bar{A}_1}^{B_2} - u_{A_2}^{B_2} u_{\bar{A}}^{A_1} u_{\bar{A}_1}^{2A_1} + u_{A_2}^{B_2} u_{\bar{A}}^{A_1} u_{\bar{A}_1}^{2A_1} - u_{A_3}^{2A_1} u_{\bar{A}}^{B_2} u_{\bar{A}_1}^{A_1} + u_{A_3}^{B_2} u_{\bar{A}}^{2A_1} u_{\bar{A}_1}^{A_1} \\
& + u_{A_3}^{A_1} u_{\bar{A}}^{B_2} u_{\bar{A}_4}^{2A_1} - u_{A_3}^{B_2} u_{\bar{A}}^{A_1} u_{\bar{A}_4}^{2A_1} - u_{A_3}^{A_1} u_{\bar{A}}^{2A_1} u_{\bar{A}_4}^{B_2} + u_{A_3}^{2A_1} u_{\bar{A}}^{A_1} u_{\bar{A}_4}^{B_2} + u_{A_3}^{2A_1} u_{\bar{A}_5}^{A_1} u_{\bar{A}_2}^{B_2} \\
& - u_{A_3}^{B_2} u_{\bar{A}_5}^{A_1} u_{\bar{A}_2}^{2A_1} - u_{A_3}^{A_1} u_{\bar{A}_5}^{2A_1} u_{\bar{A}_2}^{B_2} + u_{A_3}^{B_2} u_{\bar{A}_5}^{2A_1} u_{\bar{A}_2}^{A_1} + u_{A_3}^{A_1} u_{\bar{A}_5}^{B_2} u_{\bar{A}_2}^{2A_1} - u_{A_3}^{2A_1} u_{\bar{A}_5}^{B_2} u_{\bar{A}_2}^{A_1} \\
& - u_{A_5}^{A_1} u_{\bar{A}_4}^{2A_1} u_{\bar{A}_1}^{B_2} + u_{A_5}^{A_1} u_{\bar{A}_4}^{B_2} u_{\bar{A}_1}^{2A_1} + u_{A_5}^{2A_1} u_{\bar{A}_4}^{A_1} u_{\bar{A}_1}^{B_2} - u_{A_5}^{2A_1} u_{\bar{A}_4}^{B_2} u_{\bar{A}_1}^{A_1} - u_{A_5}^{B_2} u_{\bar{A}_4}^{A_1} u_{\bar{A}_1}^{2A_1} \\
& + u_{A_5}^{B_2} u_{\bar{A}_4}^{2A_1} u_{\bar{A}_1}^{A_1} + u_{A_3}^{A_1} u_{A_2}^{2A_1} u_{\bar{A}_5}^{B_2} - u_{A_3}^{A_1} u_{A_2}^{B_2} u_{\bar{A}_5}^{2A_1} - u_{A_3}^{2A_1} u_{A_2}^{A_1} u_{\bar{A}_5}^{B_2} + u_{A_3}^{2A_1} u_{A_2}^{B_2} u_{\bar{A}_5}^{A_1} \\
& + u_{A_3}^{B_2} u_{A_2}^{A_1} u_{\bar{A}_5}^{2A_1} - u_{A_3}^{B_2} u_{A_2}^{2A_1} u_{\bar{A}_5}^{A_1} + u_{A_1}^{A_1} u_{A_4}^{2A_1} u_{\bar{A}_5}^{B_2} - u_{A_1}^{A_1} u_{A_4}^{B_2} u_{\bar{A}_5}^{2A_1} - u_{A_1}^{2A_1} u_{A_4}^{A_1} u_{\bar{A}_5}^{B_2} \\
& + u_{A_1}^{2A_1} u_{A_4}^{B_2} u_{\bar{A}_5}^{A_1} + u_{A_1}^{B_2} u_{A_4}^{A_1} u_{\bar{A}_5}^{2A_1} - u_{A_1}^{B_2} u_{A_4}^{2A_1} u_{\bar{A}_5}^{A_1} ) \\
& + d_{A_5 \bar{A}_4 \bar{A}_1}^{A_1 2A_1 {}^1B_2} (u_{A_1}^{A_1} u_{\bar{A}_2}^{2A_1} u_{\bar{A}}^{1B_2} - u_{A_1}^{A_1} u_{\bar{A}_2}^{1B_2} u_{\bar{A}}^{2A_1} - u_{A_1}^{2A_1} u_{\bar{A}_2}^{A_1} u_{\bar{A}}^{1B_2} + u_{A_1}^{2A_1} u_{\bar{A}_2}^{1B_2} u_{\bar{A}}^{A_1} + u_{A_1}^{1B_2} u_{\bar{A}_2}^{A_1} u_{\bar{A}}^{2A_1} \\
& - u_{A_1}^{1B_2} u_{\bar{A}_2}^{2A_1} u_{\bar{A}}^{A_1} + u_{A_3}^{A_1} u_{\bar{A}_4}^{2A_1} u_{\bar{A}}^{1B_2} - u_{A_3}^{A_1} u_{\bar{A}_4}^{1B_2} u_{\bar{A}}^{2A_1} - u_{A_3}^{2A_1} u_{\bar{A}_4}^{A_1} u_{\bar{A}}^{1B_2} + u_{A_3}^{2A_1} u_{\bar{A}_4}^{1B_2} u_{\bar{A}}^{A_1} \\
& + u_{A_3}^{1B_2} u_{\bar{A}_4}^{A_1} u_{\bar{A}}^{2A_1} - u_{A_3}^{1B_2} u_{\bar{A}_4}^{2A_1} u_{\bar{A}}^{A_1} - u_{A_2}^{A_1} u_{\bar{A}}^{1B_2} u_{\bar{A}_1}^{2A_1} + u_{A_2}^{A_1} u_{\bar{A}}^{2A_1} u_{\bar{A}_1}^{1B_2} + u_{A_2}^{2A_1} u_{\bar{A}}^{1B_2} u_{\bar{A}_1}^{A_1} \\
& - u_{A_2}^{2A_1} u_{\bar{A}}^{A_1} u_{\bar{A}_1}^{1B_2} - u_{A_2}^{1B_2} u_{\bar{A}}^{2A_1} u_{\bar{A}_1}^{A_1} + u_{A_2}^{1B_2} u_{\bar{A}}^{A_1} u_{\bar{A}_1}^{2A_1} - u_{A_3}^{2A_1} u_{\bar{A}}^{1B_2} u_{\bar{A}_4}^{A_1} + u_{A_3}^{1B_2} u_{\bar{A}}^{2A_1} u_{\bar{A}_4}^{A_1} \\
& + u_{A_3}^{A_1} u_{\bar{A}}^{1B_2} u_{\bar{A}_4}^{2A_1} - u_{A_3}^{1B_2} u_{\bar{A}}^{A_1} u_{\bar{A}_4}^{2A_1} - u_{A_3}^{A_1} u_{\bar{A}}^{2A_1} u_{\bar{A}_4}^{1B_2} + u_{A_3}^{2A_1} u_{\bar{A}}^{A_1} u_{\bar{A}_4}^{1B$$

[illegible]



30

[illegible]

$$\begin{aligned}
& + u_{\bar{A}_3}^{1B_2} u_{\bar{A}_4}^{A_1} u_{\bar{A}}^{2B_1} - u_{\bar{A}_3}^{1B_2} u_{\bar{A}_4}^{2B_1} u_{\bar{A}}^{A_1} - u_{A_2}^{A_1} u_A^{1B_2} u_{\bar{A}_1}^{2B_1} + u_{A_2}^{A_1} u_A^{2B_1} u_{\bar{A}_1}^{1B_2} + u_{A_2}^{2B_1} u_A^{1B_2} u_{\bar{A}_1}^{A_1} \\
& - u_{A_2}^{2B_1} u_A^{A_1} u_{\bar{A}_1}^{1B_2} - u_{A_2}^{1B_2} u_A^{2B_1} u_{\bar{A}_1}^{A_1} + u_{A_2}^{1B_2} u_A^{A_1} u_{\bar{A}_1}^{2B_1} + u_{A_3}^{2B_1} u_A^{1B_2} u_{\bar{A}_4}^{A_1} - u_{A_3}^{1B_2} u_A^{2B_1} u_{\bar{A}_4}^{A_1} \\
& - u_{A_3}^{A_1} u_A^{1B_2} u_{\bar{A}_4}^{2B_1} + u_{A_3}^{1B_2} u_A^{A_1} u_{\bar{A}_4}^{2B_1} + u_{A_3}^{A_1} u_A^{2B_1} u_{\bar{A}_4}^{1B_2} - u_{A_3}^{2B_1} u_A^{A_1} u_{\bar{A}_4}^{1B_2} + u_{A_3}^{2B_1} u_A^{A_1} u_{\bar{A}_5}^{1B_2} \\
& - u_{A_3}^{1B_2} u_A^{A_1} u_{\bar{A}_5}^{2B_1} - u_{A_3}^{A_1} u_{A_5}^{2B_1} u_{\bar{A}_2}^{1B_2} + u_{A_3}^{1B_2} u_{A_5}^{2B_1} u_{\bar{A}_2}^{A_1} + u_{A_3}^{A_1} u_{A_5}^{1B_2} u_{\bar{A}_2}^{2B_1} - u_{A_3}^{2B_1} u_{A_5}^{1B_2} u_{\bar{A}_2}^{A_1} \\
& + u_{A_5}^{A_1} u_{\bar{A}_4}^{2B_1} u_{\bar{A}_1}^{1B_2} - u_{A_5}^{A_1} u_{\bar{A}_4}^{1B_2} u_{\bar{A}_1}^{2B_1} - u_{A_5}^{2B_1} u_{\bar{A}_4}^{A_1} u_{\bar{A}_1}^{1B_2} + u_{A_5}^{2B_1} u_{\bar{A}_4}^{1B_2} u_{\bar{A}_1}^{A_1} + u_{A_5}^{1B_2} u_{\bar{A}_4}^{A_1} u_{\bar{A}_1}^{2B_1} \\
& - u_{A_5}^{1B_2} u_{\bar{A}_4}^{A_1} u_{\bar{A}_1}^{1B_2} - u_{A_5}^{A_1} u_{A_2}^{2B_1} u_{\bar{A}_5}^{1B_2} + u_{A_5}^{A_1} u_{A_2}^{1B_2} u_{\bar{A}_5}^{2B_1} + u_{\bar{A}_3}^{2B_1} u_{A_2}^{A_1} u_{\bar{A}_5}^{1B_2} - u_{\bar{A}_3}^{2B_1} u_{A_2}^{1B_2} u_{\bar{A}_5}^{A_1} \\
& - u_{\bar{A}_3}^{1B_2} u_{A_2}^{A_1} u_{\bar{A}_5}^{2B_1} + u_{\bar{A}_3}^{1B_2} u_{A_2}^{2B_1} u_{\bar{A}_5}^{A_1} + u_{A_1}^{A_1} u_{A_4}^{2B_1} u_{\bar{A}_5}^{1B_2} - u_{A_1}^{A_1} u_{A_4}^{1B_2} u_{\bar{A}_5}^{2B_1} - u_{A_1}^{2B_1} u_{A_4}^{A_1} u_{\bar{A}_5}^{1B_2} \\
& + u_{A_1}^{2B_1} u_{A_4}^{1B_2} u_{\bar{A}_5}^{A_1} + u_{A_1}^{1B_2} u_{A_4}^{A_1} u_{\bar{A}_5}^{2B_1} - u_{A_1}^{1B_2} u_{A_4}^{2B_1} u_{\bar{A}_5}^{A_1} ) \\
& + d_{A_5 \bar{A}_4 \bar{A}_1}^{A_1 B_2 B_2} (u_{A_1}^{A_1} u_{\bar{A}_2}^{B_2} u_{\bar{A}}^{B_2} + u_{A_1}^{B_2} u_{\bar{A}_2}^{A_1} u_{\bar{A}}^{B_2} + u_{A_1}^{B_2} u_{\bar{A}_2}^{B_2} u_{\bar{A}}^{A_1} + u_{\bar{A}_3}^{A_1} u_{\bar{A}_4}^{B_2} u_{\bar{A}}^{B_2} + u_{\bar{A}_3}^{B_2} u_{\bar{A}_4}^{A_1} u_{\bar{A}}^{B_2} \\
& + u_{\bar{A}_3}^{B_2} u_{\bar{A}_4}^{B_2} u_{\bar{A}}^{A_1} + u_{A_2}^{A_1} u_A^{B_2} u_{\bar{A}_1}^{B_2} + u_{A_2}^{B_2} u_A^{B_2} u_{\bar{A}_1}^{A_1} + u_{A_2}^{B_2} u_A^{A_1} u_{\bar{A}_1}^{B_2} + u_{A_3}^{B_2} u_A^{B_2} u_{\bar{A}_1}^{A_1} \\
& + u_{A_3}^{A_1} u_A^{B_2} u_{\bar{A}_4}^{B_2} + u_{A_3}^{B_2} u_A^{A_1} u_{\bar{A}_4}^{B_2} + u_{A_3}^{B_2} u_A^{B_2} u_{\bar{A}_4}^{A_1} + u_{A_3}^{A_1} u_{A_5}^{B_2} u_{\bar{A}_2}^{B_2} + u_{A_3}^{B_2} u_{A_5}^{B_2} u_{\bar{A}_2}^{A_1} \\
& + u_{A_5}^{A_1} u_{\bar{A}_4}^{B_2} u_{\bar{A}_1}^{B_2} + u_{A_5}^{B_2} u_{\bar{A}_4}^{A_1} u_{\bar{A}_1}^{B_2} + u_{A_5}^{B_2} u_{\bar{A}_4}^{B_2} u_{\bar{A}_1}^{A_1} + u_{\bar{A}_3}^{A_1} u_{A_2}^{B_2} u_{\bar{A}_5}^{B_2} + u_{\bar{A}_3}^{B_2} u_{A_2}^{A_1} u_{\bar{A}_5}^{B_2} \\
& + u_{\bar{A}_3}^{B_2} u_{A_2}^{B_2} u_{\bar{A}_5}^{A_1} + u_{A_1}^{A_1} u_{A_4}^{B_2} u_{\bar{A}_5}^{B_2} + u_{A_1}^{B_2} u_{A_4}^{A_1} u_{\bar{A}_5}^{B_2} + u_{A_1}^{B_2} u_{A_4}^{B_2} u_{\bar{A}_5}^{A_1} ) \\
& + d_{A_5 \bar{A}_4 \bar{A}_1}^{A_1 B_2 1B_2} (u_{A_1}^{A_1} u_{\bar{A}_2}^{B_2} u_{\bar{A}}^{1B_2} + u_{A_1}^{A_1} u_{\bar{A}_2}^{1B_2} u_{\bar{A}}^{B_2} + u_{A_1}^{B_2} u_{\bar{A}_2}^{A_1} u_{\bar{A}}^{1B_2} + u_{A_1}^{B_2} u_{\bar{A}_2}^{B_2} u_{\bar{A}}^{A_1} + u_{A_1}^{1B_2} u_{\bar{A}_2}^{A_1} u_{\bar{A}}^{B_2} \\
& + u_{A_1}^{1B_2} u_{\bar{A}_2}^{B_2} u_{\bar{A}}^{A_1} + u_{\bar{A}_3}^{A_1} u_{\bar{A}_4}^{B_2} u_{\bar{A}}^{1B_2} + u_{\bar{A}_3}^{A_1} u_{\bar{A}_4}^{1B_2} u_{\bar{A}}^{B_2} + u_{\bar{A}_3}^{B_2} u_{\bar{A}_4}^{A_1} u_{\bar{A}}^{1B_2} + u_{\bar{A}_3}^{B_2} u_{\bar{A}_4}^{B_2} u_{\bar{A}}^{A_1} \\
& + u_{\bar{A}_3}^{1B_2} u_{\bar{A}_4}^{A_1} u_{\bar{A}}^{B_2} + u_{\bar{A}_3}^{1B_2} u_{\bar{A}_4}^{B_2} u_{\bar{A}}^{A_1} + u_{A_2}^{A_1} u_A^{1B_2} u_{\bar{A}_1}^{B_2} + u_{A_2}^{A_1} u_A^{B_2} u_{\bar{A}_1}^{1B_2} + u_{A_2}^{B_2} u_A^{1B_2} u_{\bar{A}_1}^{A_1} \\
& + u_{A_2}^{B_2} u_A^{A_1} u_{\bar{A}_1}^{1B_2} + u_{A_2}^{1B_2} u_A^{B_2} u_{\bar{A}_1}^{A_1} + u_{A_2}^{1B_2} u_A^{A_1} u_{\bar{A}_1}^{B_2} + u_{A_3}^{B_2} u_A^{1B_2} u_{\bar{A}_4}^{A_1} + u_{A_3}^{1B_2} u_A^{B_2} u_{\bar{A}_4}^{A_1} \\
& + u_{A_3}^{A_1} u_A^{1B_2} u_{\bar{A}_4}^{B_2} + u_{A_3}^{1B_2} u_A^{A_1} u_{\bar{A}_4}^{B_2} + u_{A_3}^{A_1} u_A^{B_2} u_{\bar{A}_4}^{1B_2} + u_{A_3}^{B_2} u_A^{A_1} u_{\bar{A}_4}^{1B_2} + u_{A_3}^{B_2} u_{A_5}^{A_1} u_{\bar{A}_2}^{1B_2} \\
& + u_{A_3}^{1B_2} u_{A_5}^{A_1} u_{\bar{A}_2}^{B_2} + u_{A_3}^{A_1} u_{A_5}^{B_2} u_{\bar{A}_2}^{1B_2} + u_{A_3}^{1B_2} u_{A_5}^{B_2} u_{\bar{A}_2}^{A_1} + u_{A_3}^{A_1} u_{A_5}^{1B_2} u_{\bar{A}_2}^{B_2} + u_{A_3}^{B_2} u_{A_5}^{1B_2} u_{\bar{A}_2}^{A_1} \\
& + u_{A_5}^{A_1} u_{\bar{A}_4}^{B_2} u_{\bar{A}_1}^{1B_2} + u_{A_5}^{A_1} u_{\bar{A}_4}^{1B_2} u_{\bar{A}_1}^{B_2} + u_{A_5}^{B_2} u_{\bar{A}_4}^{A_1} u_{\bar{A}_1}^{1B_2} + u_{A_5}^{B_2} u_{\bar{A}_4}^{B_2} u_{\bar{A}_1}^{A_1} + u_{A_5}^{1B_2} u_{\bar{A}_4}^{A_1} u_{\bar{A}_1}^{B_2} \\
& + u_{A_5}^{1B_2} u_{\bar{A}_4}^{B_2} u_{\bar{A}_1}^{A_1} + u_{\bar{A}_3}^{A_1} u_{A_2}^{1B_2} u_{\bar{A}_5}^{B_2} + u_{\bar{A}_3}^{A_1} u_{A_2}^{B_2} u_{\bar{A}_5}^{1B_2} + u_{\bar{A}_3}^{B_2} u_{A_2}^{A_1} u_{\bar{A}_5}^{1B_2} + u_{\bar{A}_3}^{B_2} u_{A_2}^{B_2} u_{\bar{A}_5}^{A_1} \\
& + u_{\bar{A}_3}^{1B_2} u_{A_2}^{A_1} u_{\bar{A}_5}^{B_2} + u_{\bar{A}_3}^{1B_2} u_{A_2}^{B_2} u_{\bar{A}_5}^{A_1} + u_{A_1}^{A_1} u_{A_4}^{B_2} u_{\bar{A}_5}^{1B_2} + u_{A_1}^{A_1} u_{A_4}^{1B_2} u_{\bar{A}_5}^{B_2} + u_{A_1}^{B_2} u_{A_4}^{A_1} u_{\bar{A}_5}^{1B_2} \\
& + u_{A_1}^{B_2} u_{A_4}^{B_2} u_{\bar{A}_5}^{A_1} + u_{A_1}^{1B_2} u_{A_4}^{A_1} u_{\bar{A}_5}^{B_2} + u_{A_1}^{1B_2} u_{A_4}^{B_2} u_{\bar{A}_5}^{A_1} ) \\
& + d_{A_5 \bar{A}_4 \bar{A}_1}^{A_1 1B_2 1B_2} (u_{A_1}^{A_1} u_{\bar{A}_2}^{1B_2} u_{\bar{A}}^{1B_2} + u_{A_1}^{1B_2} u_{\bar{A}_2}^{A_1} u_{\bar{A}}^{1B_2} + u_{A_1}^{1B_2} u_{\bar{A}_2}^{1B_2} u_{\bar{A}}^{A_1} + u_{\bar{A}_3}^{A_1} u_{\bar{A}_4}^{1B_2} u_{\bar{A}}^{1B_2} + u_{\bar{A}_3}^{1B_2} u_{\bar{A}_4}^{A_1} u_{\bar{A}}^{1B_2} \\
& + u_{\bar{A}_3}^{1B_2} u_{\bar{A}_4}^{B_2} u_{\bar{A}}^{A_1} + u_{A_2}^{A_1} u_A^{1B_2} u_{\bar{A}_1}^{1B_2} + u_{A_2}^{A_1} u_A^{1B_2} u_{\bar{A}_1}^{A_1} + u_{A_2}^{1B_2} u_A^{A_1} u_{\bar{A}_1}^{1B_2} + u_{A_2}^{1B_2} u_A^{A_1} u_{\bar{A}_1}^{A_1} \\
& + u_{A_3}^{A_1} u_A^{1B_2} u_{\bar{A}_4}^{1B_2} + u_{A_3}^{1B_2} u_A^{A_1} u_{\bar{A}_4}^{1B_2} + u_{A_3}^{1B_2} u_A^{A_1} u_{\bar{A}_4}^{A_1} + u_{A_3}^{A_1} u_{A_5}^{1B_2} u_{\bar{A}_2}^{1B_2} + u_{A_3}^{1B_2} u_{A_5}^{A_1} u_{\bar{A}_2}^{1B_2} \\
& + u_{A_5}^{A_1} u_{\bar{A}_4}^{1B_2} u_{\bar{A}_1}^{1B_2} + u_{A_5}^{1B_2} u_{\bar{A}_4}^{A_1} u_{\bar{A}_1}^{1B_2} + u_{A_5}^{1B_2} u_{\bar{A}_4}^{1B_2} u_{\bar{A}_1}^{A_1} + u_{\bar{A}_3}^{A_1} u_{A_2}^{1B_2} u_{\bar{A}_5}^{1B_2} + u_{\bar{A}_3}^{1B_2} u_{A_2}^{A_1} u_{\bar{A}_5}^{1B_2} \\
& + u_{\bar{A}_3}^{1B_2} u_{A_2}^{B_2} u_{\bar{A}_5}^{A_1} + u_{A_1}^{1B_2} u_{A_4}^{A_1} u_{\bar{A}_5}^{1B_2} + u_{A_1}^{1B_2} u_{A_4}^{1B_2} u_{\bar{A}_5}^{A_1} + u_{A_1}^{A_1} u_{A_4}^{1B_2} u_{\bar{A}_5}^{1B_2} ) \\
& + d_{A_5 \bar{A}_4 \bar{A}_1}^{1A_1 1A_1 1A_1} (u_{A_1}^{1A_1} u_{\bar{A}_2}^{1A_1} u_{\bar{A}}^{1A_1} + u_{\bar{A}_3}^{1A_1} u_{\bar{A}_4}^{1A_1} u_{\bar{A}}^{1A_1} + u_{A_2}^{1A_1} u_A^{1A_1} u_{\bar{A}_1}^{1A_1} + u_{A_3}^{1A_1} u_A^{1A_1} u_{\bar{A}_4}^{1A_1} + u_{A_3}^{1A_1} u_{A_5}^{1A_1} u_{\bar{A}_2}^{1A_1} \\
& + u_{A_5}^{1A_1} u_{\bar{A}_4}^{1A_1} u_{\bar{A}_1}^{1A_1} + u_{\bar{A}_3}^{1A_1} u_{A_2}^{1A_1} u_{\bar{A}_5}^{1A_1} + u_{A_1}^{1A_1} u_{A_4}^{1A_1} u_{\bar{A}_5}^{1A_1} ) \\
& + d_{A_5 \bar{A}_4 \bar{A}_1}^{1A_1 1A_1 2A_1} (u_{A_1}^{1A_1} u_{\bar{A}_2}^{1A_1} u_{\bar{A}}^{2A_1} + u_{A_1}^{1A_1} u_{\bar{A}_2}^{2A_1} u_{\bar{A}}^{1A_1} + u_{A_1}^{2A_1} u_{\bar{A}_2}^{1A_1} u_{\bar{A}}^{1A_1} + u_{\bar{A}_3}^{1A_1} u_{\bar{A}_4}^{1A_1} u_{\bar{A}}^{2A_1} + u_{\bar{A}_3}^{1A_1} u_{\bar{A}_4}^{2A_1} u_{\bar{A}}^{1A_1} \\
& + u_{\bar{A}_3}^{2A_1} u_{\bar{A}_4}^{1A_1} u_{\bar{A}}^{1A_1} + u_{A_2}^{1A_1} u_A^{1A_1} u_{\bar{A}_1}^{1A_1} + u_{A_2}^{1A_1} u_A^{1A_1} u_{\bar{A}_1}^{2A_1} + u_{A_2}^{2A_1} u_A^{1A_1} u_{\bar{A}_1}^{1A_1} + u_{A_3}^{2A_1} u_A^{1A_1} u_{\bar{A}_4}^{1A_1} \\
& + u_{A_3}^{2A_1} u_A^{1A_1} u_{\bar{A}_4}^{1A_1} + u_{A_3}^{1A_1} u_A^{1A_1} u_{\bar{A}_4}^{2A_1} + u_{A_3}^{1A_1} u_{A_5}^{1A_1} u_{\bar{A}_2}^{2A_1} + u_{A_3}^{2A_1} u_{A_5}^{1A_1} u_{\bar{A}_2}^{1A_1} + u_{A_3}^{1A_1} u_{A_5}^{2A_1} u_{\bar{A}_2}^{1A_1} \\
& + u_{A_5}^{1A_1} u_{\bar{A}_4}^{1A_1} u_{\bar{A}_1}^{2A_1} + u_{A_5}^{1A_1} u_{\bar{A}_4}^{2A_1} u_{\bar{A}_1}^{1A_1} + u_{A_5}^{2A_1} u_{\bar{A}_4}^{1A_1} u_{\bar{A}_1}^{1A_1} + u_{\bar{A}_3}^{1A_1} u_{A_2}^{1A_1} u_{\bar{A}_5}^{2A_1} + u_{\bar{A}_3}^{1A_1} u_{A_2}^{2A_1} u_{\bar{A}_5}^{1A_1} \\
& + u_{\bar{A}_3}^{2A_1} u_{A_2}^{1A_1} u_{\bar{A}_5}^{1A_1} + u_{A_1}^{1A_1} u_{A_4}^{1A_1} u_{\bar{A}_5}^{2A_1} + u_{A_1}^{1A_1} u_{A_4}^{2A_1} u_{\bar{A}_5}^{1A_1} + u_{A_1}^{2A_1} u_{A_4}^{1A_1} u_{\bar{A}_5}^{1A_1} )
\end{aligned}$$



[illegible]

[illegible]







[illegible]

[illegible]





[illegible]









$$+ u_{A_5}^{^2 A_1} u_{\bar{A}_4}^{^1 B_2} u_{\bar{A}_1}^{^1 B_2} + u_{A_5}^{^1 B_2} u_{\bar{A}_4}^{^2 A_1} u_{\bar{A}_1}^{^1 B_2} + u_{A_5}^{^1 B_2} u_{\bar{A}_4}^{^1 B_2} u_{\bar{A}_1}^{^2 A_1} + u_{A_3}^{^2 A_1} u_{A_2}^{^1 B_2} u_{A_5}^{^1 B_2} + u_{A_3}^{^1 B_2} u_{A_2}^{^2 A_1} u_{A_5}^{^1 B_2}) \\ + d_{A_5 \bar{A}_4 \bar{A}_1}^{A_2 A_2 B_1} (u_{A_1}^{A_2} u_{A_2}^{A_2} u_{\bar{A}}^{B_1} + u_{A_1}^{A_2} u_{A_2}^{B_1} u_{\bar{A}}^{A_2} + u_{A_1}^{B_1} u_{A_2}^{A_2} u_{\bar{A}}^{A_2} - u_{A_3}^{A_2} u_{A_4}^{A_2} u_{\bar{A}}^{B_1} - u_{A_3}^{A_2} u_{A_4}^{B_1} u_{\bar{A}}^{A_2} \\ - u_{A_3}^{B_1} u_{A_4}^{A_2} u_{\bar{A}}^{A_2} - u_{A_2}^{A_2} u_A^{B_1} u_{\bar{A}}^{A_2} - u_{A_2}^{A_2} u_A^{A_2} u_{\bar{A}}^{B_1} - u_{A_2}^{B_1} u_A^{A_2} u_{\bar{A}}^{A_2} + u_{A_3}^{A_2} u_A^{B_1} u_{A_4}^{A_2} \\ + u_{A_3}^{B_1} u_A^{A_2} u_{A_4}^{A_2} + u_{A_3}^{A_2} u_A^{A_2} u_{A_4}^{B_1} - u_{A_3}^{A_2} u_{A_5}^{A_2} u_{\bar{A}}^{B_1} - u_{A_3}^{B_1} u_{A_5}^{A_2} u_{\bar{A}}^{A_2} - u_{A_3}^{A_2} u_{A_5}^{B_1} u_{\bar{A}}^{A_2} \\ + u_{A_5}^{A_2} u_{\bar{A}_4}^{A_2} u_{\bar{A}_1}^{B_1} + u_{A_5}^{A_2} u_{\bar{A}_4}^{B_1} u_{\bar{A}_1}^{A_2} + u_{A_5}^{B_1} u_{\bar{A}_4}^{A_2} u_{\bar{A}_1}^{A_2} + u_{A_3}^{A_2} u_{A_2}^{A_2} u_{A_5}^{B_1} + u_{A_3}^{A_2} u_{A_2}^{B_1} u_{A_5}^{A_2} \\ + u_{A_3}^{B_1} u_{A_2}^{A_2} u_{A_5}^{A_2} - u_{A_1}^{A_2} u_{A_4}^{A_2} u_{A_5}^{B_1} - u_{A_1}^{A_2} u_{A_4}^{B_1} u_{A_5}^{A_2} - u_{A_1}^{B_1} u_{A_4}^{A_2} u_{A_5}^{A_2}) \\ + d_{A_5 \bar{A}_4 \bar{A}_1}^{A_2 A_2 {}^2 B_1} (u_{A_1}^{A_2} u_{A_2}^{A_2} u_{\bar{A}}^{^2 B_1} + u_{A_1}^{A_2} u_{A_2}^{^2 B_1} u_{\bar{A}}^{A_2} + u_{A_1}^{^2 B_1} u_{A_2}^{A_2} u_{\bar{A}}^{A_2} - u_{A_3}^{A_2} u_{A_4}^{A_2} u_{\bar{A}}^{^2 B_1} - u_{A_3}^{A_2} u_{A_4}^{^2 B_1} u_{\bar{A}}^{A_2} \\ - u_{A_3}^{^2 B_1} u_{A_4}^{A_2} u_{\bar{A}}^{A_2} - u_{A_2}^{A_2} u_A^{^2 B_1} u_{\bar{A}}^{A_2} - u_{A_2}^{A_2} u_A^{A_2} u_{\bar{A}}^{^2 B_1} - u_{A_2}^{^2 B_1} u_A^{A_2} u_{\bar{A}}^{A_2} + u_{A_3}^{A_2} u_A^{^2 B_1} u_{A_4}^{A_2} \\ + u_{A_3}^{^2 B_1} u_A^{A_2} u_{A_4}^{A_2} + u_{A_3}^{A_2} u_A^{A_2} u_{A_4}^{^2 B_1} - u_{A_3}^{A_2} u_{A_5}^{A_2} u_{\bar{A}}^{^2 B_1} - u_{A_3}^{^2 B_1} u_{A_5}^{A_2} u_{\bar{A}}^{A_2} - u_{A_3}^{A_2} u_{A_5}^{^2 B_1} u_{\bar{A}}^{A_2} \\ + u_{A_5}^{A_2} u_{\bar{A}_4}^{A_2} u_{\bar{A}_1}^{^2 B_1} + u_{A_5}^{A_2} u_{\bar{A}_4}^{^2 B_1} u_{\bar{A}_1}^{A_2} + u_{A_5}^{^2 B_1} u_{\bar{A}_4}^{A_2} u_{\bar{A}_1}^{A_2} + u_{A_3}^{A_2} u_{A_2}^{A_2} u_{A_5}^{^2 B_1} + u_{A_3}^{A_2} u_{A_2}^{^2 B_1} u_{A_5}^{A_2} \\ + u_{A_3}^{^2 B_1} u_{A_2}^{A_2} u_{A_5}^{A_2} - u_{A_1}^{A_2} u_{A_4}^{A_2} u_{A_5}^{^2 B_1} - u_{A_1}^{A_2} u_{A_4}^{^2 B_1} u_{A_5}^{A_2} - u_{A_1}^{^2 B_1} u_{A_4}^{A_2} u_{A_5}^{A_2}) \\ + d_{A_5 \bar{A}_4 \bar{A}_1}^{A_2 B_1 {}^1 B_1} (u_{A_1}^{A_2} u_{A_2}^{B_1} u_{\bar{A}}^{^1 B_1} - u_{A_1}^{A_2} u_{A_2}^{^1 B_1} u_{\bar{A}}^{B_1} - u_{A_1}^{B_1} u_{A_2}^{A_2} u_{\bar{A}}^{^1 B_1} + u_{A_1}^{B_1} u_{A_2}^{^1 B_1} u_{\bar{A}}^{A_2} + u_{A_1}^{^1 B_1} u_{A_2}^{A_2} u_{\bar{A}}^{B_1} \\ - u_{A_1}^{^1 B_1} u_{A_2}^{B_1} u_{\bar{A}}^{A_2} - u_{A_3}^{A_2} u_{A_4}^{B_1} u_{\bar{A}}^{^1 B_1} + u_{A_3}^{A_2} u_{A_4}^{^1 B_1} u_{\bar{A}}^{B_1} + u_{A_3}^{B_1} u_{A_4}^{A_2} u_{\bar{A}}^{^1 B_1} - u_{A_3}^{B_1} u_{A_4}^{^1 B_1} u_{\bar{A}}^{A_2} \\ - u_{A_3}^{^1 B_1} u_{A_4}^{A_2} u_{\bar{A}}^{B_1} + u_{A_3}^{^1 B_1} u_{A_4}^{B_1} u_{\bar{A}}^{A_2} + u_{A_2}^{A_2} u_A^{^1 B_1} u_{\bar{A}}^{B_1} - u_{A_2}^{A_2} u_A^{B_1} u_{\bar{A}}^{^1 B_1} - u_{A_2}^{B_1} u_A^{^1 B_1} u_{\bar{A}}^{A_2} \\ + u_{A_2}^{B_1} u_A^{A_2} u_{\bar{A}}^{^1 B_1} + u_{A_2}^{^1 B_1} u_A^{B_1} u_{\bar{A}}^{A_2} - u_{A_2}^{A_2} u_{A_4}^{B_1} u_{\bar{A}}^{^1 B_1} - u_{A_3}^{A_2} u_{A_4}^{^1 B_1} u_{\bar{A}}^{A_2} + u_{A_3}^{^1 B_1} u_{A_4}^{B_1} u_{\bar{A}}^{A_2} \\ + u_{A_3}^{A_2} u_A^{^1 B_1} u_{A_4}^{B_1} - u_{A_3}^{^1 B_1} u_A^{A_2} u_{A_4}^{B_1} - u_{A_3}^{A_2} u_{A_4}^{B_1} u_{A_5}^{^1 B_1} + u_{A_3}^{B_1} u_A^{A_2} u_{A_4}^{^1 B_1} - u_{A_3}^{B_1} u_{A_5}^{A_2} u_{\bar{A}}^{^1 B_1} \\ + u_{A_3}^{^1 B_1} u_{A_5}^{A_2} u_{\bar{A}}^{A_2} + u_{A_3}^{A_2} u_{A_5}^{^1 B_1} u_{\bar{A}}^{B_1} - u_{A_3}^{^1 B_1} u_{A_5}^{B_1} u_{\bar{A}}^{A_2} - u_{A_3}^{A_2} u_{A_5}^{B_1} u_{\bar{A}}^{A_2} + u_{A_3}^{B_1} u_{A_5}^{^1 B_1} u_{\bar{A}}^{A_2} \\ - u_{A_5}^{A_2} u_{\bar{A}_4}^{B_1} u_{\bar{A}_1}^{^1 B_1} + u_{A_5}^{A_2} u_{\bar{A}_4}^{^1 B_1} u_{\bar{A}_1}^{B_1} + u_{A_5}^{B_1} u_{\bar{A}_4}^{A_2} u_{\bar{A}_1}^{^1 B_1} - u_{A_5}^{B_1} u_{\bar{A}_4}^{^1 B_1} u_{\bar{A}_1}^{A_2} - u_{A_5}^{^1 B_1} u_{\bar{A}_4}^{A_2} u_{\bar{A}_1}^{B_1} \\ + u_{A_5}^{^1 B_1} u_{\bar{A}_4}^{B_1} u_{\bar{A}_1}^{A_2} + u_{A_3}^{A_2} u_{A_2}^{B_1} u_{A_5}^{^1 B_1} - u_{A_3}^{A_2} u_{A_2}^{^1 B_1} u_{A_5}^{B_1} - u_{A_3}^{B_1} u_{A_2}^{A_2} u_{A_5}^{^1 B_1} + u_{A_3}^{B_1} u_{A_2}^{^1 B_1} u_{A_5}^{A_2} \\ + u_{A_3}^{^1 B_1} u_{A_2}^{A_2} u_{A_5}^{B_1} - u_{A_3}^{^1 B_1} u_{A_2}^{B_1} u_{A_5}^{A_2} - u_{A_1}^{A_2} u_{A_4}^{B_1} u_{A_5}^{^1 B_1} + u_{A_1}^{A_2} u_{A_4}^{^1 B_1} u_{A_5}^{B_1} + u_{A_1}^{B_1} u_{A_4}^{A_2} u_{A_5}^{^1 B_1} \\ - u_{A_1}^{B_1} u_{A_4}^{^1 B_1} u_{A_5}^{A_2} - u_{A_1}^{^1 B_1} u_{A_4}^{A_2} u_{A_5}^{B_1} + u_{A_1}^{^1 B_1} u_{A_4}^{B_1} u_{A_5}^{A_2}) \\ + d_{A_5 \bar{A}_4 \bar{A}_1}^{A_2 B_1 {}^2 B_1} (u_{A_1}^{A_2} u_{A_2}^{B_1} u_{\bar{A}}^{^2 B_1} - u_{A_1}^{A_2} u_{A_2}^{^2 B_1} u_{\bar{A}}^{B_1} - u_{A_1}^{B_1} u_{A_2}^{A_2} u_{\bar{A}}^{^2 B_1} + u_{A_1}^{B_1} u_{A_2}^{^2 B_1} u_{\bar{A}}^{A_2} + u_{A_1}^{^2 B_1} u_{A_2}^{A_2} u_{\bar{A}}^{B_1} \\ - u_{A_1}^{^2 B_1} u_{A_2}^{B_1} u_{\bar{A}}^{A_2} - u_{A_3}^{A_2} u_{A_4}^{B_1} u_{\bar{A}}^{^2 B_1} + u_{A_3}^{A_2} u_{$$



[illegible]



$$\begin{aligned}
& + u_{A_1}^{2B_1} u_{A_4}^{1B_2} u_{A_5}^{A_2} + u_{A_1}^{1B_2} u_{A_4}^{A_2} u_{A_5}^{2B_1} + u_{A_1}^{1B_2} u_{A_4}^{2B_1} u_{A_5}^{A_2} ) \\
& + d_{A_5 A_4 A_1}^{A_2 B_2 1B_2} (u_{A_1}^{A_2} u_{A_2}^{B_2} u_{A_5}^{1B_2} - u_{A_1}^{A_2} u_{A_2}^{1B_2} u_{A_5}^{B_2} - u_{A_1}^{B_2} u_{A_2}^{A_2} u_{A_5}^{1B_2} + u_{A_1}^{B_2} u_{A_2}^{A_2} u_{A_5}^{B_2} + u_{A_1}^{1B_2} u_{A_2}^{A_2} u_{A_5}^{B_2} \\
& - u_{A_1}^{1B_2} u_{A_2}^{B_2} u_{A_5}^{A_2} - u_{A_3}^{A_2} u_{A_4}^{B_2} u_{A_5}^{1B_2} + u_{A_3}^{A_2} u_{A_4}^{1B_2} u_{A_5}^{B_2} + u_{A_3}^{B_2} u_{A_4}^{A_2} u_{A_5}^{1B_2} - u_{A_3}^{B_2} u_{A_4}^{A_2} u_{A_5}^{B_2} \\
& - u_{A_3}^{1B_2} u_{A_4}^{A_2} u_{A_5}^{B_2} + u_{A_3}^{1B_2} u_{A_4}^{B_2} u_{A_5}^{A_2} + u_{A_2}^{A_2} u_{A_4}^{1B_2} u_{A_5}^{B_2} - u_{A_2}^{A_2} u_{A_4}^{B_2} u_{A_5}^{1B_2} - u_{A_2}^{B_2} u_{A_4}^{1B_2} u_{A_5}^{A_2} \\
& + u_{A_2}^{B_2} u_{A_4}^{A_2} u_{A_5}^{1B_2} + u_{A_2}^{1B_2} u_{A_4}^{A_2} u_{A_5}^{B_2} - u_{A_2}^{1B_2} u_{A_4}^{B_2} u_{A_5}^{A_2} - u_{A_3}^{B_2} u_{A_4}^{1B_2} u_{A_5}^{A_2} + u_{A_3}^{1B_2} u_{A_4}^{B_2} u_{A_5}^{A_2} \\
& + u_{A_3}^{A_2} u_{A_4}^{1B_2} u_{A_5}^{B_2} - u_{A_3}^{1B_2} u_{A_4}^{A_2} u_{A_5}^{B_2} - u_{A_3}^{A_2} u_{A_4}^{B_2} u_{A_5}^{1B_2} + u_{A_3}^{B_2} u_{A_4}^{A_2} u_{A_5}^{1B_2} - u_{A_3}^{B_2} u_{A_4}^{A_2} u_{A_5}^{1B_2} \\
& + u_{A_3}^{1B_2} u_{A_4}^{A_2} u_{A_5}^{B_2} + u_{A_3}^{A_2} u_{A_4}^{B_2} u_{A_5}^{1B_2} - u_{A_3}^{1B_2} u_{A_4}^{B_2} u_{A_5}^{A_2} - u_{A_3}^{A_2} u_{A_4}^{1B_2} u_{A_5}^{B_2} + u_{A_3}^{B_2} u_{A_4}^{1B_2} u_{A_5}^{A_2} \\
& - u_{A_5}^{A_2} u_{A_4}^{B_2} u_{A_1}^{1B_2} + u_{A_5}^{A_2} u_{A_4}^{1B_2} u_{A_1}^{B_2} + u_{A_5}^{B_2} u_{A_4}^{A_2} u_{A_1}^{1B_2} - u_{A_5}^{B_2} u_{A_4}^{A_2} u_{A_1}^{B_2} - u_{A_5}^{1B_2} u_{A_4}^{A_2} u_{A_1}^{B_2} \\
& + u_{A_5}^{1B_2} u_{A_4}^{B_2} u_{A_1}^{A_2} + u_{A_3}^{A_2} u_{A_2}^{B_2} u_{A_5}^{1B_2} - u_{A_3}^{A_2} u_{A_2}^{1B_2} u_{A_5}^{B_2} - u_{A_3}^{B_2} u_{A_2}^{A_2} u_{A_5}^{1B_2} + u_{A_3}^{B_2} u_{A_2}^{A_2} u_{A_5}^{B_2} \\
& + u_{A_3}^{1B_2} u_{A_2}^{A_2} u_{A_5}^{B_2} - u_{A_3}^{1B_2} u_{A_2}^{B_2} u_{A_5}^{A_2} - u_{A_1}^{A_2} u_{A_4}^{B_2} u_{A_5}^{1B_2} + u_{A_1}^{A_2} u_{A_4}^{1B_2} u_{A_5}^{B_2} + u_{A_1}^{B_2} u_{A_4}^{A_2} u_{A_5}^{1B_2} \\
& - u_{A_1}^{B_2} u_{A_4}^{A_2} u_{A_5}^{B_2} - u_{A_1}^{1B_2} u_{A_4}^{A_2} u_{A_5}^{B_2} + u_{A_1}^{1B_2} u_{A_4}^{B_2} u_{A_5}^{A_2} ) \\
& + d_{A_5 A_4 A_1}^{B_1 B_1 B_1} (u_{A_1}^{B_1} u_{A_2}^{B_1} u_{A_5}^{B_1} - u_{A_3}^{B_1} u_{A_4}^{B_1} u_{A_5}^{B_1} - u_{A_2}^{B_1} u_{A_4}^{B_1} u_{A_5}^{B_1} + u_{A_3}^{B_1} u_{A_4}^{B_1} u_{A_5}^{B_1} - u_{A_3}^{B_1} u_{A_5}^{B_1} u_{A_2}^{B_1} \\
& + u_{A_5}^{B_1} u_{A_4}^{B_1} u_{A_1}^{B_1} + u_{A_3}^{B_1} u_{A_2}^{B_1} u_{A_5}^{B_1} - u_{A_1}^{B_1} u_{A_4}^{B_1} u_{A_5}^{B_1} ) \\
& + d_{A_5 A_4 A_1}^{B_1 B_1 1B_1} (u_{A_1}^{B_1} u_{A_2}^{B_1} u_{A_5}^{1B_1} + u_{A_1}^{B_1} u_{A_2}^{1B_1} u_{A_5}^{B_1} + u_{A_1}^{1B_1} u_{A_2}^{B_1} u_{A_5}^{B_1} - u_{A_3}^{B_1} u_{A_4}^{B_1} u_{A_5}^{1B_1} - u_{A_3}^{B_1} u_{A_4}^{1B_1} u_{A_5}^{B_1} \\
& - u_{A_3}^{1B_1} u_{A_4}^{B_1} u_{A_5}^{B_1} - u_{A_2}^{B_1} u_{A_4}^{1B_1} u_{A_5}^{B_1} - u_{A_2}^{B_1} u_{A_4}^{B_1} u_{A_5}^{1B_1} - u_{A_2}^{1B_1} u_{A_4}^{B_1} u_{A_5}^{B_1} + u_{A_3}^{B_1} u_{A_4}^{1B_1} u_{A_5}^{B_1} \\
& + u_{A_3}^{1B_1} u_{A_4}^{B_1} u_{A_5}^{B_1} + u_{A_3}^{B_1} u_{A_4}^{B_1} u_{A_5}^{1B_1} - u_{A_3}^{B_1} u_{A_5}^{B_1} u_{A_2}^{1B_1} - u_{A_3}^{B_1} u_{A_5}^{1B_1} u_{A_2}^{B_1} - u_{A_3}^{1B_1} u_{A_5}^{B_1} u_{A_2}^{B_1} \\
& + u_{A_5}^{B_1} u_{A_4}^{B_1} u_{A_1}^{1B_1} + u_{A_5}^{B_1} u_{A_4}^{1B_1} u_{A_1}^{B_1} + u_{A_5}^{1B_1} u_{A_4}^{B_1} u_{A_1}^{B_1} + u_{A_5}^{1B_1} u_{A_4}^{1B_1} u_{A_1}^{B_1} + u_{A_3}^{B_1} u_{A_2}^{B_1} u_{A_5}^{1B_1} + u_{A_3}^{B_1} u_{A_2}^{1B_1} u_{A_5}^{B_1} \\
& + u_{A_3}^{1B_1} u_{A_2}^{B_1} u_{A_5}^{B_1} - u_{A_1}^{B_1} u_{A_4}^{B_1} u_{A_5}^{1B_1} - u_{A_1}^{B_1} u_{A_4}^{1B_1} u_{A_5}^{B_1} - u_{A_1}^{1B_1} u_{A_4}^{B_1} u_{A_5}^{B_1} - u_{A_1}^{1B_1} u_{A_4}^{B_1} u_{A_5}^{1B_1} ) \\
& + d_{A_5 A_4 A_1}^{B_1 B_1 2B_1} (u_{A_1}^{B_1} u_{A_2}^{B_1} u_{A_5}^{2B_1} + u_{A_1}^{B_1} u_{A_2}^{2B_1} u_{A_5}^{B_1} + u_{A_1}^{2B_1} u_{A_2}^{B_1} u_{A_5}^{B_1} - u_{A_3}^{B_1} u_{A_4}^{B_1} u_{A_5}^{2B_1} - u_{A_3}^{B_1} u_{A_4}^{2B_1} u_{A_5}^{B_1} \\
& - u_{A_3}^{2B_1} u_{A_4}^{B_1} u_{A_5}^{B_1} - u_{A_2}^{B_1} u_{A_4}^{2B_1} u_{A_5}^{B_1} - u_{A_2}^{B_1} u_{A_4}^{B_1} u_{A_5}^{2B_1} + u_{A_3}^{B_1} u_{A_4}^{B_1} u_{A_5}^{2B_1} + u_{A_3}^{B_1} u_{A_4}^{2B_1} u_{A_5}^{B_1} \\
& + u_{A_3}^{2B_1} u_{A_4}^{B_1} u_{A_5}^{B_1} + u_{A_5}^{B_1} u_{A_4}^{2B_1} u_{A_1}^{B_1} + u_{A_5}^{B_1} u_{A_4}^{B_1} u_{A_1}^{2B_1} + u_{A_5}^{2B_1} u_{A_4}^{B_1} u_{A_1}^{B_1} + u_{A_5}^{2B_1} u_{A_4}^{B_1} u_{A_1}^{2B_1} + u_{A_3}^{B_1} u_{A_2}^{B_1} u_{A_5}^{1B_1} \\
& + u_{A_3}^{B_1} u_{A_2}^{1B_1} u_{A_5}^{B_1} - u_{A_1}^{B_1} u_{A_4}^{B_1} u_{A_5}^{2B_1} - u_{A_1}^{B_1} u_{A_4}^{2B_1} u_{A_5}^{B_1} - u_{A_1}^{2B_1} u_{A_4}^{B_1} u_{A_5}^{B_1} - u_{A_1}^{2B_1} u_{A_4}^{B_1} u_{A_5}^{1B_1} ) \\
& + d_{A_5 A_4 A_1}^{B_1 1B_1 1B_1} (u_{A_1}^{B_1} u_{A_2}^{1B_1} u_{A_5}^{1B_1} + u_{A_1}^{B_1} u_{A_2}^{1B_1} u_{A_5}^{B_1} + u_{A_1}^{1B_1} u_{A_2}^{B_1} u_{A_5}^{B_1} - u_{A_3}^{B_1} u_{A_4}^{B_1} u_{A_5}^{1B_1} - u_{A_3}^{B_1} u$$



[illegible]

[illegible]



[illegible]

55





57

58



[illegible]

[illegible]



























[illegible]









[illegible]

79

$$\begin{aligned}
& + u_{\bar{A}4}^{B_1} u_A^{2B_1} u_{A_1}^{1B_1} - u_{\bar{A}4}^{2B_1} u_A^{B_1} u_{A_1}^{1B_1} - u_{\bar{A}4}^{B_1} u_A^{1B_1} u_{A_1}^{2B_1} + u_{\bar{A}4}^{1B_1} u_A^{B_1} u_{A_1}^{2B_1} - u_{\bar{A}1}^{B_1} u_{\bar{A}2}^{2B_1} u_{\bar{A}5}^{B_1} \\
& + u_{\bar{A}1}^{2B_1} u_{\bar{A}2}^{1B_1} u_{\bar{A}5}^{B_1} + u_{\bar{A}1}^{B_1} u_{\bar{A}2}^{2B_1} u_{\bar{A}5}^{1B_1} - u_{\bar{A}1}^{2B_1} u_{\bar{A}2}^{B_1} u_{\bar{A}5}^{1B_1} - u_{\bar{A}1}^{B_1} u_{\bar{A}2}^{1B_1} u_{\bar{A}5}^{2B_1} + u_{\bar{A}1}^{1B_1} u_{\bar{A}2}^{B_1} u_{\bar{A}5}^{2B_1} \\
& + u_{\bar{A}3}^{1B_1} u_{\bar{A}4}^{2B_1} u_{\bar{A}5}^{B_1} - u_{\bar{A}3}^{2B_1} u_{\bar{A}4}^{1B_1} u_{\bar{A}5}^{B_1} - u_{\bar{A}3}^{B_1} u_{\bar{A}4}^{2B_1} u_{\bar{A}5}^{1B_1} + u_{\bar{A}3}^{2B_1} u_{\bar{A}4}^{B_1} u_{\bar{A}5}^{1B_1} + u_{\bar{A}3}^{B_1} u_{\bar{A}4}^{1B_1} u_{\bar{A}5}^{2B_1} \\
& - u_{\bar{A}3}^{1B_1} u_{\bar{A}4}^{B_1} u_{\bar{A}5}^{2B_1} + u_{\bar{A}2}^{1B_1} u_{\bar{A}5}^{2B_1} u_{\bar{A}1}^{B_1} - u_{\bar{A}2}^{2B_1} u_{\bar{A}5}^{1B_1} u_{\bar{A}1}^{B_1} - u_{\bar{A}2}^{B_1} u_{\bar{A}5}^{2B_1} u_{\bar{A}1}^{1B_1} + u_{\bar{A}2}^{2B_1} u_{\bar{A}5}^{B_1} u_{\bar{A}1}^{1B_1} \\
& + u_{\bar{A}2}^{B_1} u_{\bar{A}5}^{1B_1} u_{\bar{A}1}^{2B_1} - u_{\bar{A}2}^{1B_1} u_{\bar{A}5}^{B_1} u_{\bar{A}1}^{2B_1} + u_{\bar{A}3}^{1B_1} u_{\bar{A}5}^{2B_1} u_{\bar{A}4}^{B_1} - u_{\bar{A}3}^{2B_1} u_{\bar{A}5}^{1B_1} u_{\bar{A}4}^{B_1} - u_{\bar{A}3}^{B_1} u_{\bar{A}5}^{2B_1} u_{\bar{A}4}^{1B_1} \\
& + u_{\bar{A}3}^{2B_1} u_{\bar{A}5}^{B_1} u_{\bar{A}4}^{1B_1} + u_{\bar{A}3}^{B_1} u_{\bar{A}5}^{1B_1} u_{\bar{A}4}^{2B_1} - u_{\bar{A}3}^{1B_1} u_{\bar{A}5}^{B_1} u_{\bar{A}4}^{2B_1} ) \\
& + d_{\bar{A}1\bar{A}2\bar{A}5}^{B_2B_11B_1} (u_{\bar{A}1}^{1B_1} u_{\bar{A}}^{B_2} u_{\bar{A}4}^{B_1} - u_{\bar{A}1}^{B_2} u_{\bar{A}}^{1B_1} u_{\bar{A}4}^{B_1} - u_{\bar{A}1}^{B_1} u_{\bar{A}}^{B_2} u_{\bar{A}4}^{1B_1} + u_{\bar{A}1}^{B_2} u_{\bar{A}}^{B_1} u_{\bar{A}4}^{1B_1} + u_{\bar{A}1}^{B_1} u_{\bar{A}}^{1B_1} u_{\bar{A}4}^{B_2} \\
& - u_{\bar{A}1}^{1B_1} u_{\bar{A}}^{B_1} u_{\bar{A}4}^{B_2} + u_{\bar{A}3}^{1B_1} u_{\bar{A}2}^{B_1} u_{\bar{A}}^{B_2} - u_{\bar{A}3}^{B_2} u_{\bar{A}2}^{B_1} u_{\bar{A}}^{1B_1} - u_{\bar{A}3}^{B_1} u_{\bar{A}2}^{1B_1} u_{\bar{A}}^{B_2} + u_{\bar{A}3}^{B_2} u_{\bar{A}2}^{1B_1} u_{\bar{A}}^{B_1} \\
& + u_{\bar{A}3}^{B_1} u_{\bar{A}2}^{B_2} u_{\bar{A}}^{1B_1} - u_{\bar{A}3}^{1B_1} u_{\bar{A}2}^{B_2} u_{\bar{A}}^{B_1} - u_{\bar{A}3}^{B_1} u_{\bar{A}}^{B_2} u_{\bar{A}2}^{1B_1} + u_{\bar{A}3}^{B_2} u_{\bar{A}}^{1B_1} u_{\bar{A}2}^{B_2} + u_{\bar{A}3}^{1B_1} u_{\bar{A}}^{B_2} u_{\bar{A}2}^{B_1} \\
& - u_{\bar{A}3}^{1B_1} u_{\bar{A}}^{B_1} u_{\bar{A}2}^{B_2} - u_{\bar{A}3}^{B_2} u_{\bar{A}}^{1B_1} u_{\bar{A}2}^{B_1} + u_{\bar{A}3}^{B_2} u_{\bar{A}}^{B_1} u_{\bar{A}2}^{1B_1} - u_{\bar{A}3}^{1B_1} u_{\bar{A}}^{B_2} u_{\bar{A}2}^{B_1} + u_{\bar{A}3}^{B_2} u_{\bar{A}}^{B_1} u_{\bar{A}2}^{B_1} \\
& + u_{\bar{A}4}^{B_1} u_{\bar{A}}^{B_2} u_{\bar{A}1}^{1B_1} - u_{\bar{A}4}^{B_2} u_{\bar{A}}^{B_1} u_{\bar{A}1}^{1B_1} - u_{\bar{A}4}^{B_1} u_{\bar{A}}^{1B_1} u_{\bar{A}1}^{B_2} + u_{\bar{A}4}^{1B_1} u_{\bar{A}}^{B_1} u_{\bar{A}1}^{B_2} - u_{\bar{A}4}^{1B_1} u_{\bar{A}}^{B_2} u_{\bar{A}1}^{B_1} \\
& + u_{\bar{A}1}^{B_2} u_{\bar{A}2}^{1B_1} u_{\bar{A}5}^{B_1} + u_{\bar{A}1}^{B_1} u_{\bar{A}2}^{B_2} u_{\bar{A}5}^{1B_1} - u_{\bar{A}1}^{B_2} u_{\bar{A}2}^{B_1} u_{\bar{A}5}^{1B_1} - u_{\bar{A}1}^{B_1} u_{\bar{A}2}^{1B_1} u_{\bar{A}5}^{B_2} + u_{\bar{A}1}^{1B_1} u_{\bar{A}2}^{B_1} u_{\bar{A}5}^{B_2} \\
& - u_{\bar{A}3}^{1B_1} u_{\bar{A}4}^{B_2} u_{\bar{A}5}^{B_1} + u_{\bar{A}3}^{B_2} u_{\bar{A}4}^{1B_1} u_{\bar{A}5}^{B_1} + u_{\bar{A}3}^{B_1} u_{\bar{A}4}^{B_2} u_{\bar{A}5}^{1B_1} - u_{\bar{A}3}^{B_2} u_{\bar{A}4}^{B_1} u_{\bar{A}5}^{1B_1} - u_{\bar{A}3}^{B_1} u_{\bar{A}4}^{1B_1} u_{\bar{A}5}^{B_2} \\
& + u_{\bar{A}3}^{1B_1} u_{\bar{A}4}^{B_1} u_{\bar{A}5}^{B_2} - u_{\bar{A}2}^{1B_1} u_{\bar{A}5}^{B_2} u_{\bar{A}1}^{B_1} + u_{\bar{A}2}^{B_2} u_{\bar{A}5}^{B_1} u_{\bar{A}1}^{1B_1} + u_{\bar{A}2}^{B_2} u_{\bar{A}5}^{1B_1} u_{\bar{A}1}^{B_1} - u_{\bar{A}2}^{B_1} u_{\bar{A}5}^{B_2} u_{\bar{A}1}^{1B_1} \\
& - u_{\bar{A}2}^{B_1} u_{\bar{A}5}^{1B_1} u_{\bar{A}1}^{B_2} + u_{\bar{A}2}^{1B_1} u_{\bar{A}5}^{B_2} u_{\bar{A}1}^{B_2} + u_{\bar{A}3}^{1B_1} u_{\bar{A}5}^{B_2} u_{\bar{A}4}^{B_1} - u_{\bar{A}3}^{B_2} u_{\bar{A}5}^{1B_1} u_{\bar{A}4}^{B_1} - u_{\bar{A}3}^{B_1} u_{\bar{A}5}^{B_2} u_{\bar{A}4}^{1B_1} \\
& + u_{\bar{A}3}^{B_2} u_{\bar{A}5}^{B_1} u_{\bar{A}4}^{1B_1} + u_{\bar{A}3}^{B_1} u_{\bar{A}5}^{1B_1} u_{\bar{A}4}^{B_2} - u_{\bar{A}3}^{1B_1} u_{\bar{A}5}^{B_2} u_{\bar{A}4}^{B_2} ) \\
& + d_{\bar{A}1\bar{A}2\bar{A}5}^{1B_2B_11B_1} (u_{\bar{A}1}^{1B_1} u_{\bar{A}}^{1B_2} u_{\bar{A}4}^{B_1} - u_{\bar{A}1}^{1B_2} u_{\bar{A}}^{1B_1} u_{\bar{A}4}^{B_1} - u_{\bar{A}1}^{B_1} u_{\bar{A}}^{1B_2} u_{\bar{A}4}^{1B_1} + u_{\bar{A}1}^{1B_2} u_{\bar{A}}^{B_1} u_{\bar{A}4}^{1B_1} + u_{\bar{A}1}^{B_1} u_{\bar{A}}^{1B_1} u_{\bar{A}4}^{1B_2} \\
& - u_{\bar{A}1}^{1B_1} u_{\bar{A}}^{B_1} u_{\bar{A}4}^{1B_2} + u_{\bar{A}3}^{1B_1} u_{\bar{A}2}^{B_1} u_{\bar{A}}^{1B_2} - u_{\bar{A}3}^{1B_2} u_{\bar{A}2}^{B_1} u_{\bar{A}}^{1B_1} - u_{\bar{A}3}^{B_1} u_{\bar{A}2}^{1B_1} u_{\bar{A}}^{1B_2} + u_{\bar{A}3}^{1B_2} u_{\bar{A}2}^{1B_1} u_{\bar{A}}^{B_1} \\
& + u_{\bar{A}3}^{B_1} u_{\bar{A}2}^{1B_2} u_{\bar{A}}^{1B_1} - u_{\bar{A}3}^{1B_1} u_{\bar{A}2}^{1B_2} u_{\bar{A}}^{B_1} - u_{\bar{A}3}^{B_1} u_{\bar{A}}^{1B_2} u_{\bar{A}2}^{1B_1} + u_{\bar{A}3}^{1B_2} u_{\bar{A}}^{1B_1} u_{\bar{A}2}^{B_2} + u_{\bar{A}3}^{1B_1} u_{\bar{A}}^{1B_2} u_{\bar{A}2}^{B_1} \\
& - u_{\bar{A}3$$





[illegible]

$$\begin{aligned}
& + u_X^{A_{1g}} u_{\bar{A}_2}^{A_1} u_{A_4}^{2A_1} + u_{\bar{A}_3}^{A_1} u_{\bar{A}_1}^{2A_1} u_X^{A_{1g}} + u_{\bar{A}_3}^{2A_1} u_{\bar{A}_1}^{A_1} u_X^{A_{1g}} + u_{A_2}^{A_1} u_{\bar{A}_4}^{2A_1} u_X^{A_{1g}} + u_{A_2}^{2A_1} u_{\bar{A}_4}^{A_1} u_X^{A_{1g}} \\
& + u_{A_3}^{2A_1} u_X^{A_{1g}} u_{A_1}^{A_1} + u_{A_3}^{A_1} u_X^{A_{1g}} u_{A_1}^{2A_1} + u_{A_5}^{A_1} u_A^{2A_1} u_{X_2}^{A_{1g}} + u_{A_5}^{2A_1} u_A^{A_1} u_{X_2}^{A_{1g}} + u_{X_1}^{A_{1g}} u_A^{2A_1} u_{\bar{A}_5}^{A_1} \\
& + u_{X_1}^{A_{1g}} u_A^{A_1} u_{\bar{A}_5}^{2A_1} + u_{X_1}^{A_{1g}} u_{\bar{A}_4}^{A_1} u_{\bar{A}_2}^{2A_1} + u_{X_1}^{A_{1g}} u_{\bar{A}_4}^{2A_1} u_{\bar{A}_2}^{A_1} + u_{A_3}^{A_{1g}} u_{X_2}^{2A_1} u_{\bar{A}_1}^{A_1} + u_{A_3}^{2A_1} u_{X_2}^{A_{1g}} u_{\bar{A}_1}^{A_1} \\
& + u_{\bar{A}_3}^{2A_1} u_{X_2}^{A_{1g}} u_{A_1}^{A_1} + u_{\bar{A}_3}^{A_1} u_{X_2}^{A_{1g}} u_{A_1}^{2A_1} + u_{X_1}^{A_{1g}} u_{A_2}^{2A_1} u_{A_4}^{A_1} + u_{X_1}^{A_{1g}} u_{A_2}^{A_1} u_{A_4}^{2A_1}) \\
& + d_{A_3 X_2 \bar{A}_1}^{A_1 A_{1g} B_2} (-u_{X_2}^{A_{1g}} u_{\bar{A}}^{B_2} u_{\bar{A}_5}^{A_1} - u_{X_2}^{A_{1g}} u_{\bar{A}}^{A_1} u_{A_5}^{B_2} + u_{X_1}^{A_{1g}} u_{A_5}^{A_1} u_{\bar{A}}^{B_2} + u_{X_1}^{A_{1g}} u_{A_5}^{B_2} u_{\bar{A}}^{A_1} + u_X^{A_{1g}} u_{\bar{A}_2}^{B_2} u_{A_4}^{A_1} \\
& + u_X^{A_{1g}} u_{\bar{A}_2}^{A_1} u_{A_4}^{B_2} - u_{\bar{A}_3}^{A_1} u_{\bar{A}_1}^{B_2} u_X^{A_{1g}} - u_{\bar{A}_3}^{B_2} u_{\bar{A}_1}^{A_1} u_X^{A_{1g}} + u_{A_2}^{A_1} u_{\bar{A}_4}^{B_2} u_X^{A_{1g}} + u_{A_2}^{B_2} u_{\bar{A}_4}^{A_1} u_X^{A_{1g}} \\
& - u_{A_3}^{B_2} u_X^{A_{1g}} u_{A_1}^{A_1} - u_{A_3}^{A_1} u_X^{A_{1g}} u_{A_1}^{B_2} - u_{A_5}^{A_1} u_A^{B_2} u_{X_2}^{A_{1g}} - u_{A_5}^{B_2} u_A^{A_1} u_{X_2}^{A_{1g}} + u_{X_1}^{A_{1g}} u_A^{B_2} u_{\bar{A}_5}^{A_1} \\
& + u_{X_1}^{A_{1g}} u_A^{A_1} u_{\bar{A}_5}^{B_2} - u_{X_1}^{A_{1g}} u_{\bar{A}_4}^{A_1} u_{\bar{A}_2}^{B_2} - u_{X_1}^{A_{1g}} u_{\bar{A}_4}^{B_2} u_{\bar{A}_2}^{A_1} + u_{A_3}^{A_{1g}} u_{X_2}^{B_2} u_{\bar{A}_1}^{A_1} + u_{A_3}^{B_2} u_{X_2}^{A_{1g}} u_{\bar{A}_1}^{A_1} \\
& + u_{\bar{A}_3}^{B_2} u_{X_2}^{A_{1g}} u_{A_1}^{A_1} + u_{\bar{A}_3}^{A_1} u_{X_2}^{A_{1g}} u_{A_1}^{B_2} - u_{X_1}^{A_{1g}} u_{A_2}^{B_2} u_{A_4}^{A_1} - u_{X_1}^{A_{1g}} u_{A_2}^{A_1} u_{A_4}^{B_2}) \\
& + d_{A_3 X_2 \bar{A}_1}^{A_1 A_{1g} {}^1B_2} (-u_{X_2}^{A_{1g}} u_{\bar{A}}^{1B_2} u_{\bar{A}_5}^{A_1} - u_{X_2}^{A_{1g}} u_{\bar{A}}^{A_1} u_{\bar{A}_5}^{1B_2} + u_{X_1}^{A_{1g}} u_{A_5}^{A_1} u_{\bar{A}}^{1B_2} + u_{X_1}^{A_{1g}} u_{A_5}^{1B_2} u_{\bar{A}}^{A_1} + u_X^{A_{1g}} u_{\bar{A}_2}^{1B_2} u_{A_4}^{A_1} \\
& + u_X^{A_{1g}} u_{\bar{A}_2}^{A_1} u_{A_4}^{1B_2} - u_{\bar{A}_3}^{A_1} u_{\bar{A}_1}^{1B_2} u_X^{A_{1g}} - u_{\bar{A}_3}^{1B_2} u_{\bar{A}_1}^{A_1} u_X^{A_{1g}} + u_{A_2}^{A_1} u_{\bar{A}_4}^{1B_2} u_X^{A_{1g}} + u_{A_2}^{1B_2} u_{\bar{A}_4}^{A_1} u_X^{A_{1g}} \\
& - u_{A_3}^{1B_2} u_X^{A_{1g}} u_{A_1}^{A_1} - u_{A_3}^{A_1} u_X^{A_{1g}} u_{A_1}^{1B_2} - u_{A_5}^{A_1} u_A^{1B_2} u_{X_2}^{A_{1g}} - u_{A_5}^{1B_2} u_A^{A_1} u_{X_2}^{A_{1g}} + u_{X_1}^{A_{1g}} u_A^{1B_2} u_{\bar{A}_5}^{A_1} \\
& + u_{X_1}^{A_{1g}} u_A^{A_1} u_{\bar{A}_5}^{1B_2} - u_{X_1}^{A_{1g}} u_{\bar{A}_4}^{A_1} u_{\bar{A}_2}^{1B_2} - u_{X_1}^{A_{1g}} u_{\bar{A}_4}^{1B_2} u_{\bar{A}_2}^{A_1} + u_{A_3}^{A_{1g}} u_{X_2}^{1B_2} u_{\bar{A}_1}^{A_1} + u_{A_3}^{1B_2} u_{X_2}^{A_{1g}} u_{\bar{A}_1}^{A_1} \\
& + u_{\bar{A}_3}^{1B_2} u_{X_2}^{A_{1g}} u_{A_1}^{A_1} + u_{\bar{A}_3}^{A_1} u_{X_2}^{A_{1g}} u_{A_1}^{1B_2} - u_{X_1}^{A_{1g}} u_{A_2}^{1B_2} u_{A_4}^{A_1} - u_{X_1}^{A_{1g}} u_{A_2}^{A_1} u_{A_4}^{1B_2}) \\
& + d_{A_3 X_2 \bar{A}_1}^{A_1 E_g A_2} (u_{X_2}^{E_g(0)} u_{\bar{A}}^{A_2} u_{\bar{A}_5}^{A_1} - u_{X_2}^{E_g(0)} u_{\bar{A}}^{A_1} u_{\bar{A}_5}^{A_2} - u_{X_1}^{E_g(0)} u_{A_5}^{A_1} u_{\bar{A}}^{A_2} + u_{X_1}^{E_g(0)} u_{A_5}^{A_2} u_{\bar{A}}^{A_1} + u_X^{E_g(0)} u_{\bar{A}_2}^{A_2} u_{A_4}^{A_1} \\
& - u_X^{E_g(0)} u_{\bar{A}_2}^{A_1} u_{A_4}^{A_2} + u_{\bar{A}_3}^{A_1} u_{\bar{A}_1}^{A_2} u_X^{E_g(1)} - u_{\bar{A}_3}^{A_2} u_{\bar{A}_1}^{A_1} u_X^{E_g(1)} + u_{A_2}^{A_1} u_{\bar{A}_4}^{A_2} u_X^{E_g(0)} - u_{A_2}^{A_2} u_{\bar{A}_4}^{A_1} u_X^{E_g(0)} \\
& + u_{A_3}^{A_2} u_X^{E_g(1)} u_{A_1}^{A_1} - u_{A_3}^{A_1} u_X^{E_g(1)} u_{A_1}^{A_2} - u_{A_5}^{A_1} u_A^{A_2} u_{X_2}^{E_g(0)} + u_{A_5}^{A_2} u_A^{A_1} u_{X_2}^{E_g(0)} + u_{X_1}^{E_g(0)} u_A^{A_2} u_{\bar{A}_5}^{A_1} \\
& - u_{X_1}^{E_g(0)} u_A^{A_1} u_{\bar{A}_5}^{A_2} - u_{X_1}^{E_g(1)} u_{\bar{A}_4}^{A_1} u_{\bar{A}_2}^{A_2} + u_{X_1}^{E_g(1)} u_{\bar{A}_4}^{A_2} u_{\bar{A}_2}^{A_1} + u_{A_3}^{A_1} u_{X_2}^{E_g(1)} u_{\bar{A}_1}^{A_2} - u_{A_3}^{A_2} u_{X_2}^{E_g(1)} u_{\bar{A}_1}^{A_1} \\
& + u_{\bar{A}_3}^{A_2} u_{X_2}^{E_g(1)} u_{A_1}^{A_1} - u_{\bar{A}_3}^{A_1} u_{X_2}^{E_g(1)} u_{A_1}^{A_2} + u_{X_1}^{E_g(1)} u_{A_2}^{A_2} u_{A_4}^{A_1} - u_{X_1}^{E_g(1)} u_{A_2}^{A_1} u_{A_4}^{A_2}) \\
& + d_{A_3 X_2 \bar{A}_1}^{A_1 E_g B_1} (u_{X_2}^{E_g(0)} u_{\bar{A}}^{B_1} u_{\bar{A}_5}^{A_1} - u_{X_2}^{E_g(0)} u_{\bar{A}}^{A_1} u_{\bar{A}_5}^{B_1} + u_{X_1}^{E_g(0)} u_{A_5}^{A_1} u_{\bar{A}}^{B_1} - u_{X_1}^{E_g(0)} u_{A_5}^{B_1} u_{\bar{A}}^{A_1} - u_X^{E_g(0)} u_{\bar{A}_2}^{B_1} u_{A_4}^{A_1} \\
& + u_X^{E_g(0)} u_{\bar{A}_2}^{A_1} u_{A_4}^{B_1} + u_{\bar{A}_3}^{A_1} u_{\bar{A}_1}^{B_1} u_X^{E_g(1)} - u_{\bar{A}_3}^{B_1} u_{\bar{A}_1}^{A_1} u_X^{E_g(1)} - u_{A_2}^{A_1} u_{\bar{A}_4}^{B_1} u_X^{E_g(0)} + u_{A_2}^{B_1} u_{\bar{A}_4}^{A_1} u_X^{E_g(0)} \\
& + u_{A_3}^{B_1} u_X^{E_g(1)} u_{A_1}^{A_1} - u_{A_3}^{A_1} u_X^{E_g(1)} u_{A_1}^{B_1} - u_{A_5}^{A_1} u_A^{B_1} u_{X_2}^{E_g(0)} + u_{A_5}^{B_1} u_A^{A_1} u_{X_2}^{E_g(0)} - u_{X_1}^{E_g(0)} u_A^{B_1} u_{\bar{A}_5}^{A_1} \\
& + u_{X_1}^{E_g(0)} u_A^{A_1} u_{\bar{A}_5}^{B_1} - u_{X_1}^{E_g(1)} u_{\bar{A}_4}^{A_1} u_{\bar{A}_2}^{B_1} + u_{X_1}$$

[illegible]



$$\begin{aligned}
& + u_{A_3}^{2A_1} u_X^{E_u^{(1)}} u_{A_1}^{A_1} - u_{A_3}^{E_u^{(1)}} u_X^{A_1} u_{A_1}^{2A_1} - u_{A_5}^{2A_1} u_A^{E_u^{(0)}} u_{X_2}^{A_1} + u_{A_5}^{A_1} u_A^{E_u^{(0)}} u_{X_2}^{2A_1} + u_{X_1}^{E_u^{(0)}} u_A^{2A_1} u_{A_5}^{A_1} \\
& - u_{X_1}^{E_u^{(0)}} u_A^{A_1} u_{A_5}^{2A_1} - u_{X_1}^{E_u^{(1)}} u_A^{A_1} u_{A_4}^{2A_1} + u_{X_1}^{E_u^{(1)}} u_{A_4}^{2A_1} u_{A_2}^{A_1} + u_{A_3}^{A_1} u_{X_2}^{E_u^{(1)}} u_{A_1}^{2A_1} - u_{A_3}^{2A_1} u_{X_2}^{E_u^{(1)}} u_{A_1}^{A_1} \\
& + u_{A_3}^{2A_1} u_{X_2}^{E_u^{(1)}} u_{A_1}^{A_1} - u_{A_3}^{A_1} u_{X_2}^{E_u^{(1)}} u_{A_1}^{2A_1} + u_{X_1}^{E_u^{(1)}} u_{A_2}^{2A_1} u_{A_4}^{A_1} - u_{X_1}^{E_u^{(1)}} u_{A_2}^{A_1} u_{A_4}^{2A_1} ) \\
& + d_{A_3 X_2 \bar{A}_1}^{A_1 E_u B_2} (u_{X_2}^{E_u^{(0)}} u_{\bar{A}}^{B_2} u_{A_5}^{A_1} - u_{X_2}^{E_u^{(0)}} u_{\bar{A}}^{A_1} u_{A_5}^{B_2} + u_{X_1}^{E_u^{(0)}} u_{A_5}^{A_1} u_{\bar{A}}^{B_2} - u_{X_1}^{E_u^{(0)}} u_{A_5}^{B_2} u_{\bar{A}}^{A_1} - u_X^{E_u^{(0)}} u_{A_2}^{B_2} u_{A_4}^{A_1} \\
& + u_X^{E_u^{(0)}} u_{A_2}^{A_1} u_{A_4}^{B_2} + u_{A_3}^{A_1} u_{A_1}^{B_2} u_X^{E_u^{(1)}} - u_{A_3}^{B_2} u_{A_1}^{A_1} u_X^{E_u^{(1)}} - u_{A_2}^{A_1} u_{A_4}^{B_2} u_X^{E_u^{(0)}} + u_{A_2}^{B_2} u_{A_4}^{A_1} u_X^{E_u^{(0)}} \\
& + u_{A_3}^{B_2} u_X^{E_u^{(1)}} u_{A_1}^{A_1} - u_{A_3}^{A_1} u_X^{E_u^{(1)}} u_{A_1}^{B_2} - u_{A_5}^{A_1} u_A^{B_2} u_{X_2}^{E_u^{(0)}} + u_{A_5}^{B_2} u_A^{A_1} u_{X_2}^{E_u^{(0)}} - u_{X_1}^{E_u^{(0)}} u_{A_3}^{B_2} u_{A_5}^{A_1} \\
& + u_{X_1}^{E_u^{(0)}} u_A^{A_1} u_{A_5}^{B_2} - u_{X_1}^{E_u^{(1)}} u_A^{A_1} u_{A_2}^{B_2} + u_{X_1}^{E_u^{(1)}} u_{A_4}^{B_2} u_{A_2}^{A_1} - u_{A_3}^{A_1} u_{X_2}^{E_u^{(1)}} u_{A_1}^{B_2} + u_{A_3}^{B_2} u_{X_2}^{E_u^{(1)}} u_{A_1}^{A_1} \\
& - u_{A_3}^{B_2} u_{X_2}^{E_u^{(1)}} u_{A_1}^{A_1} + u_{A_3}^{A_1} u_{X_2}^{E_u^{(1)}} u_{A_1}^{B_2} + u_{X_1}^{E_u^{(1)}} u_{A_2}^{B_2} u_{A_4}^{A_1} - u_{X_1}^{E_u^{(1)}} u_{A_2}^{A_1} u_{A_4}^{B_2} ) \\
& + d_{A_3 X_2 \bar{A}_1}^{A_1 E_u {}^1B_2} (u_{X_2}^{E_u^{(0)}} u_{\bar{A}}^{^1B_2} u_{A_5}^{A_1} - u_{X_2}^{E_u^{(0)}} u_{\bar{A}}^{A_1} u_{A_5}^{^1B_2} + u_{X_1}^{E_u^{(0)}} u_{A_5}^{A_1} u_{\bar{A}}^{^1B_2} - u_{X_1}^{E_u^{(0)}} u_{A_5}^{^1B_2} u_{\bar{A}}^{A_1} - u_X^{E_u^{(0)}} u_{A_2}^{^1B_2} u_{A_4}^{A_1} \\
& + u_X^{E_u^{(0)}} u_{A_2}^{A_1} u_{A_4}^{^1B_2} + u_{A_3}^{A_1} u_{A_1}^{^1B_2} u_X^{E_u^{(1)}} - u_{A_3}^{^1B_2} u_{A_1}^{A_1} u_X^{E_u^{(1)}} - u_{A_2}^{A_1} u_{A_4}^{^1B_2} u_X^{E_u^{(0)}} + u_{A_2}^{^1B_2} u_{A_4}^{A_1} u_X^{E_u^{(0)}} \\
& + u_{A_3}^{^1B_2} u_X^{E_u^{(1)}} u_{A_1}^{A_1} - u_{A_3}^{A_1} u_X^{E_u^{(1)}} u_{A_1}^{^1B_2} - u_{A_5}^{A_1} u_A^{^1B_2} u_{X_2}^{E_u^{(0)}} + u_{A_5}^{^1B_2} u_A^{A_1} u_{X_2}^{E_u^{(0)}} - u_{X_1}^{E_u^{(0)}} u_{A_3}^{^1B_2} u_{A_5}^{A_1} \\
& + u_{X_1}^{E_u^{(0)}} u_A^{A_1} u_{A_5}^{^1B_2} - u_{X_1}^{E_u^{(1)}} u_{A_4}^{^1B_2} u_{A_2}^{A_1} + u_{X_1}^{E_u^{(1)}} u_{A_4}^{A_1} u_{A_2}^{^1B_2} - u_{A_3}^{A_1} u_{X_2}^{E_u^{(1)}} u_{A_1}^{^1B_2} + u_{A_3}^{^1B_2} u_{X_2}^{E_u^{(1)}} u_{A_1}^{A_1} \\
& - u_{A_3}^{^1B_2} u_{X_2}^{E_u^{(1)}} u_{A_1}^{A_1} + u_{A_3}^{A_1} u_{X_2}^{E_u^{(1)}} u_{A_1}^{^1B_2} + u_{X_1}^{E_u^{(1)}} u_{A_2}^{^1B_2} u_{A_4}^{A_1} - u_{X_1}^{E_u^{(1)}} u_{A_2}^{A_1} u_{A_4}^{^1B_2} ) \\
& + d_{A_3 X_2 \bar{A}_1}^{A_1 E_u A_2} (-u_{X_2}^{E_u^{(1)}} u_{\bar{A}}^{A_2} u_{A_5}^{A_1} + u_{X_2}^{E_u^{(1)}} u_{\bar{A}}^{A_1} u_{A_5}^{A_2} + u_{X_1}^{E_u^{(1)}} u_{A_5}^{A_1} u_{\bar{A}}^{A_2} - u_{X_1}^{E_u^{(1)}} u_{A_5}^{A_2} u_{\bar{A}}^{A_1} + u_X^{E_u^{(1)}} u_{A_2}^{A_2} u_{A_4}^{A_1} \\
& - u_X^{E_u^{(1)}} u_{A_2}^{A_1} u_{A_4}^{A_2} + u_{A_3}^{A_1} u_{A_1}^{A_2} u_X^{E_u^{(0)}} - u_{A_3}^{A_2} u_{A_1}^{A_1} u_X^{E_u^{(0)}} - u_{A_2}^{A_1} u_{A_4}^{A_2} u_X^{E_u^{(1)}} + u_{A_2}^{A_2} u_{A_4}^{A_1} u_X^{E_u^{(1)}} \\
& - u_{A_3}^{A_2} u_X^{E_u^{(0)}} u_{A_1}^{A_1} + u_{A_3}^{A_1} u_X^{E_u^{(0)}} u_{A_1}^{A_2} - u_{A_5}^{A_1} u_A^{A_2} u_{X_2}^{E_u^{(1)}} + u_{A_5}^{A_2} u_A^{A_1} u_{X_2}^{E_u^{(1)}} + u_{X_1}^{E_u^{(1)}} u_A^{A_2} u_{A_5}^{A_1} \\
& - u_{X_1}^{E_u^{(1)}} u_A^{A_1} u_{A_5}^{A_2} - u_{X_1}^{E_u^{(0)}} u_{A_4}^{A_1} u_{A_2}^{A_2} + u_{X_1}^{E_u^{(0)}} u_{A_4}^{A_2} u_{A_2}^{A_1} - u_{A_3}^{A_1} u_{X_2}^{E_u^{(0)}} u_{A_1}^{A_2} + u_{A_3}^{A_2} u_{X_2}^{E_u^{(0)}} u_{A_1}^{A_1} \\
& + u_{A_3}^{A_2} u_{X_2}^{E_u^{(0)}} u_{A_1}^{A_1} - u_{A_3}^{A_1} u_{X_2}^{E_u^{(0)}} u_{A_1}^{A_2} - u_{X_1}^{E_u^{(0)}} u_{A_2}^{A_2} u_{A_4}^{A_1} + u_{X_1}^{E_u^{(0)}} u_{A_2}^{A_1} u_{A_4}^{A_2} ) \\
& + d_{A_3 X_2 \bar{A}_1}^{A_1 E_u B_1} (-u_{X_2}^{E_u^{(1)}} u_{\bar{A}}^{B_1} u_{A_5}^{A_1} + u_{X_2}^{E_u^{(1)}} u_{\bar{A}}^{A_1} u_{A_5}^{B_1} - u_{X_1}^{E_u^{(1)}} u_{A_5}^{A_1} u_{\bar{A}}^{B_1} + u_{X_1}^{E_u^{(1)}} u_{A_5}^{B_1} u_{\bar{A}}^{A_1} - u_X^{E_u^{(1)}} u_{A_2}^{B_1} u_{A_4}^{A_1} \\
& + u_X^{E_u^{(1)}} u_{A_2}^{A_1} u_{A_4}^{B_1} + u_{A_3}^{A_1} u_{A_1}^{B_1} u_X^{E_u^{(0)}} - u_{A_3}^{B_1} u_{A_1}^{A_1} u_X^{E_u^{(0)}} + u_{A_2}^{A_1} u_{A_4}^{B_1} u_X^{E_u^{(1)}} - u_{A_2}^{B_1} u_{A_4}^{A_1} u_X^{E_u^{(1)}} \\
& - u_{A_3}^{B_1} u_X^{E_u^{(0)}} u_{A_1}^{A_1} + u_{A_3}^{A_1} u_X^{E_u^{(0)}} u_{A_1}^{B_1} - u_{A_5}^{A_1} u_A^{B_1} u_{X_2}^{E_u^{(1)}} + u_{A_5}^{B_1} u_A^{A_1} u_{X_2}^{E_u^{(1)}} - u_{X_1}^{E_u^{(1)}} u_A^{B_1} u_{A_5}^{A_1} \\
& + u_{X_1}^{E_u^{(1)}} u_A^{A_1} u_{A_5}^{B_1} - u_{X_1}^{E_u^{(0)}} u_{A_4}^{A_1} u_{A_2}^{B_1} + u_{X_1}^{E_u^{(0)}} u_{A_4}^{B_1} u_{A_2}^{A_1} + u_{A_3}^{A_1} u_{X_2}^{E_u^{(0)}} u_{A_1}^{B_1} - u_{A_3}^{B_1} u_{X_2}^{E_u^{(0)}} u_{A_1}^{A_1} \\
& - u_{A_3}^{B_1} u_{X_2}^{E_u^{(0)}} u_{A_1}^{A_1} + u_{A_3}^{A_1} u_{X_2}^{E_u^{(0)}} u_{A_1}^{B_1} - u_{X_1}^{E_u^{(0)}} u_{A_2}^{B_1} u_{A_4}^{A_1} + u_{X_1}^{E_u^{(0)}} u_{A_2}^{A_1} u_{A_4}^{B_1} ) \\
& + d_{A_3 X_2 \bar{A}_1}^{A_1 E_u {}^1B_1} (-u_{X_2}^{E_u^{(1)}} u_{\bar{A}}^{^1B_$$

[illegible]

[illegible]



$$\begin{aligned}
& + u_X^{E_g^{(0)}} u_{\bar{A}_2}^{1A_1} u_{A_4}^{1B_1} + u_{\bar{A}_3}^{1A_1} u_{\bar{A}_1}^{1B_1} u_X^{E_g^{(1)}} - u_{\bar{A}_3}^{1B_1} u_{\bar{A}_1}^{1A_1} u_X^{E_g^{(1)}} - u_{A_2}^{1A_1} u_{\bar{A}_4}^{1B_1} u_X^{E_g^{(0)}} + u_{A_2}^{1B_1} u_{\bar{A}_4}^{1A_1} u_X^{E_g^{(0)}} \\
& + u_{A_3}^{1B_1} u_X^{E_g^{(1)}} u_{A_1}^{1A_1} - u_{A_3}^{1A_1} u_X^{E_g^{(1)}} u_{A_1}^{1B_1} - u_{A_5}^{1A_1} u_A^{1B_1} u_{X_2}^{E_g^{(0)}} + u_{A_5}^{1B_1} u_A^{1A_1} u_{X_2}^{E_g^{(0)}} - u_{X_1}^{E_g^{(0)}} u_A^{1A_1} u_{\bar{A}_5}^{1A_1} \\
& + u_{X_1}^{E_g^{(0)}} u_A^{1A_1} u_{\bar{A}_5}^{1B_1} - u_{X_1}^{E_g^{(1)}} u_{\bar{A}_4}^{1A_1} u_{\bar{A}_2}^{1B_1} + u_{X_1}^{E_g^{(1)}} u_{\bar{A}_4}^{1B_1} u_{\bar{A}_2}^{1A_1} - u_{A_3}^{1A_1} u_{X_2}^{E_g^{(1)}} u_{\bar{A}_1}^{1B_1} + u_{A_3}^{1B_1} u_{X_2}^{E_g^{(1)}} u_{\bar{A}_1}^{1A_1} \\
& - u_{\bar{A}_3}^{1B_1} u_{X_2}^{E_g^{(1)}} u_{A_1}^{1A_1} + u_{\bar{A}_3}^{1A_1} u_{X_2}^{E_g^{(1)}} u_{A_1}^{1B_1} + u_{X_1}^{E_g^{(1)}} u_{A_2}^{1B_1} u_{A_4}^{1A_1} - u_{X_1}^{E_g^{(1)}} u_{A_2}^{1A_1} u_{A_4}^{1B_1} \\
& + d_{A_3 X_2 \bar{A}_1}^{1A_1 E_g 2B_1} (u_{X_2}^{E_g^{(0)}} u_{\bar{A}}^{2B_1} u_{\bar{A}_5}^{1A_1} - u_{X_2}^{E_g^{(0)}} u_{\bar{A}}^{1A_1} u_{\bar{A}_5}^{2B_1} + u_{X_1}^{E_g^{(0)}} u_{A_5}^{1A_1} u_{\bar{A}}^{2B_1} - u_{X_1}^{E_g^{(0)}} u_{A_5}^{2B_1} u_{\bar{A}}^{1A_1} - u_X^{E_g^{(0)}} u_{\bar{A}_2}^{2B_1} u_{A_4}^{1A_1} \\
& + u_X^{E_g^{(0)}} u_{\bar{A}_2}^{1A_1} u_{A_4}^{2B_1} + u_{\bar{A}_3}^{1A_1} u_{\bar{A}_1}^{2B_1} u_X^{E_g^{(1)}} - u_{\bar{A}_3}^{2B_1} u_{\bar{A}_1}^{1A_1} u_X^{E_g^{(1)}} - u_{A_2}^{1A_1} u_{\bar{A}_4}^{2B_1} u_X^{E_g^{(0)}} + u_{A_2}^{2B_1} u_{\bar{A}_4}^{1A_1} u_X^{E_g^{(0)}} \\
& + u_{A_3}^{2B_1} u_X^{E_g^{(1)}} u_{A_1}^{1A_1} - u_{A_3}^{1A_1} u_X^{E_g^{(1)}} u_{A_1}^{2B_1} - u_{A_5}^{1A_1} u_A^{2B_1} u_{X_2}^{E_g^{(0)}} + u_{A_5}^{2B_1} u_A^{1A_1} u_{X_2}^{E_g^{(0)}} - u_{X_1}^{E_g^{(0)}} u_A^{2B_1} u_{\bar{A}_5}^{1A_1} \\
& + u_{X_1}^{E_g^{(0)}} u_A^{1A_1} u_{\bar{A}_5}^{2B_1} - u_{X_1}^{E_g^{(1)}} u_{\bar{A}_4}^{1A_1} u_{\bar{A}_2}^{2B_1} + u_{X_1}^{E_g^{(1)}} u_{\bar{A}_4}^{2B_1} u_{\bar{A}_2}^{1A_1} - u_{A_3}^{1A_1} u_{X_2}^{E_g^{(1)}} u_{\bar{A}_1}^{2B_1} + u_{A_3}^{2B_1} u_{X_2}^{E_g^{(1)}} u_{\bar{A}_1}^{1A_1} \\
& - u_{\bar{A}_3}^{2B_1} u_{X_2}^{E_g^{(1)}} u_{A_1}^{1A_1} + u_{\bar{A}_3}^{1A_1} u_{X_2}^{E_g^{(1)}} u_{A_1}^{2B_1} + u_{X_1}^{E_g^{(1)}} u_{A_2}^{2B_1} u_{A_4}^{1A_1} - u_{X_1}^{E_g^{(1)}} u_{A_2}^{1A_1} u_{A_4}^{2B_1} \\
& + d_{A_3 X_2 \bar{A}_1}^{1A_1 E_g 2A_1} (-u_{X_2}^{E_g^{(1)}} u_{\bar{A}}^{2A_1} u_{\bar{A}_5}^{1A_1} + u_{X_2}^{E_g^{(1)}} u_{\bar{A}}^{1A_1} u_{\bar{A}_5}^{2A_1} + u_{X_1}^{E_g^{(1)}} u_{A_5}^{1A_1} u_{\bar{A}}^{2A_1} - u_{X_1}^{E_g^{(1)}} u_{A_5}^{2A_1} u_{\bar{A}}^{1A_1} + u_X^{E_g^{(1)}} u_{\bar{A}_2}^{2A_1} u_{A_4}^{1A_1} \\
& - u_X^{E_g^{(1)}} u_{\bar{A}_2}^{1A_1} u_{A_4}^{2A_1} + u_{\bar{A}_3}^{1A_1} u_{\bar{A}_1}^{2A_1} u_X^{E_g^{(0)}} - u_{\bar{A}_3}^{2A_1} u_{\bar{A}_1}^{1A_1} u_X^{E_g^{(0)}} - u_{A_2}^{1A_1} u_{\bar{A}_4}^{2A_1} u_X^{E_g^{(1)}} + u_{A_2}^{2A_1} u_{\bar{A}_4}^{1A_1} u_X^{E_g^{(1)}} \\
& - u_{A_3}^{2A_1} u_X^{E_g^{(0)}} u_{A_1}^{1A_1} + u_{A_3}^{1A_1} u_X^{E_g^{(0)}} u_{A_1}^{2A_1} - u_{A_5}^{1A_1} u_A^{2A_1} u_{X_2}^{E_g^{(1)}} + u_{A_5}^{2A_1} u_A^{1A_1} u_{X_2}^{E_g^{(1)}} + u_{X_1}^{E_g^{(1)}} u_A^{2A_1} u_{\bar{A}_5}^{1A_1} \\
& - u_{X_1}^{E_g^{(1)}} u_A^{1A_1} u_{\bar{A}_5}^{2A_1} - u_{X_1}^{E_g^{(0)}} u_{\bar{A}_4}^{1A_1} u_{\bar{A}_2}^{2A_1} + u_{X_1}^{E_g^{(0)}} u_{\bar{A}_4}^{2A_1} u_{\bar{A}_2}^{1A_1} - u_{A_3}^{1A_1} u_{X_2}^{E_g^{(0)}} u_{\bar{A}_1}^{2A_1} + u_{A_3}^{2A_1} u_{X_2}^{E_g^{(0)}} u_{\bar{A}_1}^{1A_1} \\
& + u_{\bar{A}_3}^{2A_1} u_{X_2}^{E_g^{(0)}} u_{A_1}^{1A_1} - u_{\bar{A}_3}^{1A_1} u_{X_2}^{E_g^{(0)}} u_{A_1}^{2A_1} - u_{X_1}^{E_g^{(0)}} u_{A_2}^{2A_1} u_{A_4}^{1A_1} + u_{X_1}^{E_g^{(0)}} u_{A_2}^{1A_1} u_{A_4}^{2A_1} \\
& + d_{A_3 X_2 \bar{A}_1}^{1A_1 E_g B_2} (-u_{X_2}^{E_g^{(1)}} u_{\bar{A}}^{B_2} u_{\bar{A}_5}^{1A_1} + u_{X_2}^{E_g^{(1)}} u_{\bar{A}}^{1A_1} u_{\bar{A}_5}^{B_2} - u_{X_1}^{E_g^{(1)}} u_{A_5}^{1A_1} u_{\bar{A}}^{B_2} + u_{X_1}^{E_g^{(1)}} u_{A_5}^{B_2} u_{\bar{A}}^{1A_1} - u_X^{E_g^{(1)}} u_{\bar{A}_2}^{B_2} u_{A_4}^{1A_1} \\
& + u_X^{E_g^{(1)}} u_{\bar{A}_2}^{1A_1} u_{A_4}^{B_2} + u_{\bar{A}_3}^{1A_1} u_{\bar{A}_1}^{B_2} u_X^{E_g^{(0)}} - u_{\bar{A}_3}^{B_2} u_{\bar{A}_1}^{1A_1} u_X^{E_g^{(0)}} + u_{A_2}^{1A_1} u_{\bar{A}_4}^{B_2} u_X^{E_g^{(1)}} - u_{A_2}^{B_2} u_{\bar{A}_4}^{1A_1} u_X^{E_g^{(1)}} \\
& - u_{A_3}^{B_2} u_X^{E_g^{(0)}} u_{A_1}^{1A_1} + u_{A_3}^{1A_1} u_X^{E_g^{(0)}} u_{A_1}^{B_2} - u_{A_5}^{1A_1} u_A^{B_2} u_{X_2}^{E_g^{(1)}} + u_{A_5}^{B_2} u_A^{1A_1} u_{X_2}^{E_g^{(1)}} - u_{X_1}^{E_g^{(1)}} u_A^{B_2} u_{\bar{A}_5}^{1A_1} \\
& + u_{X_1}^{E_g^{(1)}} u_A^{1A_1} u_{\bar{A}_5}^{B_2} - u_{X_1}^{E_g^{(0)}} u_{\bar{A}_4}^{1A_1} u_{\bar{A}_2}^{B_2} + u_{X_1}^{E_g^{(0)}} u_{\bar{A}_4}^{B_2} u_{\bar{A}_2}^{1A_1} + u_{A_3}^{1A_1} u_{X_2}^{E_g^{(0)}} u_{\bar{A}_1}^{B_2} - u_{A_3}^{B_2} u_{X_2}^{E_g^{(0)}} u_{\bar{A}_1}^{1A_1} \\
& - u_{\bar{A}_3}^{B_2} u_{X_2}^{E_g^{(0)}} u_{A_1}^{1A_1} + u_{\bar{A}_3}^{1A_1} u_{X_2}^{E_g^{(0)}} u_{A_1}^{B_2} - u_{X_1}^{E_g^{(0)}} u_{A_2}^{B_2} u_{A_4}^{1A_1} + u_{X_1}^{E_g^{(0)}} u_{A_2}^{1A_1} u_{A_4}^{B_2} \\
& + d_{A_3 X_2 \bar{A}_1}^{1A_1 E_g 1B_2} (-u_{X_2}^{E_g^{(1)}} u_{\bar{A}}^{1B_2} u_{\bar{A}_5}^{1A_1} + u_{X_2}^{E_g^{(1)}} u_{\bar{A}}^{1A_1} u_{\bar{A}_5}^{1B_2} - u_{X_1}^{E_g^{(1)}} u_{A_5}^{1A_1} u_{\bar{A}}^{1B_2} + u_{X_1}^{E_g^{(1)}} u_{A_5}^{1B_2} u_{\bar{A}}^{1A_1} - u_X^{E_g^{(1)}} u_{\bar{A}_2}^{1B_2} u_{A_4}^{1A_1} \\
& + u_X^{E_g^{(1)}} u_{\bar{A}_2}^{1A_1} u_{A_4}^{1B_2} + u_{\bar{A}_3}^{1A_1} u_{\bar{A}_1}^{1B_2} u_X^{E_g^{(0)}} - u_{\bar{A}_3}^{1B_2} u_{\bar{A}_1}^{1A_1} u_X^{E_g^{(0)}} + u_{A_2}^{1A_1} u_{\bar{A}_4}^{1B_2} u_X^{E_g^{(1)}} - u_{A_2}^{1B_2} u_{\bar{A}_4}^{1A_1} u_X^{E_g^{(1)}} \\
& - u_{A$$

$$\begin{aligned}
& + u_X^{A_2u} u_{A_2}^{1A_1} u_{A_4}^{B_2} + u_{A_3}^{1A_1} u_{A_1}^{B_2} u_X^{A_2u} + u_{A_3}^{B_2} u_{A_1}^{1A_1} u_X^{A_2u} - u_{A_2}^{1A_1} u_{A_4}^{B_2} u_X^{A_2u} - u_{A_2}^{B_2} u_{A_4}^{1A_1} u_X^{A_2u} \\
& - u_{A_3}^{B_2} u_X^{A_2u} u_{A_1}^{1A_1} - u_{A_3}^{1A_1} u_X^{A_2u} u_{A_1}^{B_2} + u_{A_5}^{1A_1} u_A^{B_2} u_{X_2}^{A_2u} + u_{A_5}^{B_2} u_A^{1A_1} u_{X_2}^{A_2u} + u_{X_1}^{A_2u} u_A^{B_2} u_{A_5}^{1A_1} \\
& + u_{X_1}^{A_2u} u_A^{1A_1} u_{A_5}^{B_2} + u_{X_1}^{A_2u} u_{A_4}^{1A_1} u_{A_2}^{B_2} + u_{X_1}^{A_2u} u_{A_4}^{B_2} u_{A_2}^{1A_1} - u_{A_3}^{1A_1} u_{X_2}^{A_2u} u_{A_1}^{B_2} - u_{A_3}^{B_2} u_{X_2}^{A_2u} u_{A_1}^{1A_1} \\
& + u_{A_3}^{B_2} u_{X_2}^{A_2u} u_{A_1}^{1A_1} + u_{A_3}^{1A_1} u_{X_2}^{A_2u} u_{A_1}^{B_2} - u_{X_1}^{A_2u} u_{A_2}^{B_2} u_{A_4}^{1A_1} - u_{X_1}^{A_2u} u_{A_2}^{1A_1} u_{A_4}^{B_2}) \\
+ d_{A_3 X_2}^{1A_1 A_2 u} \bar{B}_2 (-u_{X_2}^{A_2u} u_{\bar{A}}^{1B_2} u_{\bar{A}_5}^{1A_1} - u_{X_2}^{A_2u} u_{\bar{A}}^{1A_1} u_{\bar{A}_5}^{1B_2} - u_{X_1}^{A_2u} u_{A_5}^{1A_1} u_{\bar{A}}^{1B_2} - u_{X_1}^{A_2u} u_{A_5}^{1B_2} u_{\bar{A}}^{1A_1} + u_{X_2}^{A_2u} u_{\bar{A}_2}^{1B_2} u_{A_4}^{1A_1} \\
& + u_{X_2}^{A_2u} u_{\bar{A}_2}^{1A_1} u_{A_4}^{1B_2} + u_{A_3}^{1A_1} u_{\bar{A}_1}^{1B_2} u_X^{A_2u} + u_{A_3}^{1B_2} u_{\bar{A}_1}^{1A_1} u_X^{A_2u} - u_{A_2}^{1A_1} u_{A_4}^{1B_2} u_X^{A_2u} - u_{A_2}^{1B_2} u_{A_4}^{1A_1} u_X^{A_2u} \\
& - u_{A_3}^{1B_2} u_X^{A_2u} u_{A_1}^{1A_1} - u_{A_3}^{1A_1} u_X^{A_2u} u_{A_1}^{1B_2} + u_{A_5}^{1A_1} u_A^{1B_2} u_{X_2}^{A_2u} + u_{A_5}^{1B_2} u_A^{1A_1} u_{X_2}^{A_2u} + u_{X_1}^{A_2u} u_A^{1B_2} u_{A_5}^{1A_1} \\
& + u_{X_1}^{A_2u} u_A^{1A_1} u_{A_5}^{1B_2} + u_{X_1}^{A_2u} u_{A_4}^{1A_1} u_{A_2}^{1B_2} + u_{X_1}^{A_2u} u_{A_4}^{1B_2} u_{A_2}^{1A_1} - u_{A_3}^{1A_1} u_{X_2}^{A_2u} u_{A_1}^{1B_2} - u_{A_3}^{1B_2} u_{X_2}^{A_2u} u_{A_1}^{1A_1} \\
& + u_{A_3}^{1B_2} u_{X_2}^{A_2u} u_{A_1}^{1A_1} + u_{A_3}^{1A_1} u_{X_2}^{A_2u} u_{A_1}^{1B_2} - u_{X_1}^{A_2u} u_{A_2}^{1B_2} u_{A_4}^{1A_1} - u_{X_1}^{A_2u} u_{A_2}^{1A_1} u_{A_4}^{1B_2}) \\
+ d_{A_3 X_2}^{1A_1 B_1 u} A_2 (u_{X_2}^{B_1u} u_{\bar{A}}^{A_2} u_{\bar{A}_5}^{1A_1} + u_{X_2}^{B_1u} u_{\bar{A}}^{1A_1} u_{\bar{A}_5}^{A_2} - u_{X_1}^{B_1u} u_{A_5}^{1A_1} u_{\bar{A}}^{A_2} - u_{X_1}^{B_1u} u_{A_5}^{A_2} u_{\bar{A}}^{1A_1} - u_X^{B_1u} u_{A_2}^{A_2} u_{A_4}^{1A_1} \\
& - u_X^{B_1u} u_{A_2}^{1A_1} u_{A_4}^{A_2} + u_{A_3}^{1A_1} u_{A_1}^{A_2} u_X^{B_1u} + u_{A_3}^{A_2} u_{A_1}^{1A_1} u_X^{B_1u} - u_{A_2}^{1A_1} u_{A_4}^{A_2} u_X^{B_1u} - u_{A_2}^{A_2} u_{A_4}^{1A_1} u_X^{B_1u} \\
& + u_{A_3}^{A_2} u_X^{B_1u} u_{A_1}^{1A_1} + u_{A_3}^{1A_1} u_X^{B_1u} u_{A_1}^{A_2} + u_{A_5}^{1A_1} u_A^{A_2} u_{X_2}^{B_1u} + u_{A_5}^{A_2} u_A^{1A_1} u_{X_2}^{B_1u} - u_{X_1}^{B_1u} u_A^{A_2} u_{A_5}^{1A_1} \\
& - u_{X_1}^{B_1u} u_A^{1A_1} u_{A_5}^{A_2} + u_{X_1}^{B_1u} u_{A_4}^{1A_1} u_{A_2}^{A_2} + u_{X_1}^{B_1u} u_{A_4}^{A_2} u_{A_2}^{1A_1} - u_{A_3}^{1A_1} u_{X_2}^{B_1u} u_{A_1}^{A_2} - u_{A_3}^{A_2} u_{X_2}^{B_1u} u_{A_1}^{1A_1} \\
& - u_{A_3}^{A_2} u_{X_2}^{B_1u} u_{A_1}^{1A_1} - u_{A_3}^{1A_1} u_{X_2}^{B_1u} u_{A_1}^{A_2} + u_{X_1}^{B_1u} u_{A_2}^{A_2} u_{A_4}^{1A_1} + u_{X_1}^{B_1u} u_{A_2}^{1A_1} u_{A_4}^{A_2}) \\
+ d_{A_3 X_2}^{1A_1 B_1 u} B_1 (u_{X_2}^{B_1u} u_{\bar{A}}^{B_1} u_{A_5}^{1A_1} + u_{X_2}^{B_1u} u_{\bar{A}}^{1A_1} u_{A_5}^{B_1} + u_{X_1}^{B_1u} u_{A_5}^{1A_1} u_{\bar{A}}^{B_1} + u_{X_1}^{B_1u} u_{A_5}^{B_1} u_{\bar{A}}^{1A_1} + u_X^{B_1u} u_{A_2}^{B_1} u_{A_4}^{1A_1} \\
& + u_X^{B_1u} u_{A_2}^{1A_1} u_{A_4}^{B_1} + u_{A_3}^{1A_1} u_{A_1}^{B_1} u_X^{B_1u} + u_{A_3}^{B_1} u_{A_1}^{1A_1} u_X^{B_1u} + u_{A_2}^{1A_1} u_{A_4}^{B_1} u_X^{B_1u} + u_{A_2}^{B_1} u_{A_4}^{1A_1} u_X^{B_1u} \\
& + u_{A_3}^{B_1u} u_X^{B_1u} u_{A_1}^{1A_1} + u_{A_3}^{1A_1} u_X^{B_1u} u_{A_1}^{B_1} + u_{A_5}^{1A_1} u_A^{B_1} u_{X_2}^{B_1u} + u_{A_5}^{B_1} u_A^{1A_1} u_{X_2}^{B_1u} + u_{X_1}^{B_1u} u_A^{B_1} u_{A_5}^{1A_1} \\
& + u_{X_1}^{B_1u} u_A^{1A_1} u_{A_5}^{B_1} + u_{X_1}^{B_1u} u_{A_4}^{1A_1} u_{A_2}^{B_1} + u_{X_1}^{B_1u} u_{A_4}^{B_1} u_{A_2}^{1A_1} + u_{A_3}^{1A_1} u_{X_2}^{B_1u} u_{A_1}^{B_1} + u_{A_3}^{B_1} u_{X_2}^{B_1u} u_{A_1}^{1A_1} \\
& + u_{A_3}^{B_1} u_{X_2}^{B_1u} u_{A_1}^{1A_1} + u_{A_3}^{1A_1} u_{X_2}^{B_1u} u_{A_1}^{B_1} + u_{X_1}^{B_1u} u_{A_2}^{B_1} u_{A_4}^{1A_1} + u_{X_1}^{B_1u} u_{A_2}^{1A_1} u_{A_4}^{B_1}) \\
+ d_{A_3 X_2}^{1A_1 B_1 u} \bar{B}_1 (u_{X_2}^{B_1u} u_{\bar{A}}^{1B_1} u_{\bar{A}_5}^{1A_1} + u_{X_2}^{B_1u} u_{\bar{A}}^{1A_1} u_{\bar{A}_5}^{1B_1} + u_{X_1}^{B_1u} u_{A_5}^{1A_1} u_{\bar{A}}^{1B_1} + u_{X_1}^{B_1u} u_{A_5}^{1B_1} u_{\bar{A}}^{1A_1} + u_X^{B_1u} u_{A_2}^{1B_1} u_{A_4}^{1A_1} \\
& + u_X^{B_1u} u_{A_2}^{1A_1} u_{A_4}^{1B_1} + u_{A_3}^{1A_1} u_{A_1}^{1B_1} u_X^{B_1u} + u_{A_3}^{1B_1} u_{A_1}^{1A_1} u_X^{B_1u} + u_{A_2}^{1A_1} u_{A_4}^{1B_1} u_X^{B_1u} + u_{A_2}^{1B_1} u_{A_4}^{1A_1} u_X^{B_1u} \\
& + u_{A_3}^{1B_1} u_X^{B_1u} u_{A_1}^{1A_1} + u_{A_3}^{1A_1} u_X^{B_1u} u_{A_1}^{1B_1} + u_{A_5}^{1A_1} u_A^{1B_1} u_{X_2}^{B_1u} + u_{A_5}^{1B_1} u_A^{1A_1} u_{X_2}^{B_1u} + u_{X_1}^{B_1u} u_A^{1B_1} u_{A_5}^{1A_1} \\
& + u_{X_1}^{B_1u} u_A^{1A_1} u_{A_5}^{1B_1} + u_{X_1}^{B_1u} u_{A_4}^{1A_1} u_{A_2}^{1B_1} + u_{X_1}^{B_1u} u_{A_4}^{1B_1} u_{A_2}^{1A_1} + u_{A_3}^{1A_1} u_{X_2}^{B_1u} u_{A_1}^{1B_1} + u_{A_3}^{1B_1} u_{X_2}^{B_1u} u_{A_1}^{1A_1} \\
& + u_{A_3}^{1B_1} u_{X_2}^{B_1u} u_{A_1}^{1A_1} + u_{$$



[illegible]

93



$$\begin{aligned}
& + u_X^{B_{1u}} u_{A_2}^{2A_1} u_{A_4}^{2B_1} + u_{A_3}^{2A_1} u_{A_1}^{2B_1} u_X^{B_{1u}} + u_{A_3}^{2B_1} u_{A_1}^{2A_1} u_X^{B_{1u}} + u_{A_2}^{2A_1} u_{A_4}^{2B_1} u_X^{B_{1u}} + u_{A_2}^{2B_1} u_{A_4}^{2A_1} u_X^{B_{1u}} \\
& + u_{A_3}^{2B_1} u_X^{B_{1u}} u_{A_1}^{2A_1} + u_{A_3}^{2A_1} u_X^{B_{1u}} u_{A_1}^{2B_1} + u_{A_5}^{2A_1} u_A^{2B_1} u_{X_2}^{B_{1u}} + u_{A_5}^{2B_1} u_A^{2A_1} u_{X_2}^{B_{1u}} + u_{X_1}^{B_{1u}} u_A^{2B_1} u_{A_5}^{2A_1} \\
& + u_{X_1}^{B_{1u}} u_A^{2A_1} u_{A_5}^{2B_1} + u_{X_1}^{B_{1u}} u_{A_4}^{2A_1} u_{A_2}^{2B_1} + u_{X_1}^{B_{1u}} u_{A_4}^{2B_1} u_{A_2}^{2A_1} + u_{A_3}^{2A_1} u_{X_2}^{B_{1u}} u_{A_1}^{2B_1} + u_{A_3}^{2B_1} u_{X_2}^{B_{1u}} u_{A_1}^{2A_1} \\
& + u_{A_3}^{2B_1} u_{X_2}^{B_{1u}} u_{A_1}^{2A_1} + u_{A_3}^{2A_1} u_{X_2}^{B_{1u}} u_{A_1}^{2B_1} + u_{X_1}^{B_{1u}} u_{A_2}^{2B_1} u_{A_4}^{2A_1} + u_{X_1}^{B_{1u}} u_{A_2}^{2A_1} u_{A_4}^{2B_1} ) \\
& + d_{A_3 X_2 A_1}^{2A_1 E_u B_2} (u_{X_2}^{E_u^{(0)}} u_{\bar{A}}^{B_2} u_{\bar{A}_5}^{2A_1} - u_{X_2}^{E_u^{(0)}} u_{\bar{A}}^{2A_1} u_{A_5}^{B_2} + u_{X_1}^{E_u^{(0)}} u_{A_5}^{2A_1} u_{\bar{A}}^{B_2} - u_{X_1}^{E_u^{(0)}} u_{A_5}^{B_2} u_{\bar{A}}^{2A_1} - u_{X'}^{E_u^{(0)}} u_{\bar{A}_2}^{B_2} u_{A_4}^{2A_1} \\
& + u_{X'}^{E_u^{(0)}} u_{\bar{A}_2}^{2A_1} u_{A_4}^{B_2} + u_{A_3}^{2A_1} u_{A_1}^{B_2} u_{X'}^{E_u^{(0)}} - u_{A_3}^{B_2} u_{A_1}^{2A_1} u_{X'}^{E_u^{(0)}} - u_{A_2}^{2A_1} u_{A_4}^{B_2} u_{X'}^{E_u^{(0)}} + u_{A_2}^{B_2} u_{A_4}^{2A_1} u_{X'}^{E_u^{(0)}} \\
& + u_{A_3}^{B_2} u_{X'}^{E_u^{(1)}} u_{A_1}^{2A_1} - u_{A_3}^{2A_1} u_{X'}^{E_u^{(1)}} u_{A_1}^{B_2} - u_{A_5}^{2A_1} u_A^{B_2} u_{X_2}^{E_u^{(0)}} + u_{A_5}^{B_2} u_A^{2A_1} u_{X_2}^{E_u^{(0)}} - u_{X_1}^{E_u^{(0)}} u_A^{B_2} u_{A_5}^{2A_1} \\
& + u_{X_1}^{E_u^{(0)}} u_A^{2A_1} u_{A_5}^{B_2} - u_{X_1}^{E_u^{(1)}} u_{A_4}^{2A_1} u_{A_2}^{B_2} + u_{X_1}^{E_u^{(1)}} u_{A_4}^{B_2} u_{A_2}^{2A_1} - u_{A_3}^{2A_1} u_{X_2}^{E_u^{(1)}} u_{A_1}^{B_2} + u_{A_3}^{B_2} u_{X_2}^{E_u^{(1)}} u_{A_1}^{2A_1} \\
& - u_{A_3}^{B_2} u_{X_2}^{E_u^{(1)}} u_{A_1}^{2A_1} + u_{A_3}^{2A_1} u_{X_2}^{E_u^{(1)}} u_{A_1}^{B_2} + u_{X_1}^{E_u^{(1)}} u_{A_2}^{B_2} u_{A_4}^{2A_1} - u_{X_1}^{E_u^{(1)}} u_{A_2}^{2A_1} u_{A_4}^{B_2} ) \\
& + d_{A_3 X_2 A_1}^{2A_1 E_u B_2} (u_{X_2}^{E_u^{(0)}} u_{\bar{A}}^{1B_2} u_{A_5}^{2A_1} - u_{X_2}^{E_u^{(0)}} u_{\bar{A}}^{2A_1} u_{A_5}^{1B_2} + u_{X_1}^{E_u^{(0)}} u_{A_5}^{2A_1} u_{\bar{A}}^{1B_2} - u_{X_1}^{E_u^{(0)}} u_{A_5}^{1B_2} u_{\bar{A}}^{2A_1} - u_{X'}^{E_u^{(0)}} u_{\bar{A}_2}^{1B_2} u_{A_4}^{2A_1} \\
& + u_{X'}^{E_u^{(0)}} u_{\bar{A}_2}^{2A_1} u_{A_4}^{1B_2} + u_{A_3}^{2A_1} u_{A_1}^{1B_2} u_{X'}^{E_u^{(1)}} - u_{A_3}^{1B_2} u_{A_1}^{2A_1} u_{X'}^{E_u^{(1)}} - u_{A_2}^{2A_1} u_{A_4}^{1B_2} u_{X'}^{E_u^{(0)}} + u_{A_2}^{1B_2} u_{A_4}^{2A_1} u_{X'}^{E_u^{(0)}} \\
& + u_{A_3}^{1B_2} u_{X'}^{E_u^{(1)}} u_{A_1}^{2A_1} - u_{A_3}^{2A_1} u_{X'}^{E_u^{(1)}} u_{A_1}^{1B_2} - u_{A_5}^{2A_1} u_A^{1B_2} u_{X_2}^{E_u^{(0)}} + u_{A_5}^{1B_2} u_A^{2A_1} u_{X_2}^{E_u^{(0)}} - u_{X_1}^{E_u^{(0)}} u_A^{1B_2} u_{A_5}^{2A_1} \\
& + u_{X_1}^{E_u^{(0)}} u_A^{2A_1} u_{A_5}^{1B_2} - u_{X_1}^{E_u^{(1)}} u_{A_4}^{2A_1} u_{A_2}^{1B_2} + u_{X_1}^{E_u^{(1)}} u_{A_4}^{1B_2} u_{A_2}^{2A_1} - u_{A_3}^{2A_1} u_{X_2}^{E_u^{(1)}} u_{A_1}^{1B_2} + u_{A_3}^{1B_2} u_{X_2}^{E_u^{(1)}} u_{A_1}^{2A_1} \\
& - u_{A_3}^{1B_2} u_{X_2}^{E_u^{(1)}} u_{A_1}^{2A_1} + u_{A_3}^{2A_1} u_{X_2}^{E_u^{(1)}} u_{A_1}^{1B_2} + u_{X_1}^{E_u^{(1)}} u_{A_2}^{1B_2} u_{A_4}^{2A_1} - u_{X_1}^{E_u^{(1)}} u_{A_2}^{2A_1} u_{A_4}^{1B_2} ) \\
& + d_{A_3 X_2 A_1}^{2A_1 E_u A_2} (-u_{X_2}^{E_u^{(1)}} u_{\bar{A}}^{A_2} u_{A_5}^{2A_1} + u_{X_2}^{E_u^{(1)}} u_{\bar{A}}^{2A_1} u_{A_5}^{A_2} + u_{X_1}^{E_u^{(1)}} u_{A_5}^{2A_1} u_{\bar{A}}^{A_2} - u_{X_1}^{E_u^{(1)}} u_{A_5}^{A_2} u_{\bar{A}}^{2A_1} + u_{X'}^{E_u^{(1)}} u_{\bar{A}_2}^{A_2} u_{A_4}^{2A_1} \\
& - u_{X'}^{E_u^{(1)}} u_{\bar{A}_2}^{2A_1} u_{A_4}^{A_2} + u_{A_3}^{2A_1} u_{A_1}^{A_2} u_{X'}^{E_u^{(0)}} - u_{A_3}^{A_2} u_{A_1}^{2A_1} u_{X'}^{E_u^{(0)}} - u_{A_2}^{2A_1} u_{A_4}^{A_2} u_{X'}^{E_u^{(1)}} + u_{A_2}^{A_2} u_{A_4}^{2A_1} u_{X'}^{E_u^{(1)}} \\
& - u_{A_3}^{A_2} u_{X'}^{E_u^{(0)}} u_{A_1}^{2A_1} + u_{A_3}^{2A_1} u_{X'}^{E_u^{(0)}} u_{A_1}^{A_2} - u_{A_5}^{2A_1} u_A^{A_2} u_{X_2}^{E_u^{(1)}} + u_{A_5}^{A_2} u_A^{2A_1} u_{X_2}^{E_u^{(1)}} + u_{X_1}^{E_u^{(1)}} u_A^{A_2} u_{A_5}^{2A_1} \\
& - u_{X_1}^{E_u^{(1)}} u_A^{2A_1} u_{A_5}^{A_2} - u_{X_1}^{E_u^{(0)}} u_{A_4}^{2A_1} u_{A_2}^{A_2} + u_{X_1}^{E_u^{(0)}} u_{A_4}^{A_2} u_{A_2}^{2A_1} - u_{A_3}^{2A_1} u_{X_2}^{E_u^{(0)}} u_{A_1}^{A_2} + u_{A_3}^{A_2} u_{X_2}^{E_u^{(0)}} u_{A_1}^{2A_1} \\
& + u_{A_3}^{A_2} u_{X_2}^{E_u^{(0)}} u_{A_1}^{2A_1} - u_{A_3}^{2A_1} u_{X_2}^{E_u^{(0)}} u_{A_1}^{A_2} - u_{X_1}^{E_u^{(0)}} u_{A_2}^{A_2} u_{A_4}^{2A_1} + u_{X_1}^{E_u^{(0)}} u_{A_2}^{2A_1} u_{A_4}^{A_2} ) \\
& + d_{A_3 X_2 A_1}^{2A_1 E_u B_1} (-u_{X_2}^{E_u^{(1)}} u_{\bar{A}}^{B_1} u_{A_5}^{2A_1} + u_{X_2}^{E_u^{(1)}} u_{\bar{A}}^{2A_1} u_{A_5}^{B_1} - u_{X_1}^{E_u^{(1)}} u_{A_5}^{2A_1} u_{\bar{A}}^{B_1} + u_{X_1}^{E_u^{(1)}} u_{A_5}^{B_1} u_{\bar{A}}^{2A_1} - u_{X'}^{E_u^{(1)}} u_{\bar{A}_2}^{B_1} u_{A_4}^{2A_1} \\
& + u_{X'}^{E_u^{(1)}} u_{\bar{A}_2}^{2A_1} u_{A_4}^{B_1} + u_{A_3}^{2A_1} u_{A_1}^{B_1} u_{X'}^{E_u^{(0)}} - u_{A_3}^{B_1} u_{A_1}^{2A_1} u_{X'}^{E_u^{(0)}} + u_{A_2}^{2A_1} u_{A_4}^{B_1} u_{X'}^{E_u^{(1)}} - u_{A_2}^{B_1} u_{A_4}^{2A_1} u_{X'}^{E_u^{(1)}} \\
& - u_{A_3}^{B_1} u_{X'}^{E_u^{(0)}} u_{A_1}^{2A_1} + u_{A_3}^{2A_1} u_{X'}^{E_u^{(0)}} u_{A_1}^{B_1} - u_{A_5}^{2A_1} u_A^{B_1} u_{X_2}^{E_u^{(1)}} + u_{A_5}^{B_1} u_A^{2A_1} u_{X_2}^{E_u^{(1)}} - u_{X_1}^{E_u^{(1)}} u_A^{B_1} u_{A_5}^{2A_1} \\
& + u_{X_1}^{E_u^{(1)}} u_A^{2A_1} u_{A_5}^{B_1} - u_{X_1}^{E_u^{(0)}} u_{A_4}^{2A_1} u_{A_2}^{B_1} + u$$

$$\begin{aligned}
& +d_{A_3 X_2 \bar{A}_1}^{2A_1 1E_u B_2} (u_{X_2}^{1E_u(0)} u_{\bar{A}}^{B_2} u_{\bar{A}_5}^{2A_1} - u_{X_2}^{1E_u(0)} u_{\bar{A}}^{2A_1} u_{\bar{A}_5}^{B_2} + u_{X_1}^{1E_u(0)} u_{A_5}^{2A_1} u_{\bar{A}}^{B_2} - u_{X_1}^{1E_u(0)} u_{A_5}^{B_2} u_{\bar{A}}^{2A_1} - u_X^{1E_u(0)} u_{\bar{A}_2}^{B_2} u_{A_4}^{2A_1} \\
& + u_X^{1E_u(0)} u_{\bar{A}_2}^{2A_1} u_{A_4}^{B_2} + u_{\bar{A}_3}^{2A_1} u_{\bar{A}_1}^{B_2} u_X^{1E_u(1)} - u_{\bar{A}_3}^{B_2} u_{\bar{A}_1}^{2A_1} u_X^{1E_u(1)} - u_{A_2}^{2A_1} u_{\bar{A}_4}^{B_2} u_X^{1E_u(0)} + u_{A_2}^{B_2} u_{\bar{A}_4}^{2A_1} u_X^{1E_u(0)} \\
& + u_{A_3}^{B_2} u_X^{1E_u(1)} u_{A_1}^{2A_1} - u_{A_3}^{2A_1} u_X^{1E_u(1)} u_{A_1}^{B_2} - u_{A_5}^{2A_1} u_{A_1}^{B_2} u_{X_2}^{1E_u(0)} + u_{A_5}^{B_2} u_{A_1}^{1E_u(0)} u_{X_2}^{2A_1} - u_{X_1}^{1E_u(0)} u_{A_4}^{B_2} u_{\bar{A}_5}^{2A_1} \\
& + u_{X_1}^{1E_u(0)} u_{A_4}^{2A_1} u_{\bar{A}_5}^{B_2} - u_{X_1}^{1E_u(1)} u_{\bar{A}_4}^{2A_1} u_{\bar{A}_2}^{B_2} + u_{X_1}^{1E_u(1)} u_{\bar{A}_4}^{B_2} u_{\bar{A}_2}^{2A_1} - u_{A_3}^{2A_1} u_{X_2}^{1E_u(1)} u_{\bar{A}_1}^{B_2} + u_{A_3}^{B_2} u_{X_2}^{1E_u(1)} u_{\bar{A}_1}^{2A_1} \\
& - u_{\bar{A}_3}^{B_2} u_{X_2}^{1E_u(1)} u_{A_1}^{2A_1} + u_{\bar{A}_3}^{2A_1} u_{X_2}^{1E_u(1)} u_{A_1}^{B_2} + u_{X_1}^{1E_u(1)} u_{A_4}^{B_2} u_{A_4}^{2A_1} - u_{X_1}^{1E_u(1)} u_{A_2}^{2A_1} u_{A_4}^{B_2}) \\
& +d_{A_3 X_2 \bar{A}_1}^{2A_1 1E_u 1B_2} (u_{X_2}^{1E_u(0)} u_{\bar{A}}^{1B_2} u_{\bar{A}_5}^{2A_1} - u_{X_2}^{1E_u(0)} u_{\bar{A}}^{2A_1} u_{\bar{A}_5}^{1B_2} + u_{X_1}^{1E_u(0)} u_{A_5}^{2A_1} u_{\bar{A}}^{1B_2} - u_{X_1}^{1E_u(0)} u_{A_5}^{1B_2} u_{\bar{A}}^{2A_1} - u_X^{1E_u(0)} u_{\bar{A}_2}^{1B_2} u_{A_4}^{2A_1} \\
& + u_X^{1E_u(0)} u_{\bar{A}_2}^{2A_1} u_{A_4}^{1B_2} + u_{\bar{A}_3}^{2A_1} u_{\bar{A}_1}^{1B_2} u_X^{1E_u(1)} - u_{\bar{A}_3}^{1B_2} u_{\bar{A}_1}^{2A_1} u_X^{1E_u(1)} - u_{A_2}^{2A_1} u_{\bar{A}_4}^{1B_2} u_X^{1E_u(0)} + u_{A_2}^{1B_2} u_{\bar{A}_4}^{2A_1} u_X^{1E_u(0)} \\
& + u_{A_3}^{1B_2} u_X^{1E_u(1)} u_{A_1}^{2A_1} - u_{A_3}^{2A_1} u_X^{1E_u(1)} u_{A_1}^{1B_2} - u_{A_5}^{2A_1} u_{A_1}^{1B_2} u_{X_2}^{1E_u(0)} + u_{A_5}^{1B_2} u_{A_1}^{2A_1} u_{X_2}^{1E_u(0)} - u_{X_1}^{1E_u(0)} u_{A_4}^{1B_2} u_{\bar{A}_5}^{2A_1} \\
& + u_{X_1}^{1E_u(0)} u_{A_4}^{2A_1} u_{\bar{A}_5}^{1B_2} - u_{X_1}^{1E_u(1)} u_{\bar{A}_4}^{2A_1} u_{\bar{A}_2}^{1B_2} + u_{X_1}^{1E_u(1)} u_{\bar{A}_4}^{1B_2} u_{\bar{A}_2}^{2A_1} - u_{A_3}^{2A_1} u_{X_2}^{1E_u(1)} u_{\bar{A}_1}^{1B_2} + u_{A_3}^{1B_2} u_{X_2}^{1E_u(1)} u_{\bar{A}_1}^{2A_1} \\
& - u_{\bar{A}_3}^{1B_2} u_{X_2}^{1E_u(1)} u_{A_1}^{2A_1} + u_{\bar{A}_3}^{2A_1} u_{X_2}^{1E_u(1)} u_{A_1}^{1B_2} + u_{X_1}^{1E_u(1)} u_{A_2}^{1B_2} u_{A_4}^{2A_1} - u_{X_1}^{1E_u(1)} u_{A_2}^{2A_1} u_{A_4}^{1B_2}) \\
& +d_{A_3 X_2 \bar{A}_1}^{2A_1 1E_u A_2} (-u_{X_2}^{1E_u(1)} u_{\bar{A}}^{A_2} u_{\bar{A}_5}^{2A_1} + u_{X_2}^{1E_u(1)} u_{\bar{A}}^{2A_1} u_{\bar{A}_5}^{A_2} + u_{X_1}^{1E_u(1)} u_{A_5}^{2A_1} u_{\bar{A}}^{A_2} - u_{X_1}^{1E_u(1)} u_{A_5}^{A_2} u_{\bar{A}}^{2A_1} + u_X^{1E_u(1)} u_{\bar{A}_2}^{A_2} u_{A_4}^{2A_1} \\
& - u_X^{1E_u(1)} u_{\bar{A}_2}^{2A_1} u_{A_4}^{A_2} + u_{\bar{A}_3}^{2A_1} u_{\bar{A}_1}^{A_2} u_X^{1E_u(0)} - u_{\bar{A}_3}^{A_2} u_{\bar{A}_1}^{2A_1} u_X^{1E_u(0)} - u_{A_2}^{2A_1} u_{\bar{A}_4}^{A_2} u_X^{1E_u(1)} + u_{A_2}^{A_2} u_{\bar{A}_4}^{2A_1} u_X^{1E_u(1)} \\
& - u_{A_3}^{A_2} u_X^{1E_u(0)} u_{A_1}^{2A_1} + u_{A_3}^{2A_1} u_X^{1E_u(0)} u_{A_1}^{A_2} - u_{A_5}^{2A_1} u_{A_1}^{A_2} u_{X_2}^{1E_u(1)} + u_{A_5}^{A_2} u_{A_1}^{1E_u(1)} u_{X_2}^{2A_1} + u_{X_1}^{1E_u(1)} u_{A_4}^{A_2} u_{\bar{A}_5}^{2A_1} \\
& - u_{X_1}^{1E_u(1)} u_{A_4}^{2A_1} u_{\bar{A}_5}^{A_2} - u_{X_1}^{1E_u(0)} u_{\bar{A}_4}^{2A_1} u_{\bar{A}_2}^{A_2} + u_{X_1}^{1E_u(0)} u_{\bar{A}_4}^{A_2} u_{\bar{A}_2}^{2A_1} - u_{A_3}^{2A_1} u_{X_2}^{1E_u(0)} u_{\bar{A}_1}^{A_2} + u_{A_3}^{A_2} u_{X_2}^{1E_u(0)} u_{\bar{A}_1}^{2A_1} \\
& + u_{A_3}^{A_2} u_{X_2}^{1E_u(0)} u_{A_1}^{2A_1} - u_{A_3}^{2A_1} u_{X_2}^{1E_u(0)} u_{A_1}^{A_2} - u_{X_1}^{1E_u(0)} u_{A_2}^{2A_1} u_{A_4}^{A_2} + u_{X_1}^{1E_u(0)} u_{A_2}^{A_2} u_{A_4}^{2A_1}) \\
& +d_{A_3 X_2 \bar{A}_1}^{2A_1 1E_u B_1} (-u_{X_2}^{1E_u(1)} u_{\bar{A}}^{B_1} u_{\bar{A}_5}^{2A_1} + u_{X_2}^{1E_u(1)} u_{\bar{A}}^{2A_1} u_{\bar{A}_5}^{B_1} - u_{X_1}^{1E_u(1)} u_{A_5}^{2A_1} u_{\bar{A}}^{B_1} + u_{X_1}^{1E_u(1)} u_{A_5}^{B_1} u_{\bar{A}}^{2A_1} - u_X^{1E_u(1)} u_{\bar{A}_2}^{B_1} u_{A_4}^{2A_1} \\
& + u_X^{1E_u(1)} u_{\bar{A}_2}^{2A_1} u_{A_4}^{B_1} + u_{\bar{A}_3}^{2A_1} u_{\bar{A}_1}^{B_1} u_X^{1E_u(0)} - u_{\bar{A}_3}^{B_1} u_{\bar{A}_1}^{2A_1} u_X^{1E_u(0)} + u_{A_2}^{2A_1} u_{\bar{A}_4}^{B_1} u_X^{1E_u(1)} - u_{A_2}^{B_1} u_{\bar{A}_4}^{2A_1} u_X^{1E_u(1)} \\
& - u_{A_3}^{B_1} u_X^{1E_u(0)} u_{A_1}^{2A_1} + u_{A_3}^{2A_1} u_X^{1E_u(0)} u_{A_1}^{B_1} - u_{A_5}^{2A_1} u_{A_1}^{B_1} u_{X_2}^{1E_u(1)} + u_{A_5}^{B_1} u_{A_1}^{2A_1} u_{X_2}^{1E_u(1)} - u_{X_1}^{1E_u(1)} u_{A_4}^{B_1} u_{\bar{A}_5}^{2A_1} \\
& + u_{X_1}^{1E_u(1)} u_{A_4}^{2A_1} u_{\bar{A}_5}^{B_1} - u_{X_1}^{1E_u(0)} u_{\bar{A}_4}^{2A_1} u_{\bar{A}_2}^{B_1} + u_{X_1}^{1E_u(0)} u_{\bar{A}_4}^{B_1} u_{\bar{A}_2}^{2A_1} + u_{A_3}^{2A_1} u_{X_2}^{1E_u(0)} u_{\bar{A}_1}^{B_1} - u_{A_3}^{B_1} u_{X_2}^{1E_u(0)} u_{\bar{A}_1}^{2A_1} \\
& - u_{\bar{A}_3}^{B_1} u_{X_2}^{1E_u(0)} u_{A_1}^{2A_1} + u_{\bar{A}_3}^{2A_1} u_{X_2}^{1E_u(0)} u_{A_1}^{B_1} - u_{X_1}^{1E_u(0)} u_{A_2}^{2A_1} u_{A_4}^{B_1} + u_{X_1}^{1E_u(0)} u_{A_2}^{B_1} u_{A_4}^{2A_1}) \\
& +d_{A_3 X_2 \bar{A}_1}^{2A_1 1E_u 1B_1} (-u_{X_2}^{1E_u(1)} u_{\bar{A}}^{1B_1} u_{\bar{A}_5}^{2A_1} + u_{X_2}^{1E_u(1)} u_{\bar{A}}^{2A_1} u_{\bar{A}_5}^{1B_1} - u_{X_1}^{1E_u(1)} u_{A_5}^{2A_1} u_{\bar{A}}^{1B_1} + u_{X_1}^{1E_u(1)} u_{A_5}^{1B_1} u_{\bar{A}}^{2A_1} - u_X^{1E_u(1)} u_{\bar{A}_2}^{1B_1} u_{A_4}^{2A_1} \\
& + u_X^{1E_u(1)} u_{\bar{A}_2}^{2A_1} u_{A_4}^{1B_1} + u_{\bar{A}_3}^{2A_1} u_{\bar{A}_1}^{1B_1} u_X^{1E_u(0)} - u_{\bar{A}_3}^{1B_1} u_{\bar{A}_1}^{2A_1} u_X^{1E_u(0)} + u_{A_2}^{2A_1} u_{\bar{A}_4}^{1B_1} u_X^{1E_u(1)} - u_{A_2}^{1B_1} u_{\bar{A}_4}^{2A_1} u_X^{1E_u(1)} \\
& - u_{A_3}^{1B_1} u_X^{1E_u(0)} u_{A_1}^{2A_1} + u_{A_3}^{2A_1} u_X^{1E_u(0)} u_{A_1}^{1B_1} - u_{A_5}^{2A_1} u_{A_1}^{1B_1} u_{X_2}^{1E_u(1)} + u_{A_5}^{1B_1} u_{A_1}^{2A_1} u_{X_2}^{1E_u(1)} - u_{X_1}^{1E_u(1)} u_{A_4}^{1B_1} u_{\bar{A}_5}^{2A_1} \\
& + u_{X_1}^{1E_u(1)} u_{A_4}^{2A_1} u_{\bar{A}_5}^{1B_1} - u_{X_1}^{1E_u(0)} u_{\bar{A}_4}^{2A_1} u_{\bar{A}_2}^{1B_1} + u_{X_1}^{1E_u(0)} u_{\bar{A}_4}^{1B_1} u_{\bar{A}_2}^{2A_1} + u_{A_3}^{2A_1} u_{X_2}^{1E_u(0)} u_{\bar{A}_1}^{1B_1} - u_{A_3}^{1B_1} u_{X_2}^{1E_u(0)} u_{\bar{A}_1}^{2A_1} \\
& - u_{\bar{A}_3}^{1B_1} u_{X_2}^{1E_u(0)} u_{A_1}^{2A_1} + u_{\bar{A}_3}^{2A_1} u_{X_2}^{1E_u(0)} u_{A_1}^{1B_1} - u_{X_1}^{1E_u(0)} u_{A_2}^{2A_1} u_{A_4}^{1B_1} + u_{X_1}^{1E_u(0)} u_{A_2}^{1B_1} u_{A_4}^{2A_1}) \\
& +d_{A_3 X_2 \bar{A}_1}^{2A_1 1E_u 2B_1} (-u_{X_2}^{1E_u(1)} u_{\bar{A}}^{2B_1} u_{\bar{A}_5}^{2A_1} + u_{X_2}^{1E_u(1)} u_{\bar{A}}^{2A_1} u_{\bar{A}_5}^{2B_1} - u_{X_1}^{1E_u(1)} u_{A_5}^{2A_1} u_{\bar{A}}^{2B_1} + u_{X_1}^{1E_u(1)} u_{A_5}^{2B_1} u_{\bar{A}}^{2A_1} - u_X^{1E_u(1)} u_{\bar{A}_2}^{2B_1} u_{A_4}^{2A_1} \\
& + u_X^{1E_u(1)} u_{\bar{A}_2}^{2A_1} u_{A_4}^{2B_1} + u_{\bar{A}_3}^{2A_1} u_{\bar{A}_1}^{2B_1} u_X^{1E_u(0)} - u_{\bar{A}_3}^{2B_1} u_{\bar{A}_1}^{2A_1} u_X^{1E_u(0)} + u_{A_2}^{2A_1} u_{\bar{A}_4}^{2B_1} u_X^{1E_u(1)} - u_{A_2}^{2B_1} u_{\bar{A}_4}^{2A_1} u_X^{1E_u(1)} \\
& - u_{A_3}^{2B_1} u_X^{1E_u(0)} u_{A_1}^{2A_1} + u_{A_3}^{2A_1} u_X^{1E_u(0)} u_{A_1}^{2B_1} - u_{A_5}^{2A_1} u_{A_1}^{2B_1} u_{X_2}^{1E_u(1)} + u_{A_5}^{2B_1} u_{A_1}^{2A_1} u_{X_2}^{1E_u(1)} - u_{X_1}^{1E_u(1)} u_{A_4}^{2B_1} u_{\bar{A}_5}^{2A_1} \\
& + u_{X_1}^{1E_u(1)} u_{A_4}^{2A_1} u_{\bar{A}_5}^{2B_1} - u_{X_1}^{1E_u(0)} u_{\bar{A}_4}^{2A_1} u_{\bar{A}_2}^{2B_1} + u_{X_1}^{1E_u(0)} u_{\bar{A}_4}^{2B_1} u_{\bar{A}_2}^{2A_1} + u_{A_3}^{2A_1} u_{X_2}^{1E_u(0)} u_{\bar{A}_1}^{2B_1} - u_{A_3}^{2B_1} u_{X_2}^{1E_u(0)} u_{\bar{A}_1}^{2A_1} \\
& - u_{\bar{A}_3}^{2B_1} u_{X_2}^{1E_u(0)} u_{A_1}^{2A_1} + u_{\bar{A}_3}^{2A_1} u_{X_2}^{1E_u(0)} u_{A_1}^{2B_1} - u_{X_1}^{1E_u(0)} u_{A_2}^{2B_1} u_{A_4}^{2A_1} + u_{X_1}^{1E_u(0)} u_{A_2}^{2A_1} u_{A_4}^{2B_1}) \\
& +d_{A_3 X_2 \bar{A}_1}^{A_2 A_1 g A_2} (u_{X_2}^{A_1 g} u_{\bar{A}}^{A_2} u_{\bar{A}_5}^{A_2} + u_{X_1}^{A_1 g} u_{A_5}^{A_2} u_{\bar{A}}^{A_2} + u_X^{A_1 g} u_{A_2}^{A_2} u_{A_4}^{A_2} + u_{\bar{A}_3}^{A_2} u_{\bar{A}_1}^{A_2} u_X^{A_1 g} + u_{A_2}^{A_2} u_{\bar{A}_4}^{A_2} u_X^{A_1 g} \\
& + u_{A_3}^{A_2} u_X^{A_1 g} u_{A_1}^{A_2} + u_{A_5}^{A_2} u_{A_1}^{A_2} u_{X_2}^{A_1 g} + u_{X_1}^{A_1 g} u_{A_4}^{A_2} u_{\bar{A}_5}^{A_2} + u_{X_1}^{A_1 g} u_{\bar{A}_4}^{A_2} u_{\bar{A}_2}^{A_2} + u_{A_3}^{A_2} u_{X_2}^{A_1 g} u_{\bar{A}_1}^{A_2} \\
& + u_{\bar{A}_3}^{A_2} u_{X_2}^{A_1 g} u_{A_1}^{A_2} + u_{X_1}^{A_1 g} u_{A_2}^{A_2} u_{A_4}^{A_2}) \\
& +d_{A_3 X_2 \bar{A}_1}^{A_2 A_1 g B_1} (u_{X_2}^{A_1 g} u_{\bar{A}}^{B_1} u_{\bar{A}_5}^{A_2} + u_{X_2}^{A_1 g} u_{\bar{A}}^{A_2} u_{\bar{A}_5}^{B_1} - u_{X_1}^{A_1 g} u_{A_5}^{A_2} u_{\bar{A}}^{B_1} - u_{X_1}^{A_1 g} u_{A_5}^{B_1} u_{\bar{A}}^{A_2} - u_X^{A_1 g} u_{\bar{A}_2}^{B_1} u_{A_4}^{A_2}
\end{aligned}$$



[illegible]

$$\begin{aligned}
& +d_{A_3 X_2 \bar{A}_1}^{A_2 E_g \bar{2} B_1} (-u_{X_2}^{E_g(1)} u_{\bar{A}}^{2 B_1} u_{A_5}^{A_2} + u_{X_2}^{E_g(1)} u_{\bar{A}}^{A_2} u_{A_5}^{2 B_1} - u_{X_1}^{E_g(1)} u_{A_5}^{A_2} u_{\bar{A}}^{2 B_1} + u_{X_1}^{E_g(1)} u_{A_5}^{2 B_1} u_{\bar{A}}^{A_2} - u_{X_1}^{E_g(1)} u_{A_5}^{2 B_1} u_{\bar{A}}^{A_2} \\
& + u_X^{E_g(1)} u_{\bar{A}_2}^{A_2} u_{A_4}^{2 B_1} + u_{A_3}^{A_2} u_{\bar{A}_1}^{2 B_1} u_X^{E_g(0)} - u_{\bar{A}_3}^{2 B_1} u_{\bar{A}_1}^{A_2} u_X^{E_g(0)} + u_{A_2}^{A_2} u_{\bar{A}_4}^{2 B_1} u_X^{E_g(1)} - u_{A_2}^{2 B_1} u_{\bar{A}_4}^{A_2} u_X^{E_g(1)} \\
& - u_{A_3}^{2 B_1} u_X^{E_g(0)} u_{A_1}^{A_2} + u_{A_3}^{A_2} u_X^{E_g(0)} u_{A_1}^{2 B_1} - u_{A_5}^{A_2} u_{X_2}^{2 B_1} u_{A_1}^{E_g(1)} + u_{A_5}^{2 B_1} u_{A_1}^{A_2} u_{X_2}^{E_g(1)} - u_{X_1}^{E_g(1)} u_{A_1}^{2 B_1} u_{A_5}^{A_2} \\
& + u_{X_1}^{E_g(1)} u_{A_1}^{A_2} u_{A_5}^{2 B_1} - u_{X_1}^{E_g(0)} u_{A_4}^{A_2} u_{A_2}^{2 B_1} + u_{X_1}^{E_g(0)} u_{A_4}^{2 B_1} u_{A_2}^{A_2} + u_{A_3}^{A_2} u_{X_2}^{E_g(0)} u_{A_1}^{2 B_1} - u_{A_3}^{2 B_1} u_{X_2}^{E_g(0)} u_{A_1}^{A_2} \\
& - u_{\bar{A}_3}^{2 B_1} u_X^{E_g(0)} u_{A_1}^{A_2} + u_{\bar{A}_3}^{A_2} u_X^{E_g(0)} u_{A_1}^{2 B_1} - u_{X_1}^{E_g(0)} u_{A_2}^{A_2} u_{A_4}^{2 B_1} + u_{X_1}^{E_g(0)} u_{A_2}^{2 B_1} u_{A_4}^{A_2}) \\
& +d_{A_3 X_2 \bar{A}_1}^{A_2 A_{2u} A_2} (-u_{X_2}^{A_{2u}} u_{\bar{A}}^{A_2} u_{A_5}^{A_2} + u_{X_1}^{A_{2u}} u_{A_5}^{A_2} u_{\bar{A}}^{A_2} - u_X^{A_{2u}} u_{A_2}^{A_2} u_{A_4}^{A_2} + u_{\bar{A}_3}^{A_2} u_{\bar{A}_1}^{A_{2u}} u_X^{A_2} + u_{A_2}^{A_2} u_{A_4}^{A_{2u}} u_X^{A_2} \\
& - u_{A_3}^{A_2} u_X^{A_{2u}} u_{A_1}^{A_2} + u_{A_5}^{A_2} u_{A_1}^{A_{2u}} u_{X_2}^{A_2} - u_{X_1}^{A_{2u}} u_{A_1}^{A_2} u_{A_5}^{A_2} + u_{X_1}^{A_{2u}} u_{A_4}^{A_2} u_{A_2}^{A_2} + u_{A_3}^{A_2} u_{X_2}^{A_{2u}} u_{A_1}^{A_2} \\
& - u_{A_3}^{A_2} u_{X_2}^{A_{2u}} u_{A_1}^{A_2} - u_{X_1}^{A_{2u}} u_{A_2}^{A_2} u_{A_4}^{A_2}) \\
& +d_{A_3 X_2 \bar{A}_1}^{A_2 A_{2u} B_1} (-u_{X_2}^{A_{2u}} u_{\bar{A}}^{B_1} u_{A_5}^{A_2} - u_{X_2}^{A_{2u}} u_{A_5}^{A_2} u_{\bar{A}}^{B_1} - u_{X_1}^{A_{2u}} u_{A_5}^{A_2} u_{\bar{A}}^{B_1} - u_{X_1}^{A_{2u}} u_{A_5}^{B_1} u_{\bar{A}}^{A_2} + u_X^{A_{2u}} u_{\bar{A}_2}^{B_1} u_{A_4}^{A_2} \\
& + u_X^{A_{2u}} u_{\bar{A}_2}^{B_1} u_{A_4}^{A_2} + u_{A_3}^{A_2} u_{\bar{A}_1}^{B_1} u_X^{A_{2u}} + u_{\bar{A}_3}^{B_1} u_{\bar{A}_1}^{A_2} u_X^{A_{2u}} - u_{A_2}^{A_2} u_{\bar{A}_4}^{B_1} u_X^{A_{2u}} - u_{A_2}^{B_1} u_{\bar{A}_4}^{A_2} u_X^{A_{2u}} \\
& - u_{A_3}^{B_1} u_X^{A_{2u}} u_{A_1}^{A_2} - u_{A_3}^{A_2} u_X^{A_{2u}} u_{A_1}^{B_1} + u_{A_5}^{A_2} u_{A_1}^{B_1} u_{X_2}^{A_{2u}} + u_{A_5}^{B_1} u_{A_1}^{A_2} u_{X_2}^{A_{2u}} + u_{X_1}^{A_{2u}} u_{A_1}^{B_1} u_{A_5}^{A_2} \\
& + u_{X_1}^{A_{2u}} u_{A_1}^{A_2} u_{A_5}^{B_1} + u_{X_1}^{A_{2u}} u_{A_4}^{B_1} u_{A_2}^{A_2} - u_{A_3}^{A_2} u_{X_2}^{B_1} u_{A_1}^{A_2} - u_{A_3}^{B_1} u_{X_2}^{A_{2u}} u_{A_1}^{A_2} \\
& + u_{\bar{A}_3}^{B_1} u_{X_2}^{A_{2u}} u_{A_1}^{A_2} + u_{\bar{A}_3}^{A_2} u_{X_2}^{B_1} u_{A_1}^{A_2} - u_{X_1}^{A_{2u}} u_{A_2}^{B_1} u_{A_4}^{A_2} - u_{X_1}^{A_{2u}} u_{A_2}^{A_2} u_{A_4}^{B_1}) \\
& +d_{A_3 X_2 \bar{A}_1}^{A_2 A_{2u} \bar{1} B_1} (-u_{X_2}^{A_{2u}} u_{\bar{A}}^{\bar{1} B_1} u_{A_5}^{A_2} - u_{X_2}^{A_{2u}} u_{\bar{A}}^{A_2} u_{A_5}^{\bar{1} B_1} - u_{X_1}^{A_{2u}} u_{A_5}^{A_2} u_{\bar{A}}^{\bar{1} B_1} - u_{X_1}^{A_{2u}} u_{A_5}^{\bar{1} B_1} u_{\bar{A}}^{A_2} + u_X^{A_{2u}} u_{\bar{A}_2}^{\bar{1} B_1} u_{A_4}^{A_2} \\
& + u_X^{A_{2u}} u_{\bar{A}_2}^{A_2} u_{A_4}^{\bar{1} B_1} + u_{A_3}^{A_2} u_{\bar{A}_1}^{\bar{1} B_1} u_X^{A_{2u}} + u_{\bar{A}_3}^{\bar{1} B_1} u_{\bar{A}_1}^{A_2} u_X^{A_{2u}} - u_{A_2}^{A_2} u_{\bar{A}_4}^{\bar{1} B_1} u_X^{A_{2u}} - u_{A_2}^{\bar{1} B_1} u_{\bar{A}_4}^{A_2} u_X^{A_{2u}} \\
& - u_{A_3}^{\bar{1} B_1} u_X^{A_{2u}} u_{A_1}^{A_2} - u_{A_3}^{A_2} u_X^{A_{2u}} u_{A_1}^{\bar{1} B_1} + u_{A_5}^{A_2} u_{A_1}^{\bar{1} B_1} u_{X_2}^{A_{2u}} + u_{A_5}^{\bar{1} B_1} u_{A_1}^{A_2} u_{X_2}^{A_{2u}} + u_{X_1}^{A_{2u}} u_{A_1}^{\bar{1} B_1} u_{A_5}^{A_2} \\
& + u_{X_1}^{A_{2u}} u_{A_1}^{A_2} u_{A_5}^{\bar{1} B_1} + u_{X_1}^{A_{2u}} u_{A_4}^{A_2} u_{A_2}^{\bar{1} B_1} + u_{X_1}^{A_{2u}} u_{A_4}^{\bar{1} B_1} u_{A_2}^{A_2} - u_{A_3}^{A_2} u_{X_2}^{\bar{1} B_1} u_{A_1}^{A_2} - u_{A_3}^{\bar{1} B_1} u_{X_2}^{A_{2u}} u_{A_1}^{A_2} \\
& + u_{\bar{A}_3}^{\bar{1} B_1} u_{X_2}^{A_{2u}} u_{A_1}^{A_2} + u_{\bar{A}_3}^{A_2} u_{X_2}^{\bar{1} B_1} u_{A_1}^{A_2} - u_{X_1}^{A_{2u}} u_{A_2}^{\bar{1} B_1} u_{A_4}^{A_2} - u_{X_1}^{A_{2u}} u_{A_2}^{A_2} u_{A_4}^{\bar{1} B_1}) \\
& +d_{A_3 X_2 \bar{A}_1}^{A_2 A_{2u} \bar{2} B_1} (-u_{X_2}^{A_{2u}} u_{\bar{A}}^{\bar{2} B_1} u_{A_5}^{A_2} - u_{X_2}^{A_{2u}} u_{\bar{A}}^{A_2} u_{A_5}^{\bar{2} B_1} - u_{X_1}^{A_{2u}} u_{A_5}^{A_2} u_{\bar{A}}^{\bar{2} B_1} - u_{X_1}^{A_{2u}} u_{A_5}^{\bar{2} B_1} u_{\bar{A}}^{A_2} + u_X^{A_{2u}} u_{\bar{A}_2}^{\bar{2} B_1} u_{A_4}^{A_2} \\
& + u_X^{A_{2u}} u_{\bar{A}_2}^{A_2} u_{A_4}^{\bar{2} B_1} + u_{\bar{A}_3}^{A_2} u_{\bar{A}_1}^{\bar{2} B_1} u_X^{A_{2u}} + u_{\bar{A}_3}^{\bar{2} B_1} u_{\bar{A}_1}^{A_2} u_X^{A_{2u}} - u_{A_2}^{A_2} u_{\bar{A}_4}^{\bar{2} B_1} u_X^{A_{2u}} - u_{A_2}^{\bar{2} B_1} u_{\bar{A}_4}^{A_2} u_X^{A_{2u}} \\
& - u_{A_3}^{\bar{2} B_1} u_X^{A_{2u}} u_{A_1}^{A_2} - u_{A_3}^{A_2} u_X^{A_{2u}} u_{A_1}^{\bar{2} B_1} + u_{A_5}^{A_2} u_{A_1}^{\bar{2} B_1} u_{X_2}^{A_{2u}} + u_{A_5}^{\bar{2} B_1} u_{A_1}^{A_2} u_{X_2}^{A_{2u}} + u_{X_1}^{A_{2u}} u_{A_1}^{\bar{2} B_1} u_{A_5}^{A_2} \\
& + u_{X_1}^{A_{2u}} u_{A_1}^{A_2} u_{A_5}^{\bar{2} B_1} + u_{X_1}^{A_{2u}} u_{A_4}^{A_2} u_{A_2}^{\bar{2} B_1} + u_{X_1}^{A_{2u}} u_{A_4}^{\bar{2} B_1} u_{A_2}^{A_2} - u_{A_3}^{A_2} u_{X_2}^{\bar{2} B_1} u_{A_1}^{A_2} - u_{A_3}^{\bar{2} B_1} u_{X_2}^{A_{2u}} u_{A_1}^{A_2} \\
& + u_{\bar{A}_3}^{\bar{2} B_1} u_{X_2}^{A_{2u}} u_{A_1}^{A_2} + u_{\bar{A}_3}^{A_2} u_{X_2}^{\bar{2} B_1} u_{A_1}^{A_2} - u_{X_1}^{A_{2u}} u_{A_2}^{\bar{2} B_1} u_{A_4}^{A_2} - u_{X_1}^{A_{2u}} u_{A_2}^{A_2} u_{A_4}^{\bar{2} B_1}) \\
& +d_{A_3 X_2 \bar{A}_1}^{B_2 B_{1u} A_2} (u_{X_2}^{B_{1u}} u_{\bar{A}}^{B_2} u_{A_5}^{A_2} + u_{X_2}^{B_{1u}} u_{\bar{A}}^{A_2} u_{A_5}^{B_2} + u_{X_1}^{B_{1u}} u_{A_5}^{A_2} u_{\bar{A}}^{B_2} + u_{X_1}^{B_{1u}} u_{A_5}^{B_2} u_{\bar{A}}^{A_2} + u_X^{B_{1u}} u_{\bar{A}_2}^{B_2} u_{A_4}^{A_2} \\
& + u_X^{B_{1u}} u_{\bar{A}_2}^{A_2} u_{A_4}^{B_2} + u_{A_3}^{A_2} u_{\bar{A}_1}^{B_2} u_X^{B_{1u}} + u_{\bar{A}_3}^{B_2} u_{\bar{A}_1}^{A_2} u_X^{B_{1u}} + u_{A_2}^{A_2} u_{\bar{A}_4}^{B_{1u}} u_X^{B_{1u}} + u_{A_2}^{B_2} u_{\bar{A}_4}^{A_2} u_X^{B_{1u}} \\
& + u_{A_3}^{B_2} u_X^{B_{1u}} u_{A_1}^{A_2} + u_{A_3}^{A_2} u_X^{B_{1u}} u_{A_1}^{B_2} + u_{A_5}^{A_2} u_{A_1}^{B_2} u_{X_2}^{B_{1u}} + u_{A_5}^{B_2} u_{A_1}^{A_2} u_{X_2}^{B_{1u}} + u_{X_1}^{B_{1u}} u_{A_1}^{B_2} u_{A_5}^{A_2} \\
& + u_{X_1}^{B_{1u}} u_{A_1}^{A_2} u_{A_5}^{B_2} + u_{X_1}^{B_{1u}} u_{A_4}^{A_2} u_{A_2}^{B_2} + u_{X_1}^{B_{1u}} u_{A_4}^{B_2} u_{A_2}^{A_2} + u_{A_3}^{A_2} u_{X_2}^{B_{1u}} u_{A_1}^{B_2} + u_{A_3}^{B_2} u_{X_2}^{B_{1u}} u_{A_1}^{A_2} \\
& + u_{\bar{A}_3}^{B_2} u_{X_2}^{B_{1u}} u_{A_1}^{A_2} + u_{\bar{A}_3}^{A_2} u_{X_2}^{B_{1u}} u_{A_1}^{B_2} + u_{X_1}^{B_{1u}} u_{A_2}^{B_2} u_{A_4}^{A_2} + u_{X_1}^{B_{1u}} u_{A_2}^{A_2} u_{A_4}^{B_2}) \\
& +d_{A_3 X_2 \bar{A}_1}^{\bar{1} B_2 B_{1u} A_2} (u_{X_2}^{B_{1u}} u_{\bar{A}}^{\bar{1} B_2} u_{A_5}^{A_2} + u_{X_2}^{B_{1u}} u_{\bar{A}}^{A_2} u_{A_5}^{\bar{1} B_2} + u_{X_1}^{B_{1u}} u_{A_5}^{A_2} u_{\bar{A}}^{\bar{1} B_2} + u_{X_1}^{B_{1u}} u_{A_5}^{\bar{1} B_2} u_{\bar{A}}^{A_2} + u_X^{B_{1u}} u_{\bar{A}_2}^{\bar{1} B_2} u_{A_4}^{A_2} \\
& + u_X^{B_{1u}} u_{\bar{A}_2}^{A_2} u_{A_4}^{\bar{1} B_2} + u_{\bar{A}_3}^{A_2} u_{\bar{A}_1}^{\bar{1} B_2} u_X^{B_{1u}} + u_{\bar{A}_3}^{\bar{1} B_2} u_{\bar{A}_1}^{A_2} u_X^{B_{1u}} + u_{A_2}^{A_2} u_{\bar{A}_4}^{\bar{1} B_2} u_X^{B_{1u}} + u_{A_2}^{\bar{1} B_2} u_{\bar{A}_4}^{A_2} u_X^{B_{1u}} \\
& + u_{A_3}^{\bar{1} B_2} u_X^{B_{1u}} u_{A_1}^{A_2} + u_{A_3}^{A_2} u_X^{B_{1u}} u_{A_1}^{\bar{1} B_2} + u_{A_5}^{A_2} u_{A_1}^{\bar{1} B_2} u_{X_2}^{B_{1u}} + u_{A_5}^{\bar{1} B_2} u_{A_1}^{A_2} u_{X_2}^{B_{1u}} + u_{X_1}^{B_{1u}} u_{A_1}^{\bar{1} B_2} u_{A_5}^{A_2} \\
& + u_{X_1}^{B_{1u}} u_{A_1}^{A_2} u_{A_5}^{\bar{1} B_2} + u_{X_1}^{B_{1u}} u_{A_4}^{A_2} u_{A_2}^{\bar{1} B_2} + u_{X_1}^{B_{1u}} u_{A_4}^{\bar{1} B_2} u_{A_2}^{A_2} + u_{A_3}^{A_2} u_{X_2}^{\bar{1} B_2} u_{A_1}^{A_2} + u_{A_3}^{\bar{1} B_2} u_{X_2}^{B_{1u}} u_{A_1}^{A_2} \\
& + u_{\bar{A}_3}^{\bar{1} B_2} u_{X_2}^{B_{1u}} u_{A_1}^{A_2} + u_{\bar{A}_3}^{A_2} u_{X_2}^{\bar{1} B_2} u_{A_1}^{A_2} + u_{X_1}^{B_{1u}} u_{A_2}^{\bar{1} B_2} u_{A_4}^{A_2} + u_{X_1}^{B_{1u}} u_{A_2}^{A_2} u_{A_4}^{\bar{1} B_2}) \\
& +d_{A_3 X_2 \bar{A}_1}^{A_2 E_u B_1} (u_{X_2}^{E_u(0)} u_{\bar{A}}^{B_1} u_{A_5}^{A_2} - u_{X_2}^{E_u(0)} u_{\bar{A}}^{A_2} u_{A_5}^{B_1} + u_{X_1}^{E_u(0)} u_{A_5}^{A_2} u_{\bar{A}}^{B_1} - u_{X_1}^{E_u(0)} u_{A_5}^{B_1} u_{\bar{A}}^{A_2} - u_X^{E_u(0)} u_{\bar{A}_2}^{B_1} u_{A_4}^{A_2} \\
& + u_X^{E_u(0)} u_{\bar{A}_2}^{A_2} u_{A_4}^{B_1} + u_{A_3}^{A_2} u_{\bar{A}_1}^{B_1} u_X^{E_u(1)} - u_{\bar{A}_3}^{B_1} u_{\bar{A}_1}^{A_2} u_X^{E_u(1)} - u_{A_2}^{A_2} u_{\bar{A}_4}^{B_1} u_X^{E_u(0)} + u_{A_2}^{B_1} u_{\bar{A}_4}^{A_2} u_X^{E_u(0)})
\end{aligned}$$



$$\begin{aligned}
& + u_X^{1E_u(0)} u_{\bar{A}_2}^{2B_1} u_{A_4}^{2B_1} + u_{\bar{A}_3}^{2B_1} u_{\bar{A}_1}^{2B_1} u_X^{1E_u(1)} - u_{\bar{A}_3}^{2B_1} u_{\bar{A}_1}^{2B_1} u_X^{1E_u(1)} - u_{A_2}^{2B_1} u_{\bar{A}_4}^{2B_1} u_X^{1E_u(0)} + u_{A_2}^{2B_1} u_{\bar{A}_4}^{2B_1} u_X^{1E_u(0)} \\
& + u_{A_3}^{2B_1} u_X^{1E_u(1)} u_{A_1}^{A_2} - u_{A_3}^{2B_1} u_X^{1E_u(1)} u_{A_1}^{2B_1} - u_{A_5}^{2B_1} u_A^{2B_1} u_{X_2}^{1E_u(0)} + u_{A_5}^{2B_1} u_A^{2B_1} u_{X_2}^{1E_u(0)} - u_{X_1}^{1E_u(0)} u_A^{2B_1} u_{\bar{A}_5}^{A_2} \\
& + u_{X_1}^{1E_u(0)} u_A^{2B_1} u_{\bar{A}_5}^{2B_1} - u_{X_1}^{1E_u(1)} u_{\bar{A}_4}^{A_2} u_{\bar{A}_5}^{2B_1} + u_{X_1}^{1E_u(1)} u_{\bar{A}_4}^{2B_1} u_{\bar{A}_2}^{A_2} - u_{A_2}^{2B_1} u_X^{1E_u(1)} u_{\bar{A}_1}^{2B_1} + u_{A_3}^{2B_1} u_{X_2}^{1E_u(1)} u_{\bar{A}_1}^{A_2} \\
& - u_{\bar{A}_3}^{2B_1} u_{X_2}^{1E_u(1)} u_{A_1}^{A_2} + u_{\bar{A}_3}^{2B_1} u_{X_2}^{1E_u(1)} u_{A_1}^{2B_1} + u_{X_1}^{1E_u(1)} u_{A_2}^{2B_1} u_{A_4}^{A_2} - u_{X_1}^{1E_u(1)} u_{A_2}^{2B_1} u_{A_4}^{2B_1} \\
& + d_{A_3 X_2 \bar{A}_1}^{B_2 1E_u A_2} (-u_{X_2}^{1E_u(1)} u_{\bar{A}}^{B_2} u_{\bar{A}_5}^{A_2} + u_{X_2}^{1E_u(1)} u_{\bar{A}}^{A_2} u_{\bar{A}_5}^{B_2} - u_{X_1}^{1E_u(1)} u_{A_5}^{A_2} u_{\bar{A}}^{B_2} + u_{X_1}^{1E_u(1)} u_{A_5}^{B_2} u_{\bar{A}}^{A_2} - u_X^{1E_u(1)} u_{\bar{A}_2}^{B_2} u_{A_4}^{A_2} \\
& + u_X^{1E_u(1)} u_{\bar{A}_2}^{A_2} u_{A_4}^{B_2} + u_{\bar{A}_3}^{A_2} u_{\bar{A}_1}^{B_2} u_X^{1E_u(0)} - u_{\bar{A}_3}^{B_2} u_{\bar{A}_1}^{A_2} u_X^{1E_u(0)} + u_{A_2}^{A_2} u_{\bar{A}_4}^{B_2} u_X^{1E_u(1)} - u_{A_2}^{B_2} u_{\bar{A}_4}^{A_2} u_X^{1E_u(1)} \\
& - u_{A_3}^{B_2} u_X^{1E_u(0)} u_{A_1}^{A_2} + u_{A_3}^{A_2} u_X^{1E_u(0)} u_{A_1}^{B_2} - u_{A_5}^{A_2} u_{A_2}^{B_2} u_{X_2}^{1E_u(1)} + u_{A_5}^{B_2} u_{A_2}^{A_2} u_{X_2}^{1E_u(1)} - u_{X_1}^{1E_u(1)} u_A^{B_2} u_{\bar{A}_5}^{A_2} \\
& + u_X^{1E_u(1)} u_A^{A_2} u_{\bar{A}_5}^{B_2} - u_{X_1}^{1E_u(0)} u_{\bar{A}_4}^{A_2} u_{\bar{A}_2}^{B_2} + u_{X_1}^{1E_u(0)} u_{\bar{A}_4}^{B_2} u_{\bar{A}_2}^{A_2} + u_{A_3}^{A_2} u_{X_2}^{1E_u(0)} u_{\bar{A}_1}^{B_2} - u_{A_3}^{B_2} u_{X_2}^{1E_u(0)} u_{\bar{A}_1}^{A_2} \\
& - u_{\bar{A}_3}^{B_2} u_{X_2}^{1E_u(0)} u_{A_1}^{A_2} + u_{\bar{A}_3}^{A_2} u_{X_2}^{1E_u(0)} u_{A_1}^{B_2} - u_{X_1}^{1E_u(0)} u_{A_2}^{B_2} u_{A_4}^{A_2} + u_{X_1}^{1E_u(0)} u_{A_2}^{A_2} u_{A_4}^{B_2} \\
& + d_{A_3 X_2 \bar{A}_1}^{B_2 1E_u A_2} (-u_{X_2}^{1E_u(1)} u_{\bar{A}}^{1B_2} u_{\bar{A}_5}^{A_2} + u_{X_2}^{1E_u(1)} u_{\bar{A}}^{A_2} u_{\bar{A}_5}^{1B_2} - u_{X_1}^{1E_u(1)} u_{A_5}^{A_2} u_{\bar{A}}^{1B_2} + u_{X_1}^{1E_u(1)} u_{A_5}^{1B_2} u_{\bar{A}}^{A_2} - u_X^{1E_u(1)} u_{\bar{A}_2}^{1B_2} u_{A_4}^{A_2} \\
& + u_X^{1E_u(1)} u_{\bar{A}_2}^{A_2} u_{A_4}^{1B_2} + u_{\bar{A}_3}^{A_2} u_{\bar{A}_1}^{1B_2} u_X^{1E_u(0)} - u_{\bar{A}_3}^{1B_2} u_{\bar{A}_1}^{A_2} u_X^{1E_u(0)} + u_{A_2}^{A_2} u_{\bar{A}_4}^{1B_2} u_X^{1E_u(1)} - u_{A_2}^{1B_2} u_{\bar{A}_4}^{A_2} u_X^{1E_u(1)} \\
& - u_{A_3}^{1B_2} u_X^{1E_u(0)} u_{A_1}^{A_2} + u_{A_3}^{A_2} u_X^{1E_u(0)} u_{A_1}^{1B_2} - u_{A_5}^{A_2} u_{A_2}^{1B_2} u_{X_2}^{1E_u(1)} + u_{A_5}^{1B_2} u_{A_2}^{A_2} u_{X_2}^{1E_u(1)} - u_{X_1}^{1E_u(1)} u_A^{1B_2} u_{\bar{A}_5}^{A_2} \\
& + u_{X_1}^{1E_u(1)} u_A^{A_2} u_{\bar{A}_5}^{1B_2} - u_{X_1}^{1E_u(0)} u_{\bar{A}_4}^{A_2} u_{\bar{A}_2}^{1B_2} + u_{X_1}^{1E_u(0)} u_{\bar{A}_4}^{1B_2} u_{\bar{A}_2}^{A_2} + u_{A_3}^{A_2} u_{X_2}^{1E_u(0)} u_{\bar{A}_1}^{1B_2} - u_{A_3}^{1B_2} u_{X_2}^{1E_u(0)} u_{\bar{A}_1}^{A_2} \\
& - u_{\bar{A}_3}^{1B_2} u_{X_2}^{1E_u(0)} u_{A_1}^{A_2} + u_{\bar{A}_3}^{A_2} u_{X_2}^{1E_u(0)} u_{A_1}^{1B_2} - u_{X_1}^{1E_u(0)} u_{A_2}^{1B_2} u_{A_4}^{A_2} + u_{X_1}^{1E_u(0)} u_{A_2}^{A_2} u_{A_4}^{1B_2} \\
& + d_{A_3 X_2 \bar{A}_1}^{B_1 A_1 g B_1} (u_{X_2}^{A_1 g} u_{\bar{A}}^{B_1} u_{\bar{A}_5}^{B_1} + u_{X_1}^{A_1 g} u_{A_5}^{B_1} u_{\bar{A}}^{B_1} + u_X^{A_1 g} u_{A_2}^{B_1} u_{A_4}^{B_1} + u_{\bar{A}_3}^{B_1} u_{\bar{A}_1}^{B_1} u_X^{A_1 g} + u_{A_2}^{B_1} u_{A_4}^{B_1} u_X^{A_1 g} \\
& + u_{A_3}^{B_1} u_X^{A_1 g} u_{A_1}^{B_1} + u_{A_5}^{B_1} u_A^{A_1 g} u_{X_2}^{B_1} + u_{X_1}^{A_1 g} u_A^{B_1} u_{\bar{A}_5}^{B_1} + u_{X_1}^{A_1 g} u_A^{B_1} u_{\bar{A}_2}^{B_1} + u_{A_3}^{B_1} u_{X_2}^{A_1 g} u_{\bar{A}_1}^{B_1} \\
& + u_{\bar{A}_3}^{B_1} u_{X_2}^{A_1 g} u_{A_1}^{B_1} + u_{X_1}^{A_1 g} u_{A_2}^{B_1} u_{A_4}^{B_1} \\
& + d_{A_3 X_2 \bar{A}_1}^{B_1 A_1 g 1B_1} (u_{X_2}^{A_1 g} u_{\bar{A}}^{1B_1} u_{\bar{A}_5}^{B_1} + u_{X_2}^{A_1 g} u_{\bar{A}}^{B_1} u_{\bar{A}_5}^{1B_1} + u_{X_1}^{A_1 g} u_{A_5}^{B_1} u_{\bar{A}}^{1B_1} + u_{X_1}^{A_1 g} u_{A_5}^{1B_1} u_{\bar{A}}^{B_1} + u_X^{A_1 g} u_{\bar{A}_2}^{1B_1} u_{A_4}^{B_1} \\
& + u_X^{A_1 g} u_{\bar{A}_2}^{B_1} u_{A_4}^{1B_1} + u_{\bar{A}_3}^{B_1} u_{\bar{A}_1}^{1B_1} u_X^{A_1 g} + u_{\bar{A}_3}^{1B_1} u_{\bar{A}_1}^{B_1} u_X^{A_1 g} + u_{A_2}^{B_1} u_{\bar{A}_4}^{1B_1} u_X^{A_1 g} + u_{A_2}^{1B_1} u_{\bar{A}_4}^{B_1} u_X^{A_1 g} \\
& + u_{A_3}^{1B_1} u_X^{A_1 g} u_{A_1}^{B_1} + u_{A_3}^{B_1} u_X^{A_1 g} u_{A_1}^{1B_1} + u_{A_5}^{B_1} u_A^{A_1 g} u_{X_2}^{B_1} + u_{A_5}^{1B_1} u_A^{A_1 g} u_{X_2}^{B_1} + u_{X_1}^{A_1 g} u_A^{1B_1} u_{\bar{A}_5}^{B_1} \\
& + u_{X_1}^{A_1 g} u_A^{B_1} u_{\bar{A}_5}^{1B_1} + u_{X_1}^{A_1 g} u_{\bar{A}_4}^{B_1} u_{\bar{A}_2}^{1B_1} + u_{X_1}^{A_1 g} u_{\bar{A}_4}^{1B_1} u_{\bar{A}_2}^{B_1} + u_{A_3}^{B_1} u_{X_2}^{A_1 g} u_{\bar{A}_1}^{1B_1} + u_{A_3}^{1B_1} u_{X_2}^{A_1 g} u_{\bar{A}_1}^{B_1} \\
& + u_{\bar{A}_3}^{1B_1} u_{X_2}^{A_1 g} u_{A_1}^{B_1} + u_{\bar{A}_3}^{B_1} u_{X_2}^{A_1 g} u_{A_1}^{1B_1} + u_{X_1}^{A_1 g} u_{A_2}^{1B_1} u_{A_4}^{B_1} + u_{X_1}^{A_1 g} u_{A_2}^{B_1} u_{A_4}^{1B_1} \\
& + d_{A_3 X_2 \bar{A}_1}^{B_2 E_g B_1} (-u_{X_2}^{E_g(0)} u_{\bar{A}}^{B_2} u_{\bar{A}_5}^{B_1} + u_{X_2$$

[illegible]



[illegible]

$$\begin{aligned}
& -u_X^{B_2u} u_{\bar{A}_2}^{B_1} u_{A_4}^{B_2} + u_{\bar{A}_3}^{B_1} u_{\bar{A}_1}^{B_2} u_X^{A_2u} + u_{\bar{A}_3}^{B_1} u_{\bar{A}_1}^{B_1} u_X^{A_2u} + u_{A_2}^{B_1} u_{\bar{A}_4}^{A_2u} u_X^{B_1} + u_{A_2}^{B_1} u_{\bar{A}_4}^{B_1} u_X^{A_2u} \\
& - u_{A_3}^{B_1} u_X^{A_2u} u_{A_1}^{B_1} - u_{A_3}^{B_1} u_X^{A_2u} u_{A_1}^{B_2} + u_{A_5}^{B_1} u_A^{A_2u} u_{X_2}^{B_1} + u_{A_5}^{B_1} u_A^{B_1} u_{X_2}^{A_2u} - u_{X_1}^{A_2u} u_A^{B_1} u_{\bar{A}_5}^{B_1} \\
& - u_{X_1}^{A_2u} u_A^{B_1} u_{\bar{A}_5}^{B_1} + u_{X_1}^{A_2u} u_{\bar{A}_4}^{B_1} u_{\bar{A}_2}^{B_1} + u_{X_1}^{A_2u} u_{\bar{A}_4}^{B_2} u_{\bar{A}_2}^{B_1} + u_{A_3}^{B_1} u_{X_2}^{A_2u} u_{\bar{A}_1}^{B_1} + u_{A_3}^{B_1} u_{X_2}^{A_2u} u_{\bar{A}_1}^{B_2} \\
& - u_{\bar{A}_3}^{B_1} u_{X_2}^{A_2u} u_{A_1}^{B_1} - u_{\bar{A}_3}^{B_1} u_{X_2}^{A_2u} u_{A_1}^{B_2} - u_{X_1}^{A_2u} u_{A_2}^{B_1} u_{A_4}^{B_1} - u_{X_1}^{A_2u} u_{A_2}^{B_2} u_{A_4}^{B_1} \\
& + d_{A_3 X_2}^{B_2 B_1 u} u_{\bar{A}_1}^{B_1} (u_{X_2}^{B_1u} u_{\bar{A}}^{B_2} u_{\bar{A}_5}^{B_1} + u_{X_2}^{B_1u} u_{\bar{A}}^{B_1} u_{\bar{A}_5}^{B_2} - u_{X_1}^{B_1u} u_{A_5}^{B_1} u_{\bar{A}}^{B_2} - u_{X_1}^{B_1u} u_{A_5}^{B_2} u_{\bar{A}}^{B_1} - u_X^{B_1u} u_{\bar{A}_2}^{B_2} u_{A_4}^{B_1} \\
& - u_X^{B_1u} u_{\bar{A}_2}^{B_1} u_{A_4}^{B_2} + u_{\bar{A}_3}^{B_1} u_{\bar{A}_1}^{B_2} u_X^{B_1u} + u_{\bar{A}_3}^{B_2} u_{\bar{A}_1}^{B_1} u_X^{B_1u} - u_{\bar{A}_3}^{B_1} u_{\bar{A}_4}^{B_2} u_X^{B_1u} - u_{\bar{A}_2}^{B_2} u_{\bar{A}_4}^{B_1} u_X^{B_1u} \\
& + u_{A_3}^{B_2} u_X^{B_1u} u_{A_1}^{B_1} + u_{A_3}^{B_1} u_X^{B_1u} u_{A_1}^{B_2} + u_{A_5}^{B_1} u_A^{B_2} u_{X_2}^{B_1u} + u_{A_5}^{B_2} u_A^{B_1} u_{X_2}^{B_1u} - u_{X_1}^{B_1u} u_A^{B_2} u_{\bar{A}_5}^{B_1} \\
& - u_{X_1}^{B_1u} u_A^{B_1} u_{\bar{A}_5}^{B_2} + u_{X_1}^{B_1u} u_{\bar{A}_4}^{B_1} u_{\bar{A}_2}^{B_2} + u_{X_1}^{B_1u} u_{\bar{A}_4}^{B_2} u_{\bar{A}_2}^{B_1} - u_{A_3}^{B_1} u_{X_2}^{B_1u} u_{\bar{A}_1}^{B_2} - u_{A_3}^{B_2} u_{X_2}^{B_1u} u_{\bar{A}_1}^{B_1} \\
& - u_{\bar{A}_3}^{B_2} u_{X_2}^{B_1u} u_{A_1}^{B_1} - u_{\bar{A}_3}^{B_1} u_{X_2}^{B_1u} u_{A_1}^{B_2} + u_{X_1}^{B_1u} u_{A_2}^{B_2} u_{\bar{A}_4}^{B_1} + u_{X_1}^{B_1u} u_{A_2}^{B_1} u_{\bar{A}_4}^{B_2}) \\
& + d_{A_3 X_2}^{B_2 B_1 u} u_{\bar{A}_1}^{B_1} (u_{X_2}^{B_1u} u_{\bar{A}}^{B_2} u_{\bar{A}_5}^{B_1} + u_{X_2}^{B_1u} u_{\bar{A}}^{B_1} u_{\bar{A}_5}^{B_2} - u_{X_1}^{B_1u} u_{A_5}^{B_1} u_{\bar{A}}^{B_2} - u_{X_1}^{B_1u} u_{A_5}^{B_2} u_{\bar{A}}^{B_1} - u_X^{B_1u} u_{\bar{A}_2}^{B_2} u_{A_4}^{B_1} \\
& - u_X^{B_1u} u_{\bar{A}_2}^{B_1} u_{A_4}^{B_2} + u_{\bar{A}_3}^{B_1} u_{\bar{A}_1}^{B_2} u_X^{B_1u} + u_{\bar{A}_3}^{B_2} u_{\bar{A}_1}^{B_1} u_X^{B_1u} - u_{\bar{A}_2}^{B_1} u_{\bar{A}_4}^{B_2} u_X^{B_1u} - u_{\bar{A}_2}^{B_2} u_{\bar{A}_4}^{B_1} u_X^{B_1u} \\
& + u_{A_3}^{B_2} u_X^{B_1u} u_{A_1}^{B_1} + u_{A_3}^{B_1} u_X^{B_1u} u_{A_1}^{B_2} + u_{A_5}^{B_1} u_A^{B_2} u_{X_2}^{B_1u} + u_{A_5}^{B_2} u_A^{B_1} u_{X_2}^{B_1u} - u_{X_1}^{B_1u} u_A^{B_2} u_{\bar{A}_5}^{B_1} \\
& - u_{X_1}^{B_1u} u_A^{B_1} u_{\bar{A}_5}^{B_2} + u_{X_1}^{B_1u} u_{\bar{A}_4}^{B_1} u_{\bar{A}_2}^{B_2} + u_{X_1}^{B_1u} u_{\bar{A}_4}^{B_2} u_{\bar{A}_2}^{B_1} - u_{A_3}^{B_1} u_{X_2}^{B_1u} u_{\bar{A}_1}^{B_2} - u_{A_3}^{B_2} u_{X_2}^{B_1u} u_{\bar{A}_1}^{B_1} \\
& - u_{\bar{A}_3}^{B_2} u_{X_2}^{B_1u} u_{A_1}^{B_1} - u_{\bar{A}_3}^{B_1} u_{X_2}^{B_1u} u_{A_1}^{B_2} + u_{X_1}^{B_1u} u_{A_2}^{B_2} u_{\bar{A}_4}^{B_1} + u_{X_1}^{B_1u} u_{A_2}^{B_1} u_{\bar{A}_4}^{B_2}) \\
& + d_{A_3 X_2}^{B_1 E_u} u_{\bar{A}_1}^{B_1} (u_{X_2}^{E_u(0)} u_{\bar{A}}^{B_2} u_{\bar{A}_5}^{B_1} - u_{X_2}^{E_u(0)} u_{\bar{A}}^{B_1} u_{\bar{A}_5}^{B_2} - u_{X_1}^{E_u(0)} u_{A_5}^{B_1} u_{\bar{A}}^{B_2} + u_{X_1}^{E_u(0)} u_{A_5}^{B_2} u_{\bar{A}}^{B_1} + u_X^{E_u(0)} u_{\bar{A}_2}^{B_2} u_{A_4}^{B_1} \\
& - u_X^{E_u(0)} u_{\bar{A}_2}^{B_1} u_{A_4}^{B_2} + u_{\bar{A}_3}^{B_1} u_{\bar{A}_1}^{B_2} u_X^{E_u(1)} - u_{\bar{A}_3}^{B_2} u_{\bar{A}_1}^{B_1} u_X^{E_u(1)} + u_{A_2}^{B_1} u_{\bar{A}_4}^{B_2} u_X^{E_u(0)} - u_{A_2}^{B_2} u_{\bar{A}_4}^{B_1} u_X^{E_u(0)} \\
& + u_{A_3}^{B_2} u_X^{E_u(1)} u_{A_1}^{B_1} - u_{A_3}^{B_1} u_X^{E_u(1)} u_{A_1}^{B_2} - u_{A_5}^{B_1} u_A^{B_2} u_{X_2}^{E_u(0)} + u_{A_5}^{B_2} u_A^{B_1} u_{X_2}^{E_u(0)} + u_{X_1}^{E_u(0)} u_A^{B_2} u_{\bar{A}_5}^{B_1} \\
& - u_{X_1}^{E_u(0)} u_A^{B_1} u_{\bar{A}_5}^{B_2} - u_{X_1}^{E_u(1)} u_{\bar{A}_4}^{B_1} u_{\bar{A}_2}^{B_2} + u_{X_1}^{E_u(1)} u_{\bar{A}_4}^{B_2} u_{\bar{A}_2}^{B_1} + u_{A_3}^{B_1} u_{X_2}^{E_u(1)} u_{\bar{A}_1}^{B_2} - u_{A_3}^{B_2} u_{X_2}^{E_u(1)} u_{\bar{A}_1}^{B_1} \\
& + u_{\bar{A}_3}^{B_2} u_{X_2}^{E_u(1)} u_{A_1}^{B_1} - u_{\bar{A}_3}^{B_1} u_{X_2}^{E_u(1)} u_{A_1}^{B_2} + u_{X_1}^{E_u(1)} u_{A_2}^{B_2} u_{\bar{A}_4}^{B_1} - u_{X_1}^{E_u(1)} u_{A_2}^{B_1} u_{\bar{A}_4}^{B_2}) \\
& + d_{A_3 X_2}^{B_2 E_u} u_{\bar{A}_1}^{B_1} (u_{X_2}^{E_u(1)} u_{\bar{A}}^{B_2} u_{\bar{A}_5}^{B_1} - u_{X_2}^{E_u(1)} u_{\bar{A}}^{B_1} u_{\bar{A}_5}^{B_2} - u_{X_1}^{E_u(1)} u_{A_5}^{B_1} u_{\bar{A}}^{B_2} + u_{X_1}^{E_u(1)} u_{A_5}^{B_2} u_{\bar{A}}^{B_1} - u_X^{E_u(1)} u_{\bar{A}_2}^{B_2} u_{A_4}^{B_1} \\
& + u_X^{E_u(1)} u_{\bar{A}_2}^{B_1} u_{A_4}^{B_2} - u_{\bar{A}_3}^{B_1} u_{\bar{A}_1}^{B_2} u_X^{E_u(0)} + u_{\bar{A}_3}^{B_2} u_{\bar{A}_1}^{B_1} u_X^{E_u(0)} + u_{A_2}^{B_1} u_{\bar{A}_4}^{B_2} u_X^{E_u(1)} - u_{A_2}^{B_2} u_{\bar{A}_4}^{B_1} u_X^{E_u(1)} \\
& + u_{A_3}^{B_2} u_X^{E_u(0)} u_{A_1}^{B_1} - u_{A_3}^{B_1} u_X^{E_u(0)} u_{A_1}^{B_2} + u_{A_5}^{B_1} u_A^{B_2} u_{X_2}^{E_u(1)} - u_{A_5}^{B_2} u_A^{B_1} u_{X_2}^{E_u(1)} - u_{X_1}^{E_u(1)} u_A^{B_2} u_{\bar{A}_5}^{B_1} \\
& + u_{X_1}^{E_u(1)} u_A^{B_1} u_{\bar{A}_5}^{B_2} + u_{X_1}^{E_u(0)} u_{\bar{A}_4}^{B_1} u_{\bar{A}_2}^{B_2} - u$$



[illegible]

[illegible]

$$\begin{aligned}
& + u_{A_3}^{1B_2} u_{X_2}^{E_g^{(0)}} u_{A_1}^{B_2} - u_{A_3}^{B_2} u_{X_2}^{E_g^{(0)}} u_{A_1}^{1B_2} - u_{X_1}^{E_g^{(0)}} u_{A_2}^{1B_2} u_{A_4}^{B_2} + u_{X_1}^{E_g^{(0)}} u_{A_2}^{B_2} u_{A_4}^{1B_2} \\
& + d_{A_3 X_2}^{B_2 A_2 u} \left( -u_{X_2}^{A_2 u} u_{A_5}^{B_2} u_{A_1}^{B_2} + u_{X_1}^{A_2 u} u_{A_5}^{B_2} u_{A_1}^{B_2} - u_{X_1}^{A_2 u} u_{A_5}^{B_2} u_{A_1}^{B_2} + u_{A_3}^{B_2} u_{A_1}^{B_2} u_{X_2}^{A_2 u} + u_{A_2}^{B_2} u_{A_4}^{B_2} u_{X_2}^{A_2 u} \right. \\
& \quad - u_{A_3}^{B_2} u_{X_2}^{A_2 u} u_{A_1}^{B_2} + u_{A_5}^{B_2} u_{A_1}^{B_2} u_{X_2}^{A_2 u} - u_{X_1}^{A_2 u} u_{A_5}^{B_2} u_{A_1}^{B_2} + u_{X_1}^{A_2 u} u_{A_4}^{B_2} u_{A_2}^{B_2} + u_{A_3}^{B_2} u_{X_2}^{A_2 u} u_{A_1}^{B_2} \\
& \quad \left. - u_{A_3}^{B_2} u_{X_2}^{A_2 u} u_{A_1}^{B_2} - u_{X_1}^{A_2 u} u_{A_2}^{B_2} u_{A_4}^{B_2} \right) \\
& + d_{A_3 X_2}^{B_2 A_2 u} \left( -u_{X_2}^{A_2 u} u_{A_5}^{1B_2} u_{A_1}^{B_2} - u_{X_2}^{A_2 u} u_{A_5}^{1B_2} u_{A_1}^{B_2} + u_{X_1}^{A_2 u} u_{A_5}^{B_2} u_{A_1}^{1B_2} + u_{X_1}^{A_2 u} u_{A_5}^{B_2} u_{A_1}^{1B_2} - u_{X_1}^{A_2 u} u_{A_5}^{1B_2} u_{A_1}^{B_2} \right. \\
& \quad - u_{X_1}^{A_2 u} u_{A_2}^{B_2} u_{A_4}^{1B_2} + u_{A_3}^{B_2} u_{A_1}^{1B_2} u_{X_2}^{A_2 u} + u_{A_3}^{B_2} u_{A_1}^{1B_2} u_{X_2}^{A_2 u} + u_{A_2}^{B_2} u_{A_4}^{1B_2} u_{X_2}^{A_2 u} + u_{A_2}^{B_2} u_{A_4}^{1B_2} u_{X_2}^{A_2 u} \\
& \quad - u_{A_3}^{1B_2} u_{X_2}^{A_2 u} u_{A_1}^{B_2} - u_{A_3}^{B_2} u_{X_2}^{A_2 u} u_{A_1}^{1B_2} + u_{A_5}^{B_2} u_{A_1}^{1B_2} u_{X_2}^{A_2 u} + u_{A_5}^{1B_2} u_{A_1}^{B_2} u_{X_2}^{A_2 u} - u_{X_1}^{A_2 u} u_{A_1}^{1B_2} u_{A_5}^{B_2} \\
& \quad - u_{X_1}^{A_2 u} u_{A_2}^{B_2} u_{A_4}^{1B_2} + u_{X_1}^{A_2 u} u_{A_4}^{B_2} u_{A_2}^{1B_2} + u_{A_3}^{B_2} u_{X_2}^{A_2 u} u_{A_1}^{1B_2} + u_{A_3}^{1B_2} u_{X_2}^{A_2 u} u_{A_1}^{B_2} \\
& \quad \left. - u_{A_3}^{1B_2} u_{X_2}^{A_2 u} u_{A_1}^{B_2} - u_{A_3}^{B_2} u_{X_2}^{A_2 u} u_{A_1}^{1B_2} - u_{X_1}^{A_2 u} u_{A_2}^{B_2} u_{A_4}^{1B_2} - u_{X_1}^{A_2 u} u_{A_2}^{B_2} u_{A_4}^{1B_2} \right) \\
& + d_{A_3 X_2 A_1}^{B_2 E_u} \left( u_{X_2}^{E_u^{(0)}} u_{A_1}^{1B_2} u_{A_5}^{B_2} - u_{X_2}^{E_u^{(0)}} u_{A_1}^{B_2} u_{A_5}^{1B_2} - u_{X_1}^{E_u^{(0)}} u_{A_5}^{B_2} u_{A_1}^{1B_2} + u_{X_1}^{E_u^{(0)}} u_{A_5}^{B_2} u_{A_1}^{1B_2} + u_{X_1}^{E_u^{(0)}} u_{A_5}^{1B_2} u_{A_1}^{B_2} \right. \\
& \quad - u_{X_1}^{E_u^{(0)}} u_{A_2}^{B_2} u_{A_4}^{1B_2} + u_{A_3}^{B_2} u_{A_1}^{1B_2} u_{X_2}^{E_u^{(1)}} - u_{A_3}^{B_2} u_{A_1}^{1B_2} u_{X_2}^{E_u^{(1)}} + u_{A_2}^{B_2} u_{A_4}^{1B_2} u_{X_2}^{E_u^{(0)}} - u_{A_2}^{B_2} u_{A_4}^{1B_2} u_{X_2}^{E_u^{(0)}} \\
& \quad + u_{A_3}^{1B_2} u_{X_2}^{E_u^{(1)}} u_{A_1}^{B_2} - u_{A_3}^{B_2} u_{X_2}^{E_u^{(1)}} u_{A_1}^{1B_2} - u_{A_5}^{B_2} u_{A_1}^{1B_2} u_{X_2}^{E_u^{(0)}} + u_{A_5}^{1B_2} u_{A_1}^{B_2} u_{X_2}^{E_u^{(0)}} + u_{X_1}^{E_u^{(0)}} u_{A_1}^{1B_2} u_{A_5}^{B_2} \\
& \quad - u_{X_1}^{E_u^{(0)}} u_{A_2}^{B_2} u_{A_4}^{1B_2} - u_{X_1}^{E_u^{(1)}} u_{A_4}^{B_2} u_{A_2}^{1B_2} + u_{X_1}^{E_u^{(1)}} u_{A_4}^{B_2} u_{A_2}^{1B_2} + u_{A_3}^{B_2} u_{X_2}^{E_u^{(1)}} u_{A_1}^{1B_2} - u_{A_3}^{1B_2} u_{X_2}^{E_u^{(1)}} u_{A_1}^{B_2} \\
& \quad + u_{A_3}^{1B_2} u_{X_2}^{E_u^{(1)}} u_{A_1}^{B_2} - u_{A_3}^{B_2} u_{X_2}^{E_u^{(1)}} u_{A_1}^{1B_2} + u_{X_1}^{E_u^{(1)}} u_{A_2}^{B_2} u_{A_4}^{1B_2} - u_{X_1}^{E_u^{(1)}} u_{A_2}^{B_2} u_{A_4}^{1B_2} \left. \right) \\
& + d_{A_3 X_2 A_1}^{B_2 E_u} \left( u_{X_2}^{1E_u^{(0)}} u_{A_1}^{B_2} u_{A_5}^{B_2} - u_{X_2}^{1E_u^{(0)}} u_{A_1}^{B_2} u_{A_5}^{B_2} - u_{X_1}^{1E_u^{(0)}} u_{A_5}^{B_2} u_{A_1}^{B_2} + u_{X_1}^{1E_u^{(0)}} u_{A_5}^{B_2} u_{A_1}^{B_2} + u_{X_1}^{1E_u^{(0)}} u_{A_5}^{B_2} u_{A_1}^{B_2} \right. \\
& \quad - u_{X_1}^{1E_u^{(0)}} u_{A_2}^{B_2} u_{A_4}^{1B_2} + u_{A_3}^{B_2} u_{A_1}^{1B_2} u_{X_2}^{1E_u^{(1)}} - u_{A_3}^{B_2} u_{A_1}^{1B_2} u_{X_2}^{1E_u^{(1)}} + u_{A_2}^{B_2} u_{A_4}^{1B_2} u_{X_2}^{1E_u^{(0)}} - u_{A_2}^{B_2} u_{A_4}^{1B_2} u_{X_2}^{1E_u^{(0)}} \\
& \quad + u_{A_3}^{1B_2} u_{X_2}^{1E_u^{(1)}} u_{A_1}^{B_2} - u_{A_3}^{B_2} u_{X_2}^{1E_u^{(1)}} u_{A_1}^{1B_2} - u_{A_5}^{B_2} u_{A_1}^{1B_2} u_{X_2}^{1E_u^{(0)}} + u_{A_5}^{1B_2} u_{A_1}^{B_2} u_{X_2}^{1E_u^{(0)}} + u_{X_1}^{1E_u^{(0)}} u_{A_1}^{1B_2} u_{A_5}^{B_2} \\
& \quad - u_{X_1}^{1E_u^{(0)}} u_{A_2}^{B_2} u_{A_4}^{1B_2} - u_{X_1}^{1E_u^{(1)}} u_{A_4}^{B_2} u_{A_2}^{1B_2} + u_{X_1}^{1E_u^{(1)}} u_{A_4}^{B_2} u_{A_2}^{1B_2} + u_{A_3}^{B_2} u_{X_2}^{1E_u^{(1)}} u_{A_1}^{1B_2} - u_{A_3}^{1B_2} u_{X_2}^{1E_u^{(1)}} u_{A_1}^{B_2} \\
& \quad + u_{A_3}^{1B_2} u_{X_2}^{1E_u^{(1)}} u_{A_1}^{B_2} - u_{A_3}^{B_2} u_{X_2}^{1E_u^{(1)}} u_{A_1}^{1B_2} + u_{X_1}^{1E_u^{(1)}} u_{A_2}^{B_2} u_{A_4}^{1B_2} - u_{X_1}^{1E_u^{(1)}} u_{A_2}^{B_2} u_{A_4}^{1B_2} \left. \right) \\
& + d_{A_3 X_2 A_1}^{1B_2 A_1 g} \left( u_{X_2}^{1B_2} u_{A_1}^{1B_2} u_{A_5}^{B_2} + u_{X_1}^{1B_2} u_{A_5}^{B_2} u_{A_1}^{1B_2} + u_{X_1}^{1B_2} u_{A_2}^{B_2} u_{A_4}^{1B_2} + u_{A_3}^{B_2} u_{A_1}^{1B_2} u_{X_2}^{1B_2} + u_{A_2}^{B_2} u_{A_4}^{1B_2} u_{X_2}^{1B_2} \right. \\
& \quad + u_{A_3}^{1B_2} u_{X_2}^{1B_2} u_{A_1}^{B_2} + u_{A_5}^{1B_2} u_{A_1}^{B_2} u_{X_2}^{1B_2} + u_{X_1}^{1B_2} u_{A_1}^{B_2} u_{A_5}^{1B_2} + u_{X_1}^{1B_2} u_{A_4}^{B_2} u_{A_2}^{1B_2} + u_{A_3}^{1B_2} u_{X_2}^{1B_2} u_{A_1}^{B_2} \\
& \quad + u_{A_3}^{1B_2} u_{X_2}^{1B_2} u_{A_1}^{B_2} + u_{X_1}^{1B_2} u_{A_2}^{B_2} u_{A_4}^{1B_2} \left. \right) \\
& + d_{A_3 X_2 A_1}^{1B_2 A_2 u} \left( -u_{X_2}^{A_2 u} u_{A_5}^{1B_2} u_{A_1}^{B_2} + u_{X_1}^{A_2 u} u_{A_5}^{1B_2} u_{A_1}^{B_2} - u_{X_1}^{A_2 u} u_{A_5}^{1B_2} u_{A_1}^{B_2} + u_{A_3}^{B_2} u_{A_1}^{1B_2} u_{X_2}^{A_2 u} + u_{A_2}^{B_2} u_{A_4}^{1B_2} u_{X_2}^{A_2 u} \right. \\
& \quad - u_{A_3}^{1B_2} u_{X_2}^{A_2 u} u_{A_1}^{B_2} + u_{A_5}^{1B_2} u_{A_1}^{B_2} u_{X_2}^{A_2 u} - u_{X_1}^{A_2 u} u_{A_5}^{1B_2} u_{A_1}^{B_2} + u_{X_1}^{A_2 u} u_{A_4}^{B_2} u_{A_2}^{1B_2} + u_{A_3}^{B_2} u_{X_2}^{A_2 u} u_{A_1}^{1B_2} \\
& \quad \left. - u_{A_3}^{1B_2} u_{X_2}^{A_2 u} u_{A_1}^{B_2} - u_{X_1}^{A_2 u} u_{A_2}^{B_2} u_{A_4}^{1B_2} \right) \\
& + d_{X_1 X_2 X}^{A_1 g A_1 g} \left( u_{X_1}^{A_1 g} u_{X_2}^{A_1 g} u_X^{A_1 g} \right) \\
& + d_{X_1 X_2 X}^{A_1 g E_g} \left( u_{X_1}^{A_1 g} u_{X_2}^{E_g^{(0)}} u_X^{E_g^{(1)}} + u_{X_1}^{E_g^{(0)}} u_{X_2}^{A_1 g} u_X^{E_g^{(1)}} + u_{X_1}^{E_g^{(1)}} u_{X_2}^{E_g^{(1)}} u_X^{A_1 g} \right) \\
& + d_{X_1 X_2 X}^{A_1 g A_2 u} \left( u_{X_1}^{A_1 g} u_{X_2}^{A_2 u} u_X^{E_u^{(1)}} + u_{X_1}^{A_1 g} u_{X_2}^{E_u^{(1)}} u_X^{A_2 u} + u_{X_1}^{A_2 u} u_{X_2}^{A_1 g} u_X^{E_u^{(0)}} + u_{X_1}^{A_2 u} u_{X_2}^{E_u^{(0)}} u_X^{A_1 g} + u_{X_1}^{E_u^{(0)}} u_{X_2}^{A_2 u} u_X^{A_1 g} \right. \\
& \quad \left. + u_{X_1}^{E_u^{(1)}} u_{X_2}^{A_1 g} u_X^{A_2 u} \right) \\
& + d_{X_1 X_2 X}^{A_1 g A_2 u} \left( u_{X_1}^{A_1 g} u_{X_2}^{A_2 u} u_X^{1E_u^{(1)}} + u_{X_1}^{A_1 g} u_{X_2}^{1E_u^{(1)}} u_X^{A_2 u} + u_{X_1}^{A_2 u} u_{X_2}^{A_1 g} u_X^{1E_u^{(0)}} + u_{X_1}^{A_2 u} u_{X_2}^{1E_u^{(0)}} u_X^{A_1 g} + u_{X_1}^{1E_u^{(0)}} u_{X_2}^{A_2 u} u_X^{A_1 g} \right. \\
& \quad \left. + u_{X_1}^{1E_u^{(1)}} u_{X_2}^{A_1 g} u_X^{A_2 u} \right) \\
& + d_{X_1 X_2 X}^{A_1 g B_{1u} B_{1u}} \left( u_{X_1}^{A_1 g} u_{X_2}^{B_{1u}} u_X^{B_{1u}} + u_{X_1}^{B_{1u}} u_{X_2}^{A_1 g} u_X^{B_{1u}} + u_{X_1}^{B_{1u}} u_{X_2}^{B_{1u}} u_X^{A_1 g} \right) \\
& + d_{X_1 X_2 X}^{A_1 g E_u} \left( u_{X_1}^{A_1 g} u_{X_2}^{E_u^{(0)}} u_X^{E_u^{(1)}} + u_{X_1}^{E_u^{(0)}} u_{X_2}^{A_1 g} u_X^{E_u^{(1)}} + u_{X_1}^{E_u^{(1)}} u_{X_2}^{E_u^{(1)}} u_X^{A_1 g} \right) \\
& + d_{X_1 X_2 X}^{A_1 g E_u} \left( u_{X_1}^{A_1 g} u_{X_2}^{1E_u^{(0)}} u_X^{1E_u^{(0)}} + u_{X_1}^{A_1 g} u_{X_2}^{1E_u^{(0)}} u_X^{E_u^{(0)}} + u_{X_1}^{E_u^{(0)}} u_{X_2}^{A_1 g} u_X^{1E_u^{(1)}} + u_{X_1}^{E_u^{(1)}} u_{X_2}^{1E_u^{(1)}} u_X^{A_1 g} + u_{X_1}^{1E_u^{(0)}} u_{X_2}^{A_1 g} u_X^{E_u^{(1)}} \right. \\
& \quad \left. + u_{X_1}^{1E_u^{(1)}} u_{X_2}^{E_u^{(1)}} u_X^{A_1 g} \right)
\end{aligned}$$

$$\begin{aligned}
& +d_{X_1 X_2 X}^{A_{1g} {}^1E_u {}^1E_u} (u_{X_1}^{A_{1g} {}^1E_u^{(0)} {}^1E_u^{(0)}} + u_{X_1}^{1E_u^{(0)} A_{1g} {}^1E_u^{(1)}} + u_{X_1}^{1E_u^{(1)} {}^1E_u^{(1)} A_{1g}}) \\
& +d_{X_1 X_2 X}^{E_g E_g E_g} (u_{X_1}^{E_g^{(0)} E_g^{(1)} E_g^{(0)}} - u_{X_1}^{E_g^{(1)} E_g^{(0)} E_g^{(1)}}) \\
& +d_{X_1 X_2 X}^{B_{1u} A_{2u} E_g} (u_{X_1}^{E_g^{(0)} A_{2u} B_{1u}} - u_{X_1}^{E_g^{(1)} B_{1u} A_{2u}} - u_{X_1}^{A_{2u} E_g^{(0)} B_{1u}} + u_{X_1}^{A_{2u} B_{1u} E_g^{(0)}} + u_{X_1}^{B_{1u} E_g^{(1)} A_{2u}} \\
& \quad - u_{X_1}^{B_{1u} A_{2u} E_g^{(1)}}) \\
& +d_{X_1 X_2 X}^{B_{1u} E_g E_u} (-u_{X_1}^{E_g^{(0)} B_{1u} E_u^{(1)}} + u_{X_1}^{E_g^{(1)} E_u^{(1)} B_{1u}} + u_{X_1}^{B_{1u} E_g^{(0)} E_u^{(0)}} - u_{X_1}^{B_{1u} E_u^{(0)} E_g^{(0)}} + u_{X_1}^{E_u^{(0)} B_{1u} E_g^{(1)}} \\
& \quad - u_{X_1}^{E_u^{(1)} E_g^{(1)} B_{1u}}) \\
& +d_{X_1 X_2 X}^{B_{1u} E_g {}^1E_u} (-u_{X_1}^{E_g^{(0)} B_{1u} {}^1E_u^{(1)}} + u_{X_1}^{E_g^{(1)} {}^1E_u^{(1)} B_{1u}} + u_{X_1}^{B_{1u} E_g^{(0)} {}^1E_u^{(0)}} - u_{X_1}^{B_{1u} {}^1E_u^{(0)} E_g^{(0)}} + u_{X_1}^{1E_u^{(0)} B_{1u} E_g^{(1)}} \\
& \quad - u_{X_1}^{1E_u^{(1)} E_g^{(1)} B_{1u}}) \\
& +d_{X_1 X_2 X}^{A_{2u} E_g E_u} (u_{X_1}^{E_g^{(0)} E_u^{(0)} A_{2u}} - u_{X_1}^{E_g^{(1)} A_{2u} E_u^{(0)}} + u_{X_1}^{A_{2u} E_g^{(1)} E_u^{(1)}} - u_{X_1}^{A_{2u} E_u^{(1)} E_g^{(1)}} - u_{X_1}^{E_u^{(0)} E_g^{(0)} A_{2u}} \\
& \quad + u_{X_1}^{E_u^{(1)} A_{2u} E_g^{(0)}}) \\
& +d_{X_1 X_2 X}^{E_g E_u E_u} (u_{X_1}^{E_g^{(0)} E_u^{(1)} E_u^{(0)}} - u_{X_1}^{E_g^{(1)} E_u^{(0)} E_u^{(1)}} + u_{X_1}^{E_u^{(0)} E_g^{(1)} E_u^{(0)}} + u_{X_1}^{E_u^{(0)} E_u^{(1)} E_g^{(0)}} - u_{X_1}^{E_u^{(1)} E_g^{(0)} E_u^{(1)}} \\
& \quad - u_{X_1}^{E_u^{(1)} E_u^{(0)} E_g^{(1)}}) \\
& +{}^0d_{X_1 X_2 X}^{E_g E_u {}^1E_u} (u_{X_1}^{E_g^{(0)} E_u^{(1)} {}^1E_u^{(0)}} - u_{X_1}^{E_g^{(1)} {}^1E_u^{(0)} E_u^{(1)}} + u_{X_1}^{E_u^{(0)} {}^1E_u^{(1)} E_g^{(0)}} - u_{X_1}^{E_u^{(1)} E_g^{(0)} {}^1E_u^{(1)}} + u_{X_1}^{1E_u^{(0)} E_g^{(1)} E_u^{(0)}} \\
& \quad - u_{X_1}^{1E_u^{(1)} E_u^{(0)} E_g^{(1)}}) \\
& +d_{X_1 X_2 X}^{A_{2u} E_g {}^1E_u} (u_{X_1}^{E_g^{(0)} {}^1E_u^{(0)} A_{2u}} - u_{X_1}^{E_g^{(1)} A_{2u} {}^1E_u^{(0)}} + u_{X_1}^{A_{2u} E_g^{(1)} {}^1E_u^{(1)}} - u_{X_1}^{A_{2u} {}^1E_u^{(1)} E_g^{(1)}} - u_{X_1}^{1E_u^{(0)} E_g^{(0)} A_{2u}} \\
& \quad + u_{X_1}^{1E_u^{(1)} A_{2u} E_g^{(0)}}) \\
& +{}^1d_{X_1 X_2 X}^{E_g E_u {}^1E_u} (u_{X_1}^{E_g^{(0)} {}^1E_u^{(1)} E_u^{(0)}} - u_{X_1}^{E_g^{(1)} E_u^{(0)} {}^1E_u^{(1)}} + u_{X_1}^{E_u^{(0)} E_g^{(1)} {}^1E_u^{(0)}} - u_{X_1}^{E_u^{(1)} {}^1E_u^{(0)} E_g^{(1)}} + u_{X_1}^{1E_u^{(0)} E_u^{(1)} E_g^{(0)}} \\
& \quad - u_{X_1}^{1E_u^{(1)} E_g^{(0)} E_u^{(1)}}) \\
& +d_{X_1 X_2 X}^{E_g {}^1E_u {}^1E_u} (u_{X_1}^{E_g^{(0)} {}^1E_u^{(1)} {}^1E_u^{(0)}} - u_{X_1}^{E_g^{(1)} {}^1E_u^{(0)} {}^1E_u^{(1)}} + u_{X_1}^{1E_u^{(0)} E_g^{(1)} {}^1E_u^{(0)}} + u_{X_1}^{1E_u^{(0)} {}^1E_u^{(1)} E_g^{(0)}} - u_{X_1}^{1E_u^{(1)} E_g^{(0)} {}^1E_u^{(1)}} \\
& \quad - u_{X_1}^{1E_u^{(1)} {}^1E_u^{(0)} E_g^{(1)}})
\end{aligned}$$
